# Supplementary material for: On Measuring Unnoticeability of Graph Adversarial Attacks: Observations, New Measure, and Applications
Source: arXiv:2501.05015 source file (2025-01-09)
Supplement: Supplementary file 1 [file 05_abl_appendix.tex]

\begin{table*}[h]
\caption{\label{tab:exp:abl}
\underline{\smash{Ablation study}}: 
\model ranks first in all attack methods w.r.t average rank (AR) compared with its variants. O.O.T: out of time ($>$ 3 hours). O.O.M: out of (GPU) memory. N.A: not available (specifically, the maximum number of attacks allowed by \structack is exceeded). For each setting (each column), the best and second-best results are in \setlength{\fboxsep}{1pt}\colorbox{Red!40}{red} and \setlength{\fboxsep}{1pt}\colorbox{Blue!40}{blue}, respectively.
}
%\vspace{0.8cm}
\centering
\resizebox{!}{0.42\textwidth}{
    \begin{tabular}{c||ccc||c|c|c|c|c|c||c}
    \hline
    & \multicolumn{3}{c||}{\textbf{Modules}} & \multicolumn{6}{c||}{\textbf{Datasets}} & \multirow{2}{*}{\textbf{AR}} \\
    \cline{2-10}
    & $M_{G}$ & $M_{S}$ & $M_{P}$ & \cora & \citeseer & \coraml & \lastfmasia & \chameleon & \squirrel & \\
    \hline
    \hline
    \multirow{7}{*}{\rotatebox[origin=c]{90}{\random}}
    & \cmark & \xmark  & \xmark & 0.790$\pm$0.006 & 0.720$\pm$0.123 & 0.826$\pm$0.019 & 0.911$\pm$0.003 & 0.939$\pm$0.009 & 0.941$\pm$0.002 & 5.3 \\
    & \xmark & \cmark  & \xmark & 0.846$\pm$0.011 & 0.860$\pm$0.004 & 0.827$\pm$0.020 & 0.894$\pm$0.003 & 0.840$\pm$0.018 & 0.819$\pm$0.012 & 5.2 \\
    & \xmark & \xmark  & \cmark & 0.802$\pm$0.007 & 0.893$\pm$0.006 & 0.795$\pm$0.005 & 0.835$\pm$0.002 & 0.937$\pm$0.002 & 0.953$\pm$0.001 & 5.5 \\
    & \cmark & \cmark  & \xmark & 0.837$\pm$0.009 & 0.852$\pm$0.003 & 0.814$\pm$0.027 & 0.926$\pm$0.001 & 0.894$\pm$0.067 & 0.799$\pm$0.143 & 5.5 \\
    & \cmark & \xmark  & \cmark & 0.849$\pm$0.006 & 0.910$\pm$0.005 & {\setlength{\fboxsep}{1pt}\colorbox{Blue!40}{0.895$\pm$0.004}} & {\setlength{\fboxsep}{1pt}\colorbox{Blue!40}{0.928$\pm$0.002}} & {\setlength{\fboxsep}{1pt}\colorbox{Red!40}{0.974$\pm$0.001}} & {\setlength{\fboxsep}{1pt}\colorbox{Red!40}{0.976$\pm$0.001}} & {\setlength{\fboxsep}{1pt}\colorbox{Blue!40}{2.0}} \\
    & \xmark & \cmark  & \cmark & {\setlength{\fboxsep}{1pt}\colorbox{Blue!40}{0.857$\pm$0.007}} & {\setlength{\fboxsep}{1pt}\colorbox{Red!40}{0.930$\pm$0.003}} & 0.877$\pm$0.008 & 0.883$\pm$0.003 & {\setlength{\fboxsep}{1pt}\colorbox{Red!40}{0.974$\pm$0.002}} & {\setlength{\fboxsep}{1pt}\colorbox{Red!40}{0.976$\pm$0.001}} & 2.3 \\
    \cline{2-11}
    & \cmark & \cmark  & \cmark & {\setlength{\fboxsep}{1pt}\colorbox{Red!40}{0.894$\pm$0.011}} & {\setlength{\fboxsep}{1pt}\colorbox{Blue!40}{0.926$\pm$0.006}} & {\setlength{\fboxsep}{1pt}\colorbox{Red!40}{0.914$\pm$0.004}} & {\setlength{\fboxsep}{1pt}\colorbox{Red!40}{0.931$\pm$0.000}} & 0.973$\pm$0.003 & {\setlength{\fboxsep}{1pt}\colorbox{Red!40}{0.976$\pm$0.001}} & {\setlength{\fboxsep}{1pt}\colorbox{Red!40}{\textbf{1.5}}} \\
    \hline
    \hline
    \multirow{7}{*}{\rotatebox[origin=c]{90}{\dice}}
    & \cmark & \xmark  & \xmark & 0.779$\pm$0.021 & 0.675$\pm$0.163 & 0.835$\pm$0.019 & 0.917$\pm$0.005 & 0.944$\pm$0.009 & 0.938$\pm$0.002 & 5.2 \\
    & \xmark & \cmark  & \xmark & 0.856$\pm$0.017 & 0.881$\pm$0.010 & 0.836$\pm$0.023 & 0.912$\pm$0.005 & 0.855$\pm$0.012 & 0.818$\pm$0.021 & 4.8 \\
    & \xmark & \xmark  & \cmark & 0.809$\pm$0.011 & 0.896$\pm$0.009 & 0.805$\pm$0.008 & 0.842$\pm$0.005 & 0.910$\pm$0.005 & 0.940$\pm$0.001 & 5.3 \\
    & \cmark & \cmark  & \xmark & 0.854$\pm$0.008 & 0.872$\pm$0.012 & 0.826$\pm$0.021 & 0.936$\pm$0.003 & 0.786$\pm$0.150 & 0.784$\pm$0.137 & 5.7 \\
    & \cmark & \xmark  & \cmark & 0.855$\pm$0.009 & 0.914$\pm$0.012 & {\setlength{\fboxsep}{1pt}\colorbox{Blue!40}{0.904$\pm$0.005}} & {\setlength{\fboxsep}{1pt}\colorbox{Blue!40}{0.937$\pm$0.003}} & {\setlength{\fboxsep}{1pt}\colorbox{Blue!40}{0.955$\pm$0.009}} & {\setlength{\fboxsep}{1pt}\colorbox{Blue!40}{0.941$\pm$0.010}} & {\setlength{\fboxsep}{1pt}\colorbox{Blue!40}{2.5}} \\
    & \xmark & \cmark  & \cmark & {\setlength{\fboxsep}{1pt}\colorbox{Blue!40}{0.885$\pm$0.017}} & {\setlength{\fboxsep}{1pt}\colorbox{Blue!40}{0.940$\pm$0.010}} & 0.899$\pm$0.006 & 0.897$\pm$0.003 & 0.949$\pm$0.004 & {\setlength{\fboxsep}{1pt}\colorbox{Red!40}{0.944$\pm$0.004}} & 2.8 \\
    \cline{2-11}
    & \cmark & \cmark  & \cmark & {\setlength{\fboxsep}{1pt}\colorbox{Red!40}{0.899$\pm$0.011}} & {\setlength{\fboxsep}{1pt}\colorbox{Red!40}{0.942$\pm$0.008}} & {\setlength{\fboxsep}{1pt}\colorbox{Red!40}{0.932$\pm$0.003}} & {\setlength{\fboxsep}{1pt}\colorbox{Red!40}{0.941$\pm$0.003}} & {\setlength{\fboxsep}{1pt}\colorbox{Red!40}{0.960$\pm$0.003}} & 0.938$\pm$0.003 & {\setlength{\fboxsep}{1pt}\colorbox{Red!40}{\textbf{1.5}}} \\
    \hline
    \hline
    \multirow{7}{*}{\rotatebox[origin=c]{90}{\pgd}}
    & \cmark & \xmark  & \xmark & 0.644$\pm$0.012 & 0.754$\pm$0.016 & 0.762$\pm$0.020 & 0.560$\pm$0.033 & {\setlength{\fboxsep}{1pt}\colorbox{Blue!40}{0.899$\pm$0.017}} & 0.900$\pm$0.003 & 5.8 \\
    & \xmark & \cmark  & \xmark & 0.749$\pm$0.026 & 0.855$\pm$0.008 & 0.835$\pm$0.033 & 0.736$\pm$0.011 & 0.868$\pm$0.007 & 0.839$\pm$0.023 & 5.5 \\
    & \xmark & \xmark  & \cmark & 0.809$\pm$0.005 & 0.882$\pm$0.006 & 0.812$\pm$0.008 & {\setlength{\fboxsep}{1pt}\colorbox{Blue!40}{0.842$\pm$0.009}} & {\setlength{\fboxsep}{1pt}\colorbox{Red!40}{0.913$\pm$0.010}} & {\setlength{\fboxsep}{1pt}\colorbox{Red!40}{0.943$\pm$0.006}} & {\setlength{\fboxsep}{1pt}\colorbox{Blue!40}{2.8}} \\
    & \cmark & \cmark  & \xmark & 0.805$\pm$0.021 & 0.852$\pm$0.011 & 0.857$\pm$0.020 & 0.724$\pm$0.007 & 0.863$\pm$0.043 & 0.714$\pm$0.100 & 5.7 \\
    & \cmark & \xmark  & \cmark & {\setlength{\fboxsep}{1pt}\colorbox{Blue!40}{0.848$\pm$0.004}} & 0.904$\pm$0.006 & {\setlength{\fboxsep}{1pt}\colorbox{Blue!40}{0.915$\pm$0.004}} & 0.759$\pm$0.005 & 0.882$\pm$0.008 & 0.924$\pm$0.019 & 3.0 \\
    & \xmark & \cmark  & \cmark & 0.779$\pm$0.045 & {\setlength{\fboxsep}{1pt}\colorbox{Blue!40}{0.926$\pm$0.004}} & 0.886$\pm$0.014 & 0.775$\pm$0.021 & 0.877$\pm$0.009 & 0.925$\pm$0.019 & 3.5 \\
    \cline{2-11}
    & \cmark & \cmark  & \cmark & {\setlength{\fboxsep}{1pt}\colorbox{Red!40}{0.874$\pm$0.004}} & {\setlength{\fboxsep}{1pt}\colorbox{Red!40}{0.931$\pm$0.008}} & {\setlength{\fboxsep}{1pt}\colorbox{Red!40}{0.930$\pm$0.011}} & {\setlength{\fboxsep}{1pt}\colorbox{Red!40}{0.853$\pm$0.008}} & 0.880$\pm$0.012 & {\setlength{\fboxsep}{1pt}\colorbox{Blue!40}{0.926$\pm$0.019}} & {\setlength{\fboxsep}{1pt}\colorbox{Red!40}{\textbf{1.7}}} \\
    \hline
    \hline
    \multirow{7}{*}{\rotatebox[origin=c]{90}{\structack}}
    & \cmark & \xmark  & \xmark & 0.819$\pm$0.023 & 0.680$\pm$0.165 & 0.894$\pm$0.014 & 0.868$\pm$0.006 & 0.942$\pm$0.003 & N.A & 6.0 \\
    & \xmark & \cmark  & \xmark & 0.876$\pm$0.010 & 0.883$\pm$0.006 & 0.886$\pm$0.028 & {\setlength{\fboxsep}{1pt}\colorbox{Blue!40}{0.934$\pm$0.001}} & 0.856$\pm$0.017 & N.A & 5.0 \\
    & \xmark & \xmark  & \cmark & 0.842$\pm$0.000 & 0.886$\pm$0.000 & 0.823$\pm$0.000 & 0.854$\pm$0.000 & 0.948$\pm$0.000 & N.A & 5.6 \\
    & \cmark & \cmark  & \xmark & 0.894$\pm$0.014 & 0.878$\pm$0.005 & {\setlength{\fboxsep}{1pt}\colorbox{Blue!40}{0.952$\pm$0.009}} & 0.907$\pm$0.001 & 0.878$\pm$0.053 & N.A & 4.4 \\
    & \cmark & \xmark  & \cmark & {\setlength{\fboxsep}{1pt}\colorbox{Blue!40}{0.906$\pm$0.002}} & 0.916$\pm$0.003 & 0.940$\pm$0.005 & 0.904$\pm$0.001 & 0.966$\pm$0.002 & N.A & 3.2 \\
    & \xmark & \cmark  & \cmark & 0.898$\pm$0.025 & {\setlength{\fboxsep}{1pt}\colorbox{Blue!40}{0.936$\pm$0.008}} & 0.918$\pm$0.013 & 0.924$\pm$0.003 & {\setlength{\fboxsep}{1pt}\colorbox{Red!40}{0.969$\pm$0.002}} & N.A & {\setlength{\fboxsep}{1pt}\colorbox{Blue!40}{2.6}} \\
    \cline{2-11}
    & \cmark & \cmark  & \cmark & {\setlength{\fboxsep}{1pt}\colorbox{Red!40}{0.941$\pm$0.004}} & {\setlength{\fboxsep}{1pt}\colorbox{Red!40}{0.950$\pm$0.006}} & {\setlength{\fboxsep}{1pt}\colorbox{Red!40}{0.965$\pm$0.002}} & {\setlength{\fboxsep}{1pt}\colorbox{Red!40}{0.939$\pm$0.002}} & {\setlength{\fboxsep}{1pt}\colorbox{Blue!40}{0.968$\pm$0.003}} & N.A & {\setlength{\fboxsep}{1pt}\colorbox{Red!40}{\textbf{1.2}}} \\
    \hline
    \hline
    \multirow{7}{*}{\rotatebox[origin=c]{90}{\metattack}}
    & \cmark & \xmark  & \xmark & 0.696$\pm$0.025 & 0.617$\pm$0.067 & 0.613$\pm$0.016 & O.O.M & 0.939$\pm$0.005 & 0.901$\pm$0.009 & 6.0 \\
    & \xmark & \cmark  & \xmark & 0.823$\pm$0.036 & 0.798$\pm$0.016 & 0.772$\pm$0.026 & O.O.M & 0.856$\pm$0.012 & 0.881$\pm$0.022 & 5.6 \\
    & \xmark & \xmark  & \cmark & 0.840$\pm$0.004 & 0.886$\pm$0.005 & 0.791$\pm$0.011 & O.O.M & 0.940$\pm$0.005 & {\setlength{\fboxsep}{1pt}\colorbox{Red!40}{0.972$\pm$0.002}} & 3.2 \\
    & \cmark & \cmark  & \xmark & 0.811$\pm$0.022 & 0.778$\pm$0.025 & 0.588$\pm$0.007 & O.O.M & 0.899$\pm$0.112 & 0.699$\pm$0.087 & 6.4 \\
    & \cmark & \xmark  & \cmark & 0.850$\pm$0.005 & 0.867$\pm$0.011 & 0.818$\pm$0.015 & O.O.M & 0.961$\pm$0.004 & 0.969$\pm$0.004 & 3.4 \\
    & \xmark & \cmark  & \cmark & {\setlength{\fboxsep}{1pt}\colorbox{Blue!40}{0.876$\pm$0.013}} & {\setlength{\fboxsep}{1pt}\colorbox{Red!40}{0.906$\pm$0.008}} & {\setlength{\fboxsep}{1pt}\colorbox{Blue!40}{0.847$\pm$0.030}} & O.O.M & {\setlength{\fboxsep}{1pt}\colorbox{Red!40}{0.963$\pm$0.004}} & {\setlength{\fboxsep}{1pt}\colorbox{Blue!40}{0.970$\pm$0.005}} & {\setlength{\fboxsep}{1pt}\colorbox{Blue!40}{1.6}} \\
    \cline{2-11}
    & \cmark & \cmark  & \cmark & {\setlength{\fboxsep}{1pt}\colorbox{Red!40}{0.894$\pm$0.003}} & {\setlength{\fboxsep}{1pt}\colorbox{Blue!40}{0.893$\pm$0.010}} & {\setlength{\fboxsep}{1pt}\colorbox{Red!40}{0.856$\pm$0.016}} & O.O.M & {\setlength{\fboxsep}{1pt}\colorbox{Red!40}{0.963$\pm$0.004}} & {\setlength{\fboxsep}{1pt}\colorbox{Blue!40}{0.970$\pm$0.003}} & {\setlength{\fboxsep}{1pt}\colorbox{Red!40}{\textbf{1.4}}} \\
    \hline
    \hline
    \end{tabular}
}
\vspace{1cm}
\end{table*}

% \clearpage
