# Supplementary material for: On Measuring Unnoticeability of Graph Adversarial Attacks: Observations, New Measure, and Applications
Source: arXiv:2501.05015 source file (2025-01-09)
Supplement: Supplementary file 2 [file 05_q1_appendix.tex]

\begin{table*}[h]
\centering
\caption{\label{tab:exp:q1_5}
The additional experimental results regarding Q1 with an attack rate of 5\%.
\model ranks first in all attack methods w.r.t average rank (AR). O.O.T: out of time ($>$ 3 hours). O.O.M: out of (GPU) memory. N.A: not applicable (specifically, the maximum number of attacks allowed by \structack is exceeded). For each setting (each column), the best and second-best results are in \setlength{\fboxsep}{1pt}\colorbox{Red!40}{red} and \setlength{\fboxsep}{1pt}\colorbox{Blue!40}{blue}, respectively.
}
\resizebox{!}{0.47\textheight}{
    \begin{tabular}{c||c||c|c|c|c|c|c||c}
    \hline
    \multirow{12}{*}{\rotatebox[origin=c]{90}{\random}}
    & \svd & 0.688$\pm$0.015 & 0.626$\pm$0.017 & 0.795$\pm$0.007 & 0.835$\pm$0.004 & 0.935$\pm$0.003 & {\setlength{\fboxsep}{1pt}\colorbox{Blue!40}{0.953$\pm$0.002}} & 5.8 \\
    & \cosine & 0.803$\pm$0.014 & {\setlength{\fboxsep}{1pt}\colorbox{Blue!40}{0.893$\pm$0.010}} & 0.795$\pm$0.008 & 0.831$\pm$0.004 & 0.560$\pm$0.010 & 0.486$\pm$0.006 & 6.5 \\
    \cline{2-9}
    & \degreelg & 0.664$\pm$0.012 & 0.616$\pm$0.008 & 0.762$\pm$0.009 & 0.810$\pm$0.006 & 0.845$\pm$0.005 & 0.893$\pm$0.002 & 8.7 \\
    & \lclg & 0.592$\pm$0.021 & 0.614$\pm$0.006 & 0.607$\pm$0.019 & 0.677$\pm$0.011 & 0.766$\pm$0.005 & 0.841$\pm$0.002 & 10.5 \\
    & \homophilylg & 0.642$\pm$0.007 & 0.630$\pm$0.008 & 0.674$\pm$0.010 & 0.722$\pm$0.009 & 0.697$\pm$0.015 & 0.640$\pm$0.016 & 9.7 \\
    \cline{2-9}
    & \gcn & 0.779$\pm$0.014 & 0.769$\pm$0.023 & {\setlength{\fboxsep}{1pt}\colorbox{Blue!40}{0.837$\pm$0.028}} & 0.917$\pm$0.008 & 0.951$\pm$0.003 & 0.942$\pm$0.003 & {\setlength{\fboxsep}{1pt}\colorbox{Blue!40}{4.3}} \\
    & \gcnsvd & 0.685$\pm$0.018 & 0.627$\pm$0.117 & 0.771$\pm$0.017 & {\setlength{\fboxsep}{1pt}\colorbox{Blue!40}{0.925$\pm$0.005}} & 0.930$\pm$0.002 & 0.924$\pm$0.003 & 6.2 \\
    & \rgcn & {\setlength{\fboxsep}{1pt}\colorbox{Blue!40}{0.838$\pm$0.011}} & 0.817$\pm$0.021 & 0.801$\pm$0.156 & 0.920$\pm$0.006 & 0.525$\pm$0.045 & 0.585$\pm$0.043 & 5.8 \\
    & \mediangcn & 0.790$\pm$0.029 & 0.776$\pm$0.029 & 0.700$\pm$0.119 & O.O.T & 0.653$\pm$0.174 & O.O.T & 8.8 \\
    & \gnnguard & 0.788$\pm$0.071 & 0.779$\pm$0.029 & 0.812$\pm$0.007 & 0.924$\pm$0.006 & 0.919$\pm$0.038 & 0.905$\pm$0.003 & 4.5 \\
    & \metagc & 0.728$\pm$0.018 & 0.704$\pm$0.018 & 0.719$\pm$0.035 & 0.831$\pm$0.004 & {\setlength{\fboxsep}{1pt}\colorbox{Blue!40}{0.973$\pm$0.002}} & 0.950$\pm$0.009 & 5.8 \\
    \cline{2-9}
    & \model(Proposed) & {\setlength{\fboxsep}{1pt}\colorbox{Red!40}{0.890$\pm$0.020}} & {\setlength{\fboxsep}{1pt}\colorbox{Red!40}{0.932$\pm$0.011}} & {\setlength{\fboxsep}{1pt}\colorbox{Red!40}{0.916$\pm$0.003}} & {\setlength{\fboxsep}{1pt}\colorbox{Red!40}{0.933$\pm$0.004}} & {\setlength{\fboxsep}{1pt}\colorbox{Red!40}{0.976$\pm$0.002}} & {\setlength{\fboxsep}{1pt}\colorbox{Red!40}{0.978$\pm$0.001}} & {\setlength{\fboxsep}{1pt}\colorbox{Red!40}{\textbf{1.0}}} \\
    \hline
    \hline
    \multirow{12}{*}{\rotatebox[origin=c]{90}{\dice}}
    & \svd & 0.677$\pm$0.006 & 0.616$\pm$0.006 & 0.785$\pm$0.010 & 0.829$\pm$0.008 & 0.922$\pm$0.008 & 0.945$\pm$0.002 & 6.7 \\
    & \cosine & 0.827$\pm$0.008 & {\setlength{\fboxsep}{1pt}\colorbox{Blue!40}{0.904$\pm$0.009}} & 0.803$\pm$0.011 & 0.843$\pm$0.006 & 0.565$\pm$0.009 & 0.484$\pm$0.007 & 6.3 \\
    \cline{2-9}
    & \degreelg & 0.664$\pm$0.014 & 0.618$\pm$0.009 & 0.757$\pm$0.016 & 0.806$\pm$0.009 & 0.838$\pm$0.007 & 0.885$\pm$0.004 & 8.3 \\
    & \lclg & 0.595$\pm$0.018 & 0.610$\pm$0.020 & 0.608$\pm$0.025 & 0.676$\pm$0.007 & 0.761$\pm$0.015 & 0.834$\pm$0.007 & 10.7 \\
    & \homophilylg & 0.636$\pm$0.025 & 0.658$\pm$0.010 & 0.677$\pm$0.021 & 0.724$\pm$0.016 & 0.699$\pm$0.015 & 0.633$\pm$0.012 & 10.0 \\
    \cline{2-9}
    & \gcn & 0.802$\pm$0.013 & 0.808$\pm$0.019 & {\setlength{\fboxsep}{1pt}\colorbox{Blue!40}{0.842$\pm$0.016}} & 0.925$\pm$0.005 & {\setlength{\fboxsep}{1pt}\colorbox{Blue!40}{0.952$\pm$0.004}} & 0.942$\pm$0.005 & {\setlength{\fboxsep}{1pt}\colorbox{Blue!40}{3.5}} \\
    & \gcnsvd & 0.692$\pm$0.014 & 0.758$\pm$0.030 & 0.781$\pm$0.022 & {\setlength{\fboxsep}{1pt}\colorbox{Blue!40}{0.938$\pm$0.002}} & 0.950$\pm$0.005 & 0.921$\pm$0.003 & 5.2 \\
    & \rgcn & {\setlength{\fboxsep}{1pt}\colorbox{Blue!40}{0.847$\pm$0.013}} & 0.792$\pm$0.156 & 0.749$\pm$0.185 & 0.925$\pm$0.001 & 0.535$\pm$0.050 & 0.571$\pm$0.142 & 6.7 \\
    & \mediangcn & 0.830$\pm$0.027 & 0.773$\pm$0.036 & 0.748$\pm$0.093 & O.O.T & 0.770$\pm$0.172 & O.O.T & 8.2 \\
    & \gnnguard & 0.804$\pm$0.076 & 0.769$\pm$0.035 & 0.813$\pm$0.009 & 0.935$\pm$0.008 & 0.918$\pm$0.036 & 0.918$\pm$0.018 & 4.8 \\
    & \metagc & 0.737$\pm$0.022 & 0.714$\pm$0.022 & 0.694$\pm$0.053 & 0.825$\pm$0.007 & 0.948$\pm$0.003 & {\setlength{\fboxsep}{1pt}\colorbox{Blue!40}{0.949$\pm$0.008}} & 6.5 \\
    \cline{2-9}
    & \model(Proposed) & {\setlength{\fboxsep}{1pt}\colorbox{Red!40}{0.914$\pm$0.017}} & {\setlength{\fboxsep}{1pt}\colorbox{Red!40}{0.941$\pm$0.006}} & {\setlength{\fboxsep}{1pt}\colorbox{Red!40}{0.925$\pm$0.018}} & {\setlength{\fboxsep}{1pt}\colorbox{Red!40}{0.944$\pm$0.003}} & {\setlength{\fboxsep}{1pt}\colorbox{Red!40}{0.971$\pm$0.005}} & {\setlength{\fboxsep}{1pt}\colorbox{Red!40}{0.962$\pm$0.007}} & {\setlength{\fboxsep}{1pt}\colorbox{Red!40}{\textbf{1.0}}} \\
    \hline
    \hline
    \multirow{12}{*}{\rotatebox[origin=c]{90}{\pgd}}
    & \svd & {\setlength{\fboxsep}{1pt}\colorbox{Blue!40}{0.846$\pm$0.005}} & 0.737$\pm$0.007 & {\setlength{\fboxsep}{1pt}\colorbox{Blue!40}{0.909$\pm$0.002}} & 0.384$\pm$0.022 & {\setlength{\fboxsep}{1pt}\colorbox{Blue!40}{0.952$\pm$0.002}} & 0.839$\pm$0.275 & {\setlength{\fboxsep}{1pt}\colorbox{Blue!40}{4.7}} \\
    & \cosine & 0.815$\pm$0.016 & {\setlength{\fboxsep}{1pt}\colorbox{Blue!40}{0.881$\pm$0.006}} & 0.819$\pm$0.010 & 0.844$\pm$0.009 & 0.586$\pm$0.008 & 0.520$\pm$0.022 & 6.2 \\
    \cline{2-9}
    & \degreelg & 0.774$\pm$0.019 & 0.726$\pm$0.014 & 0.894$\pm$0.007 & 0.269$\pm$0.023 & {\setlength{\fboxsep}{1pt}\colorbox{Red!40}{0.966$\pm$0.005}} & 0.794$\pm$0.384 & 5.7 \\
    & \lclg & 0.693$\pm$0.035 & 0.727$\pm$0.014 & 0.724$\pm$0.041 & 0.737$\pm$0.008 & 0.895$\pm$0.012 & {\setlength{\fboxsep}{1pt}\colorbox{Red!40}{0.959$\pm$0.001}} & 6.7 \\
    & \homophilylg & 0.735$\pm$0.020 & 0.710$\pm$0.023 & 0.838$\pm$0.018 & {\setlength{\fboxsep}{1pt}\colorbox{Red!40}{0.897$\pm$0.015}} & 0.829$\pm$0.013 & 0.757$\pm$0.075 & 7.0 \\
    \cline{2-9}
    & \gcn & 0.645$\pm$0.033 & 0.718$\pm$0.123 & 0.790$\pm$0.025 & 0.611$\pm$0.038 & 0.935$\pm$0.005 & 0.853$\pm$0.161 & 7.5 \\
    & \gcnsvd & 0.770$\pm$0.021 & 0.783$\pm$0.020 & 0.878$\pm$0.010 & 0.615$\pm$0.035 & 0.949$\pm$0.008 & 0.792$\pm$0.356 & {\setlength{\fboxsep}{1pt}\colorbox{Blue!40}{4.7}} \\
    & \rgcn & 0.585$\pm$0.024 & 0.743$\pm$0.119 & 0.626$\pm$0.135 & 0.532$\pm$0.039 & 0.538$\pm$0.030 & 0.582$\pm$0.061 & 9.8 \\
    & \mediangcn & 0.657$\pm$0.113 & 0.763$\pm$0.045 & 0.724$\pm$0.086 & O.O.T & 0.822$\pm$0.184 & O.O.T & 9.7 \\
    & \gnnguard & 0.764$\pm$0.014 & 0.741$\pm$0.033 & 0.832$\pm$0.016 & 0.512$\pm$0.043 & 0.942$\pm$0.002 & 0.733$\pm$0.412 & 6.7 \\
    & \metagc & 0.738$\pm$0.033 & 0.680$\pm$0.035 & 0.783$\pm$0.021 & 0.657$\pm$0.037 & 0.907$\pm$0.013 & 0.908$\pm$0.056 & 7.2 \\
    \cline{2-9}
    & \model(Proposed) & {\setlength{\fboxsep}{1pt}\colorbox{Red!40}{0.877$\pm$0.018}} & {\setlength{\fboxsep}{1pt}\colorbox{Red!40}{0.935$\pm$0.005}} & {\setlength{\fboxsep}{1pt}\colorbox{Red!40}{0.935$\pm$0.012}} & {\setlength{\fboxsep}{1pt}\colorbox{Blue!40}{0.865$\pm$0.011}} & 0.911$\pm$0.018 & {\setlength{\fboxsep}{1pt}\colorbox{Blue!40}{0.922$\pm$0.054}} & {\setlength{\fboxsep}{1pt}\colorbox{Red!40}{\textbf{2.2}}} \\
    \hline
    \hline
    \multirow{12}{*}{\rotatebox[origin=c]{90}{\structack}}
    & \svd & 0.842$\pm$0.000 & 0.747$\pm$0.000 & 0.917$\pm$0.000 & 0.934$\pm$0.000 & 0.952$\pm$0.000 & N.A & 5.2 \\
    & \cosine & 0.831$\pm$0.000 & {\setlength{\fboxsep}{1pt}\colorbox{Blue!40}{0.892$\pm$0.000}} & 0.836$\pm$0.000 & 0.833$\pm$0.000 & 0.566$\pm$0.000 & N.A & 7.8 \\
    \cline{2-9}
    & \degreelg & {\setlength{\fboxsep}{1pt}\colorbox{Blue!40}{0.913$\pm$0.004}} & 0.819$\pm$0.008 & {\setlength{\fboxsep}{1pt}\colorbox{Blue!40}{0.965$\pm$0.001}} & {\setlength{\fboxsep}{1pt}\colorbox{Red!40}{0.975$\pm$0.000}} & 0.856$\pm$0.001 & N.A & {\setlength{\fboxsep}{1pt}\colorbox{Blue!40}{3.0}} \\
    & \lclg & 0.640$\pm$0.012 & 0.688$\pm$0.017 & 0.750$\pm$0.008 & 0.756$\pm$0.004 & 0.711$\pm$0.004 & N.A & 10.4 \\
    & \homophilylg & 0.779$\pm$0.008 & 0.735$\pm$0.009 & 0.864$\pm$0.004 & 0.868$\pm$0.002 & 0.705$\pm$0.005 & N.A & 8.2 \\
    \cline{2-9}
    & \gcn & 0.843$\pm$0.014 & 0.802$\pm$0.013 & 0.910$\pm$0.009 & 0.835$\pm$0.005 & 0.953$\pm$0.004 & N.A & 5.6 \\
    & \gcnsvd & 0.852$\pm$0.013 & 0.780$\pm$0.018 & 0.918$\pm$0.004 & {\setlength{\fboxsep}{1pt}\colorbox{Blue!40}{0.955$\pm$0.002}} & 0.951$\pm$0.004 & N.A & 3.8 \\
    & \rgcn & 0.845$\pm$0.017 & 0.580$\pm$0.177 & 0.760$\pm$0.181 & 0.877$\pm$0.008 & 0.549$\pm$0.052 & N.A & 9.0 \\
    & \mediangcn & 0.682$\pm$0.133 & 0.670$\pm$0.130 & 0.724$\pm$0.084 & O.O.T & 0.684$\pm$0.188 & N.A & 11.2 \\
    & \gnnguard & 0.889$\pm$0.010 & 0.778$\pm$0.025 & 0.911$\pm$0.009 & 0.896$\pm$0.003 & 0.927$\pm$0.035 & N.A & 5.0 \\
    & \metagc & 0.752$\pm$0.008 & 0.727$\pm$0.030 & 0.771$\pm$0.030 & 0.875$\pm$0.007 & {\setlength{\fboxsep}{1pt}\colorbox{Blue!40}{0.981$\pm$0.001}} & N.A & 7.4 \\
    \cline{2-9}
    & \model(Proposed) & {\setlength{\fboxsep}{1pt}\colorbox{Red!40}{0.950$\pm$0.006}} & {\setlength{\fboxsep}{1pt}\colorbox{Red!40}{0.950$\pm$0.003}} & {\setlength{\fboxsep}{1pt}\colorbox{Red!40}{0.975$\pm$0.002}} & 0.937$\pm$0.001 & {\setlength{\fboxsep}{1pt}\colorbox{Red!40}{0.984$\pm$0.001}} & N.A & {\setlength{\fboxsep}{1pt}\colorbox{Red!40}{\textbf{1.4}}} \\
    \hline
    \hline
    \multirow{12}{*}{\rotatebox[origin=c]{90}{\metattack}}
    & \svd & 0.805$\pm$0.004 & 0.637$\pm$0.027 & 0.768$\pm$0.041 & {\setlength{\fboxsep}{1pt}\colorbox{Blue!40}{0.925$\pm$0.004}} & 0.966$\pm$0.003 & {\setlength{\fboxsep}{1pt}\colorbox{Red!40}{0.989$\pm$0.000}} & 4.5 \\
    & \cosine & 0.835$\pm$0.006 & {\setlength{\fboxsep}{1pt}\colorbox{Blue!40}{0.875$\pm$0.006}} & {\setlength{\fboxsep}{1pt}\colorbox{Blue!40}{0.789$\pm$0.006}} & 0.870$\pm$0.005 & 0.551$\pm$0.007 & 0.453$\pm$0.006 & 5.8 \\
    \cline{2-9}
    & \degreelg & 0.681$\pm$0.009 & 0.561$\pm$0.015 & 0.701$\pm$0.017 & 0.828$\pm$0.010 & {\setlength{\fboxsep}{1pt}\colorbox{Red!40}{0.970$\pm$0.002}} & {\setlength{\fboxsep}{1pt}\colorbox{Blue!40}{0.983$\pm$0.001}} & 7.2 \\
    & \lclg & 0.693$\pm$0.072 & 0.721$\pm$0.014 & 0.632$\pm$0.266 & 0.901$\pm$0.007 & 0.948$\pm$0.005 & 0.973$\pm$0.001 & 6.7 \\
    & \homophilylg & 0.703$\pm$0.015 & 0.661$\pm$0.019 & 0.777$\pm$0.012 & 0.894$\pm$0.006 & 0.771$\pm$0.010 & 0.666$\pm$0.017 & 7.2 \\
    \cline{2-9}
    & \gcn & 0.755$\pm$0.015 & 0.714$\pm$0.019 & 0.677$\pm$0.049 & 0.835$\pm$0.012 & 0.947$\pm$0.005 & 0.919$\pm$0.004 & 7.7 \\
    & \gcnsvd & 0.801$\pm$0.005 & 0.701$\pm$0.113 & 0.776$\pm$0.032 & {\setlength{\fboxsep}{1pt}\colorbox{Red!40}{0.939$\pm$0.002}} & {\setlength{\fboxsep}{1pt}\colorbox{Red!40}{0.970$\pm$0.003}} & 0.937$\pm$0.022 & {\setlength{\fboxsep}{1pt}\colorbox{Blue!40}{4.0}} \\
    & \rgcn & 0.756$\pm$0.160 & 0.607$\pm$0.094 & 0.682$\pm$0.094 & 0.823$\pm$0.016 & 0.519$\pm$0.022 & 0.520$\pm$0.029 & 9.7 \\
    & \mediangcn & {\setlength{\fboxsep}{1pt}\colorbox{Blue!40}{0.840$\pm$0.031}} & 0.750$\pm$0.024 & 0.751$\pm$0.046 & O.O.T & 0.733$\pm$0.234 & O.O.T & 7.3 \\
    & \gnnguard & 0.824$\pm$0.019 & 0.701$\pm$0.014 & 0.635$\pm$0.013 & 0.844$\pm$0.014 & 0.954$\pm$0.004 & 0.932$\pm$0.009 & 6.8 \\
    & \metagc & 0.683$\pm$0.028 & 0.678$\pm$0.030 & 0.668$\pm$0.046 & nan$\pm$nan & 0.963$\pm$0.006 & 0.938$\pm$0.013 & 8.5 \\
    \cline{2-9}
    & \model(Proposed) & {\setlength{\fboxsep}{1pt}\colorbox{Red!40}{0.922$\pm$0.004}} & {\setlength{\fboxsep}{1pt}\colorbox{Red!40}{0.900$\pm$0.007}} & {\setlength{\fboxsep}{1pt}\colorbox{Red!40}{0.873$\pm$0.017}} & 0.894$\pm$0.008 & 0.967$\pm$0.004 & 0.980$\pm$0.001 & {\setlength{\fboxsep}{1pt}\colorbox{Red!40}{\textbf{2.2}}} \\
    \hline
    \hline
    \end{tabular}
}
\end{table*}

\begin{table*}[h]
\centering
\caption{\label{tab:exp:q1_15}
The additional experimental results regarding Q1 with an attack rate of 15\%.
\model ranks first in all attack methods w.r.t average rank (AR). O.O.T: out of time ($>$ 3 hours). O.O.M: out of (GPU) memory. N.A: not applicable (specifically, the maximum number of attacks allowed by \structack is exceeded). For each setting (each column), the best and second-best results are in \setlength{\fboxsep}{1pt}\colorbox{Red!40}{red} and \setlength{\fboxsep}{1pt}\colorbox{Blue!40}{blue}, respectively.
}
\resizebox{!}{0.47\textheight}{
    \begin{tabular}{c||c||c|c|c|c|c|c||c}
    \hline
    & \multirow{2}{*}{\textbf{Method}} & \multicolumn{6}{c||}{\textbf{Datasets}} & \multirow{2}{*}{\textbf{AR}} \\
    \cline{3-8}
    & & \cora & \citeseer & \coraml & \lastfmasia & \chameleon & \squirrel & \\
    \hline
    \hline
    \multirow{12}{*}{\rotatebox[origin=c]{90}{\random}}
    & \svd & 0.697$\pm$0.006 & 0.638$\pm$0.006 & 0.794$\pm$0.005 & 0.835$\pm$0.001 & 0.937$\pm$0.003 & {\setlength{\fboxsep}{1pt}\colorbox{Blue!40}{0.953$\pm$0.001}} & 5.0 \\
    & \cosine & {\setlength{\fboxsep}{1pt}\colorbox{Blue!40}{0.804$\pm$0.005}} & {\setlength{\fboxsep}{1pt}\colorbox{Blue!40}{0.892$\pm$0.005}} & 0.794$\pm$0.004 & 0.834$\pm$0.000 & 0.561$\pm$0.004 & 0.487$\pm$0.001 & 6.2 \\
    \cline{2-9}
    & \degreelg & 0.670$\pm$0.006 & 0.624$\pm$0.006 & 0.756$\pm$0.006 & 0.809$\pm$0.002 & 0.847$\pm$0.002 & 0.892$\pm$0.001 & 8.0 \\
    & \lclg & 0.594$\pm$0.005 & 0.609$\pm$0.006 & 0.617$\pm$0.013 & 0.688$\pm$0.004 & 0.775$\pm$0.003 & 0.857$\pm$0.001 & 10.3 \\
    & \homophilylg & 0.641$\pm$0.010 & 0.636$\pm$0.006 & 0.675$\pm$0.008 & 0.732$\pm$0.003 & 0.697$\pm$0.012 & 0.624$\pm$0.003 & 9.3 \\
    \cline{2-9}
    & \gcn & 0.776$\pm$0.017 & 0.772$\pm$0.025 & {\setlength{\fboxsep}{1pt}\colorbox{Blue!40}{0.817$\pm$0.004}} & 0.907$\pm$0.008 & 0.930$\pm$0.003 & 0.935$\pm$0.010 & {\setlength{\fboxsep}{1pt}\colorbox{Blue!40}{3.7}} \\
    & \gcnsvd & 0.657$\pm$0.009 & 0.612$\pm$0.103 & 0.750$\pm$0.005 & 0.914$\pm$0.003 & 0.890$\pm$0.022 & 0.923$\pm$0.002 & 6.8 \\
    & \rgcn & 0.751$\pm$0.145 & 0.631$\pm$0.182 & 0.661$\pm$0.119 & 0.910$\pm$0.005 & 0.573$\pm$0.010 & 0.555$\pm$0.025 & 8.0 \\
    & \mediangcn & 0.718$\pm$0.114 & 0.727$\pm$0.106 & 0.615$\pm$0.076 & O.O.T & 0.559$\pm$0.069 & O.O.T & 10.0 \\
    & \gnnguard & 0.795$\pm$0.008 & 0.735$\pm$0.028 & 0.810$\pm$0.007 & {\setlength{\fboxsep}{1pt}\colorbox{Blue!40}{0.919$\pm$0.002}} & 0.878$\pm$0.032 & 0.914$\pm$0.011 & 4.0 \\
    & \metagc & 0.730$\pm$0.007 & 0.702$\pm$0.016 & 0.712$\pm$0.034 & 0.826$\pm$0.009 & {\setlength{\fboxsep}{1pt}\colorbox{Blue!40}{0.969$\pm$0.002}} & 0.948$\pm$0.008 & 5.5 \\
    \cline{2-9}
    & \model(Proposed) & {\setlength{\fboxsep}{1pt}\colorbox{Red!40}{0.891$\pm$0.006}} & {\setlength{\fboxsep}{1pt}\colorbox{Red!40}{0.933$\pm$0.005}} & {\setlength{\fboxsep}{1pt}\colorbox{Red!40}{0.912$\pm$0.006}} & {\setlength{\fboxsep}{1pt}\colorbox{Red!40}{0.927$\pm$0.002}} & {\setlength{\fboxsep}{1pt}\colorbox{Red!40}{0.971$\pm$0.003}} & {\setlength{\fboxsep}{1pt}\colorbox{Red!40}{0.974$\pm$0.001}} & {\setlength{\fboxsep}{1pt}\colorbox{Red!40}{\textbf{1.0}}} \\
    \hline
    \hline
    \multirow{12}{*}{\rotatebox[origin=c]{90}{\dice}}
    & \svd & 0.653$\pm$0.007 & 0.606$\pm$0.013 & 0.770$\pm$0.004 & 0.816$\pm$0.005 & 0.895$\pm$0.005 & 0.932$\pm$0.001 & 6.5 \\
    & \cosine & 0.813$\pm$0.008 & {\setlength{\fboxsep}{1pt}\colorbox{Blue!40}{0.894$\pm$0.003}} & 0.806$\pm$0.003 & 0.841$\pm$0.004 & 0.565$\pm$0.005 & 0.482$\pm$0.005 & 6.2 \\
    \cline{2-9}
    & \degreelg & 0.652$\pm$0.009 & 0.606$\pm$0.012 & 0.761$\pm$0.007 & 0.806$\pm$0.006 & 0.844$\pm$0.008 & 0.885$\pm$0.002 & 8.2 \\
    & \lclg & 0.577$\pm$0.009 & 0.596$\pm$0.015 & 0.616$\pm$0.012 & 0.681$\pm$0.009 & 0.774$\pm$0.006 & 0.847$\pm$0.003 & 10.5 \\
    & \homophilylg & 0.627$\pm$0.007 & 0.639$\pm$0.015 & 0.686$\pm$0.012 & 0.729$\pm$0.006 & 0.695$\pm$0.006 & 0.622$\pm$0.009 & 9.7 \\
    \cline{2-9}
    & \gcn & 0.773$\pm$0.015 & 0.755$\pm$0.022 & {\setlength{\fboxsep}{1pt}\colorbox{Blue!40}{0.836$\pm$0.018}} & 0.907$\pm$0.005 & {\setlength{\fboxsep}{1pt}\colorbox{Blue!40}{0.937$\pm$0.013}} & {\setlength{\fboxsep}{1pt}\colorbox{Blue!40}{0.936$\pm$0.001}} & {\setlength{\fboxsep}{1pt}\colorbox{Blue!40}{3.3}} \\
    & \gcnsvd & 0.654$\pm$0.014 & 0.694$\pm$0.028 & 0.754$\pm$0.008 & {\setlength{\fboxsep}{1pt}\colorbox{Blue!40}{0.928$\pm$0.003}} & 0.923$\pm$0.004 & 0.921$\pm$0.001 & 5.2 \\
    & \rgcn & {\setlength{\fboxsep}{1pt}\colorbox{Blue!40}{0.815$\pm$0.022}} & 0.830$\pm$0.014 & 0.696$\pm$0.176 & 0.910$\pm$0.004 & 0.549$\pm$0.012 & 0.557$\pm$0.018 & 6.7 \\
    & \mediangcn & 0.687$\pm$0.139 & 0.663$\pm$0.119 & 0.707$\pm$0.098 & O.O.T & 0.625$\pm$0.184 & O.O.T & 9.5 \\
    & \gnnguard & 0.781$\pm$0.003 & 0.717$\pm$0.071 & 0.812$\pm$0.012 & 0.925$\pm$0.001 & 0.876$\pm$0.043 & 0.916$\pm$0.014 & 4.3 \\
    & \metagc & 0.717$\pm$0.041 & 0.717$\pm$0.026 & 0.656$\pm$0.054 & 0.810$\pm$0.008 & 0.896$\pm$0.002 & {\setlength{\fboxsep}{1pt}\colorbox{Red!40}{0.946$\pm$0.009}} & 5.8 \\
    \cline{2-9}
    & \model(Proposed) & {\setlength{\fboxsep}{1pt}\colorbox{Red!40}{0.890$\pm$0.009}} & {\setlength{\fboxsep}{1pt}\colorbox{Red!40}{0.936$\pm$0.010}} & {\setlength{\fboxsep}{1pt}\colorbox{Red!40}{0.930$\pm$0.006}} & {\setlength{\fboxsep}{1pt}\colorbox{Red!40}{0.933$\pm$0.002}} & {\setlength{\fboxsep}{1pt}\colorbox{Red!40}{0.945$\pm$0.009}} & 0.916$\pm$0.005 & {\setlength{\fboxsep}{1pt}\colorbox{Red!40}{\textbf{1.7}}} \\
    \hline
    \hline
    \multirow{12}{*}{\rotatebox[origin=c]{90}{\pgd}}
    & \svd & 0.765$\pm$0.008 & 0.710$\pm$0.007 & {\setlength{\fboxsep}{1pt}\colorbox{Blue!40}{0.853$\pm$0.007}} & 0.316$\pm$0.031 & {\setlength{\fboxsep}{1pt}\colorbox{Blue!40}{0.887$\pm$0.003}} & 0.928$\pm$0.016 & {\setlength{\fboxsep}{1pt}\colorbox{Blue!40}{4.2}} \\
    & \cosine & {\setlength{\fboxsep}{1pt}\colorbox{Blue!40}{0.800$\pm$0.006}} & {\setlength{\fboxsep}{1pt}\colorbox{Blue!40}{0.881$\pm$0.004}} & 0.801$\pm$0.005 & 0.838$\pm$0.007 & 0.587$\pm$0.003 & 0.521$\pm$0.003 & 5.7 \\
    \cline{2-9}
    & \degreelg & 0.710$\pm$0.008 & 0.667$\pm$0.003 & 0.840$\pm$0.009 & 0.267$\pm$0.019 & {\setlength{\fboxsep}{1pt}\colorbox{Red!40}{0.934$\pm$0.008}} & {\setlength{\fboxsep}{1pt}\colorbox{Blue!40}{0.940$\pm$0.005}} & 5.7 \\
    & \lclg & 0.636$\pm$0.057 & 0.677$\pm$0.011 & 0.690$\pm$0.035 & 0.618$\pm$0.067 & 0.865$\pm$0.011 & {\setlength{\fboxsep}{1pt}\colorbox{Red!40}{0.954$\pm$0.005}} & 6.5 \\
    & \homophilylg & 0.728$\pm$0.009 & 0.694$\pm$0.015 & 0.784$\pm$0.005 & {\setlength{\fboxsep}{1pt}\colorbox{Red!40}{0.898$\pm$0.005}} & 0.823$\pm$0.013 & 0.739$\pm$0.013 & 6.2 \\
    \cline{2-9}
    & \gcn & 0.613$\pm$0.029 & 0.741$\pm$0.007 & 0.752$\pm$0.017 & 0.517$\pm$0.014 & 0.862$\pm$0.011 & 0.881$\pm$0.014 & 6.8 \\
    & \gcnsvd & 0.734$\pm$0.017 & 0.699$\pm$0.112 & 0.829$\pm$0.018 & 0.484$\pm$0.015 & 0.883$\pm$0.008 & 0.924$\pm$0.008 & 4.7 \\
    & \rgcn & 0.591$\pm$0.011 & 0.501$\pm$0.008 & 0.660$\pm$0.092 & 0.409$\pm$0.019 & 0.523$\pm$0.049 & 0.604$\pm$0.056 & 10.8 \\
    & \mediangcn & 0.545$\pm$0.029 & 0.670$\pm$0.120 & 0.733$\pm$0.019 & O.O.T & 0.785$\pm$0.167 & O.O.T & 11.0 \\
    & \gnnguard & 0.703$\pm$0.032 & 0.734$\pm$0.025 & 0.776$\pm$0.013 & 0.400$\pm$0.022 & 0.879$\pm$0.006 & 0.905$\pm$0.015 & 6.5 \\
    & \metagc & 0.704$\pm$0.015 & 0.682$\pm$0.024 & 0.743$\pm$0.028 & 0.585$\pm$0.022 & 0.845$\pm$0.018 & 0.923$\pm$0.009 & 7.0 \\
    \cline{2-9}
    & \model(Proposed) & {\setlength{\fboxsep}{1pt}\colorbox{Red!40}{0.863$\pm$0.008}} & {\setlength{\fboxsep}{1pt}\colorbox{Red!40}{0.910$\pm$0.009}} & {\setlength{\fboxsep}{1pt}\colorbox{Red!40}{0.914$\pm$0.006}} & {\setlength{\fboxsep}{1pt}\colorbox{Blue!40}{0.841$\pm$0.008}} & 0.849$\pm$0.030 & 0.915$\pm$0.028 & {\setlength{\fboxsep}{1pt}\colorbox{Red!40}{\textbf{3.0}}} \\
    \hline
    \hline
    \multirow{12}{*}{\rotatebox[origin=c]{90}{\structack}}
    & \svd & 0.786$\pm$0.000 & 0.773$\pm$0.000 & 0.851$\pm$0.000 & 0.844$\pm$0.000 & N.A & N.A & 6.5 \\
    & \cosine & 0.829$\pm$0.000 & {\setlength{\fboxsep}{1pt}\colorbox{Blue!40}{0.894$\pm$0.000}} & 0.825$\pm$0.000 & 0.872$\pm$0.000 & N.A & N.A & 4.2 \\
    \cline{2-9}
    & \degreelg & {\setlength{\fboxsep}{1pt}\colorbox{Blue!40}{0.849$\pm$0.003}} & 0.849$\pm$0.002 & 0.885$\pm$0.001 & 0.850$\pm$0.000 & N.A & N.A & 3.8 \\
    & \lclg & 0.553$\pm$0.009 & 0.693$\pm$0.006 & 0.572$\pm$0.006 & 0.656$\pm$0.001 & N.A & N.A & 11.0 \\
    & \homophilylg & 0.687$\pm$0.004 & 0.752$\pm$0.006 & 0.715$\pm$0.002 & 0.728$\pm$0.002 & N.A & N.A & 9.2 \\
    \cline{2-9}
    & \gcn & 0.787$\pm$0.023 & 0.798$\pm$0.011 & 0.885$\pm$0.014 & 0.862$\pm$0.009 & N.A & N.A & 4.8 \\
    & \gcnsvd & 0.789$\pm$0.017 & 0.795$\pm$0.021 & 0.843$\pm$0.006 & 0.884$\pm$0.003 & N.A & N.A & 4.8 \\
    & \rgcn & 0.754$\pm$0.110 & 0.565$\pm$0.144 & 0.587$\pm$0.116 & 0.866$\pm$0.005 & N.A & N.A & 8.8 \\
    & \mediangcn & 0.546$\pm$0.044 & 0.736$\pm$0.075 & 0.568$\pm$0.053 & O.O.T & N.A & N.A & 11.2 \\
    & \gnnguard & 0.831$\pm$0.020 & 0.760$\pm$0.020 & {\setlength{\fboxsep}{1pt}\colorbox{Blue!40}{0.892$\pm$0.002}} & {\setlength{\fboxsep}{1pt}\colorbox{Blue!40}{0.891$\pm$0.003}} & N.A & N.A & {\setlength{\fboxsep}{1pt}\colorbox{Blue!40}{3.5}} \\
    & \metagc & 0.743$\pm$0.009 & 0.726$\pm$0.028 & 0.740$\pm$0.042 & 0.835$\pm$0.008 & N.A & N.A & 9.0 \\
    \cline{2-9}
    & \model(Proposed) & {\setlength{\fboxsep}{1pt}\colorbox{Red!40}{0.933$\pm$0.002}} & {\setlength{\fboxsep}{1pt}\colorbox{Red!40}{0.955$\pm$0.003}} & {\setlength{\fboxsep}{1pt}\colorbox{Red!40}{0.959$\pm$0.006}} & {\setlength{\fboxsep}{1pt}\colorbox{Red!40}{0.934$\pm$0.003}} & N.A & N.A & {\setlength{\fboxsep}{1pt}\colorbox{Red!40}{\textbf{1.0}}} \\
    \hline
    \hline
    \multirow{12}{*}{\rotatebox[origin=c]{90}{\metattack}}
    & \svd & 0.643$\pm$0.012 & 0.554$\pm$0.012 & 0.710$\pm$0.013 & O.O.M & 0.921$\pm$0.002 & 0.941$\pm$0.007 & 7.4 \\
    & \cosine & {\setlength{\fboxsep}{1pt}\colorbox{Blue!40}{0.839$\pm$0.002}} & {\setlength{\fboxsep}{1pt}\colorbox{Red!40}{0.891$\pm$0.004}} & {\setlength{\fboxsep}{1pt}\colorbox{Blue!40}{0.790$\pm$0.009}} & O.O.M & 0.557$\pm$0.004 & 0.448$\pm$0.004 & 5.4 \\
    \cline{2-9}
    & \degreelg & 0.488$\pm$0.009 & 0.373$\pm$0.004 & 0.610$\pm$0.005 & O.O.M & 0.932$\pm$0.002 & 0.952$\pm$0.003 & 8.2 \\
    & \lclg & 0.607$\pm$0.120 & 0.697$\pm$0.009 & 0.731$\pm$0.040 & O.O.M & 0.916$\pm$0.002 & {\setlength{\fboxsep}{1pt}\colorbox{Red!40}{0.967$\pm$0.001}} & 5.8 \\
    & \homophilylg & 0.702$\pm$0.012 & 0.656$\pm$0.009 & 0.755$\pm$0.009 & O.O.M & 0.755$\pm$0.015 & 0.589$\pm$0.007 & 6.2 \\
    \cline{2-9}
    & \gcn & 0.657$\pm$0.045 & 0.601$\pm$0.051 & 0.584$\pm$0.018 & O.O.M & 0.930$\pm$0.004 & 0.883$\pm$0.011 & 8.2 \\
    & \gcnsvd & 0.614$\pm$0.040 & 0.652$\pm$0.088 & 0.671$\pm$0.010 & O.O.M & 0.941$\pm$0.004 & 0.933$\pm$0.007 & 6.4 \\
    & \rgcn & 0.695$\pm$0.104 & 0.651$\pm$0.089 & 0.562$\pm$0.077 & O.O.M & 0.614$\pm$0.061 & 0.531$\pm$0.026 & 9.0 \\
    & \mediangcn & 0.650$\pm$0.147 & 0.736$\pm$0.044 & 0.734$\pm$0.060 & O.O.M & 0.556$\pm$0.125 & O.O.T & 7.8 \\
    & \gnnguard & 0.724$\pm$0.048 & 0.615$\pm$0.057 & 0.528$\pm$0.029 & O.O.M & 0.933$\pm$0.006 & 0.884$\pm$0.005 & 7.0 \\
    & \metagc & 0.700$\pm$0.021 & 0.684$\pm$0.024 & 0.665$\pm$0.052 & O.O.M & {\setlength{\fboxsep}{1pt}\colorbox{Blue!40}{0.948$\pm$0.004}} & 0.925$\pm$0.012 & {\setlength{\fboxsep}{1pt}\colorbox{Blue!40}{5.2}} \\
    \cline{2-9}
    & \model(Proposed) & {\setlength{\fboxsep}{1pt}\colorbox{Red!40}{0.875$\pm$0.007}} & {\setlength{\fboxsep}{1pt}\colorbox{Blue!40}{0.882$\pm$0.009}} & {\setlength{\fboxsep}{1pt}\colorbox{Red!40}{0.834$\pm$0.020}} & O.O.M & {\setlength{\fboxsep}{1pt}\colorbox{Red!40}{0.956$\pm$0.003}} & {\setlength{\fboxsep}{1pt}\colorbox{Blue!40}{0.957$\pm$0.003}} & {\setlength{\fboxsep}{1pt}\colorbox{Red!40}{\textbf{1.4}}} \\
    \hline
    \hline
    \end{tabular}
}
\end{table*}

\begin{table*}[h]
\centering
\caption{\label{tab:exp:q1_20}
The additional experimental results regarding Q1 with an attack rate of 20\%.
\model ranks first in all attack methods w.r.t average rank (AR). O.O.T: out of time ($>$ 3 hours). O.O.M: out of (GPU) memory. N.A: not applicable (specifically, the maximum number of attacks allowed by \structack is exceeded). For each setting (each column), the best and second-best results are in \setlength{\fboxsep}{1pt}\colorbox{Red!40}{red} and \setlength{\fboxsep}{1pt}\colorbox{Blue!40}{blue}, respectively.
}
\resizebox{!}{0.47\textheight}{
    \begin{tabular}{c||c||c|c|c|c|c|c||c}
    \hline
    & \multirow{2}{*}{\textbf{Method}} & \multicolumn{6}{c||}{\textbf{Datasets}} & \multirow{2}{*}{\textbf{AR}} \\
    \cline{3-8}
    & & \cora & \citeseer & \coraml & \lastfmasia & \chameleon & \squirrel & \\
    \hline
    \hline
    \multirow{12}{*}{\rotatebox[origin=c]{90}{\random}}
    & \svd & 0.698$\pm$0.003 & 0.641$\pm$0.007 & {\setlength{\fboxsep}{1pt}\colorbox{Blue!40}{0.796$\pm$0.005}} & 0.835$\pm$0.001 & 0.939$\pm$0.002 & {\setlength{\fboxsep}{1pt}\colorbox{Blue!40}{0.953$\pm$0.001}} & 4.7 \\
    & \cosine & {\setlength{\fboxsep}{1pt}\colorbox{Blue!40}{0.805$\pm$0.005}} & {\setlength{\fboxsep}{1pt}\colorbox{Blue!40}{0.891$\pm$0.003}} & {\setlength{\fboxsep}{1pt}\colorbox{Blue!40}{0.796$\pm$0.005}} & 0.834$\pm$0.001 & 0.562$\pm$0.004 & 0.487$\pm$0.001 & 5.8 \\
    \cline{2-9}
    & \degreelg & 0.668$\pm$0.006 & 0.624$\pm$0.009 & 0.758$\pm$0.006 & 0.810$\pm$0.001 & 0.847$\pm$0.002 & 0.892$\pm$0.001 & 8.0 \\
    & \lclg & 0.587$\pm$0.009 & 0.617$\pm$0.009 & 0.613$\pm$0.011 & 0.693$\pm$0.003 & 0.777$\pm$0.004 & 0.861$\pm$0.002 & 10.0 \\
    & \homophilylg & 0.640$\pm$0.012 & 0.638$\pm$0.015 & 0.674$\pm$0.009 & 0.732$\pm$0.003 & 0.698$\pm$0.010 & 0.613$\pm$0.003 & 9.5 \\
    \cline{2-9}
    & \gcn & 0.766$\pm$0.014 & 0.698$\pm$0.113 & 0.765$\pm$0.025 & 0.907$\pm$0.002 & 0.928$\pm$0.001 & 0.934$\pm$0.008 & 4.7 \\
    & \gcnsvd & 0.663$\pm$0.005 & 0.696$\pm$0.010 & 0.753$\pm$0.006 & 0.911$\pm$0.002 & 0.872$\pm$0.003 & 0.923$\pm$0.002 & 6.3 \\
    & \rgcn & 0.796$\pm$0.053 & 0.755$\pm$0.146 & 0.579$\pm$0.119 & 0.909$\pm$0.002 & 0.544$\pm$0.017 & 0.552$\pm$0.020 & 7.3 \\
    & \mediangcn & 0.675$\pm$0.126 & 0.602$\pm$0.118 & 0.609$\pm$0.080 & O.O.T & 0.602$\pm$0.140 & O.O.T & 10.8 \\
    & \gnnguard & 0.764$\pm$0.047 & 0.703$\pm$0.019 & 0.774$\pm$0.036 & {\setlength{\fboxsep}{1pt}\colorbox{Blue!40}{0.916$\pm$0.003}} & 0.878$\pm$0.033 & 0.910$\pm$0.015 & {\setlength{\fboxsep}{1pt}\colorbox{Blue!40}{4.3}} \\
    & \metagc & 0.730$\pm$0.006 & 0.703$\pm$0.015 & 0.721$\pm$0.034 & 0.823$\pm$0.008 & {\setlength{\fboxsep}{1pt}\colorbox{Blue!40}{0.967$\pm$0.001}} & 0.948$\pm$0.008 & 5.2 \\
    \cline{2-9}
    & \model(Proposed) & {\setlength{\fboxsep}{1pt}\colorbox{Red!40}{0.887$\pm$0.006}} & {\setlength{\fboxsep}{1pt}\colorbox{Red!40}{0.931$\pm$0.003}} & {\setlength{\fboxsep}{1pt}\colorbox{Red!40}{0.906$\pm$0.007}} & {\setlength{\fboxsep}{1pt}\colorbox{Red!40}{0.926$\pm$0.003}} & {\setlength{\fboxsep}{1pt}\colorbox{Red!40}{0.972$\pm$0.001}} & {\setlength{\fboxsep}{1pt}\colorbox{Red!40}{0.971$\pm$0.001}} & {\setlength{\fboxsep}{1pt}\colorbox{Red!40}{\textbf{1.0}}} \\
    \hline
    \hline
    \multirow{12}{*}{\rotatebox[origin=c]{90}{\dice}}
    & \svd & 0.642$\pm$0.003 & 0.603$\pm$0.008 & 0.749$\pm$0.006 & 0.812$\pm$0.003 & 0.874$\pm$0.005 & 0.923$\pm$0.001 & 7.0 \\
    & \cosine & {\setlength{\fboxsep}{1pt}\colorbox{Blue!40}{0.813$\pm$0.007}} & {\setlength{\fboxsep}{1pt}\colorbox{Blue!40}{0.895$\pm$0.003}} & 0.803$\pm$0.004 & 0.845$\pm$0.004 & 0.565$\pm$0.003 & 0.483$\pm$0.001 & 6.0 \\
    \cline{2-9}
    & \degreelg & 0.649$\pm$0.007 & 0.612$\pm$0.005 & 0.754$\pm$0.006 & 0.809$\pm$0.003 & 0.842$\pm$0.005 & 0.885$\pm$0.001 & 7.5 \\
    & \lclg & 0.584$\pm$0.020 & 0.612$\pm$0.012 & 0.629$\pm$0.012 & 0.683$\pm$0.005 & 0.777$\pm$0.004 & 0.851$\pm$0.002 & 10.0 \\
    & \homophilylg & 0.629$\pm$0.010 & 0.646$\pm$0.013 & 0.683$\pm$0.014 & 0.734$\pm$0.007 & 0.698$\pm$0.006 & 0.616$\pm$0.005 & 9.3 \\
    \cline{2-9}
    & \gcn & 0.751$\pm$0.012 & 0.709$\pm$0.118 & {\setlength{\fboxsep}{1pt}\colorbox{Blue!40}{0.816$\pm$0.007}} & 0.897$\pm$0.004 & {\setlength{\fboxsep}{1pt}\colorbox{Red!40}{0.930$\pm$0.008}} & {\setlength{\fboxsep}{1pt}\colorbox{Blue!40}{0.935$\pm$0.001}} & {\setlength{\fboxsep}{1pt}\colorbox{Blue!40}{3.2}} \\
    & \gcnsvd & 0.654$\pm$0.014 & 0.647$\pm$0.082 & 0.745$\pm$0.011 & {\setlength{\fboxsep}{1pt}\colorbox{Blue!40}{0.924$\pm$0.003}} & 0.908$\pm$0.026 & 0.920$\pm$0.002 & 5.2 \\
    & \rgcn & 0.811$\pm$0.014 & 0.546$\pm$0.113 & 0.797$\pm$0.096 & 0.905$\pm$0.008 & 0.549$\pm$0.027 & 0.572$\pm$0.019 & 7.7 \\
    & \mediangcn & 0.621$\pm$0.133 & 0.684$\pm$0.094 & 0.692$\pm$0.098 & O.O.T & 0.637$\pm$0.183 & O.O.T & 10.0 \\
    & \gnnguard & 0.733$\pm$0.065 & 0.747$\pm$0.024 & 0.807$\pm$0.004 & 0.919$\pm$0.002 & 0.875$\pm$0.039 & 0.915$\pm$0.015 & 3.8 \\
    & \metagc & 0.733$\pm$0.019 & 0.714$\pm$0.028 & 0.653$\pm$0.085 & 0.803$\pm$0.007 & 0.869$\pm$0.005 & {\setlength{\fboxsep}{1pt}\colorbox{Red!40}{0.945$\pm$0.007}} & 6.0 \\
    \cline{2-9}
    & \model(Proposed) & {\setlength{\fboxsep}{1pt}\colorbox{Red!40}{0.897$\pm$0.014}} & {\setlength{\fboxsep}{1pt}\colorbox{Red!40}{0.937$\pm$0.005}} & {\setlength{\fboxsep}{1pt}\colorbox{Red!40}{0.922$\pm$0.010}} & {\setlength{\fboxsep}{1pt}\colorbox{Red!40}{0.928$\pm$0.001}} & {\setlength{\fboxsep}{1pt}\colorbox{Red!40}{0.930$\pm$0.010}} & 0.907$\pm$0.017 & {\setlength{\fboxsep}{1pt}\colorbox{Red!40}{\textbf{1.8}}} \\
    \hline
    \hline
    \multirow{12}{*}{\rotatebox[origin=c]{90}{\pgd}}
    & \svd & 0.733$\pm$0.008 & 0.695$\pm$0.008 & {\setlength{\fboxsep}{1pt}\colorbox{Blue!40}{0.827$\pm$0.006}} & 0.322$\pm$0.024 & 0.857$\pm$0.008 & 0.915$\pm$0.021 & 4.8 \\
    & \cosine & {\setlength{\fboxsep}{1pt}\colorbox{Blue!40}{0.794$\pm$0.004}} & {\setlength{\fboxsep}{1pt}\colorbox{Blue!40}{0.884$\pm$0.004}} & 0.800$\pm$0.004 & {\setlength{\fboxsep}{1pt}\colorbox{Blue!40}{0.838$\pm$0.004}} & 0.584$\pm$0.004 & 0.520$\pm$0.002 & 5.5 \\
    \cline{2-9}
    & \degreelg & 0.689$\pm$0.010 & 0.653$\pm$0.007 & 0.816$\pm$0.003 & 0.282$\pm$0.021 & {\setlength{\fboxsep}{1pt}\colorbox{Red!40}{0.925$\pm$0.009}} & {\setlength{\fboxsep}{1pt}\colorbox{Blue!40}{0.930$\pm$0.005}} & 6.0 \\
    & \lclg & 0.583$\pm$0.131 & 0.664$\pm$0.009 & 0.701$\pm$0.018 & 0.358$\pm$0.008 & 0.852$\pm$0.010 & {\setlength{\fboxsep}{1pt}\colorbox{Red!40}{0.949$\pm$0.005}} & 7.8 \\
    & \homophilylg & 0.710$\pm$0.006 & 0.695$\pm$0.008 & 0.767$\pm$0.006 & {\setlength{\fboxsep}{1pt}\colorbox{Red!40}{0.897$\pm$0.004}} & 0.803$\pm$0.016 & 0.722$\pm$0.011 & 5.8 \\
    \cline{2-9}
    & \gcn & 0.608$\pm$0.018 & 0.669$\pm$0.102 & 0.730$\pm$0.018 & 0.514$\pm$0.010 & 0.855$\pm$0.019 & 0.865$\pm$0.006 & 7.3 \\
    & \gcnsvd & 0.700$\pm$0.010 & 0.734$\pm$0.011 & 0.817$\pm$0.009 & 0.481$\pm$0.020 & {\setlength{\fboxsep}{1pt}\colorbox{Blue!40}{0.864$\pm$0.012}} & 0.909$\pm$0.023 & {\setlength{\fboxsep}{1pt}\colorbox{Blue!40}{4.2}} \\
    & \rgcn & 0.590$\pm$0.025 & 0.600$\pm$0.146 & 0.597$\pm$0.080 & 0.421$\pm$0.020 & 0.506$\pm$0.022 & 0.579$\pm$0.047 & 10.7 \\
    & \mediangcn & 0.578$\pm$0.082 & 0.704$\pm$0.055 & 0.679$\pm$0.033 & O.O.T & 0.706$\pm$0.168 & O.O.T & 10.3 \\
    & \gnnguard & 0.689$\pm$0.024 & 0.715$\pm$0.017 & 0.746$\pm$0.017 & 0.431$\pm$0.020 & 0.863$\pm$0.008 & 0.881$\pm$0.015 & 5.8 \\
    & \metagc & 0.702$\pm$0.031 & 0.679$\pm$0.025 & 0.726$\pm$0.042 & 0.577$\pm$0.022 & 0.824$\pm$0.017 & 0.920$\pm$0.011 & 6.2 \\
    \cline{2-9}
    & \model(Proposed) & {\setlength{\fboxsep}{1pt}\colorbox{Red!40}{0.853$\pm$0.004}} & {\setlength{\fboxsep}{1pt}\colorbox{Red!40}{0.915$\pm$0.007}} & {\setlength{\fboxsep}{1pt}\colorbox{Red!40}{0.906$\pm$0.008}} & 0.837$\pm$0.003 & 0.846$\pm$0.022 & 0.907$\pm$0.035 & {\setlength{\fboxsep}{1pt}\colorbox{Red!40}{\textbf{3.2}}} \\
    \hline
    \hline
    \multirow{12}{*}{\rotatebox[origin=c]{90}{\structack}}
    & \svd & 0.774$\pm$0.000 & 0.785$\pm$0.000 & 0.816$\pm$0.000 & 0.860$\pm$0.000 & N.A & N.A & 5.5 \\
    & \cosine & 0.826$\pm$0.000 & {\setlength{\fboxsep}{1pt}\colorbox{Blue!40}{0.892$\pm$0.000}} & 0.818$\pm$0.000 & 0.863$\pm$0.000 & N.A & N.A & 3.8 \\
    \cline{2-9}
    & \degreelg & {\setlength{\fboxsep}{1pt}\colorbox{Blue!40}{0.833$\pm$0.002}} & 0.850$\pm$0.004 & 0.824$\pm$0.001 & 0.874$\pm$0.000 & N.A & N.A & {\setlength{\fboxsep}{1pt}\colorbox{Blue!40}{3.0}} \\
    & \lclg & 0.555$\pm$0.004 & 0.683$\pm$0.007 & 0.575$\pm$0.005 & 0.680$\pm$0.003 & N.A & N.A & 10.5 \\
    & \homophilylg & 0.659$\pm$0.003 & 0.715$\pm$0.007 & 0.686$\pm$0.004 & 0.768$\pm$0.001 & N.A & N.A & 9.0 \\
    \cline{2-9}
    & \gcn & 0.783$\pm$0.029 & 0.648$\pm$0.188 & {\setlength{\fboxsep}{1pt}\colorbox{Blue!40}{0.831$\pm$0.002}} & 0.844$\pm$0.006 & N.A & N.A & 6.5 \\
    & \gcnsvd & 0.767$\pm$0.013 & 0.722$\pm$0.126 & 0.801$\pm$0.003 & {\setlength{\fboxsep}{1pt}\colorbox{Blue!40}{0.880$\pm$0.004}} & N.A & N.A & 5.8 \\
    & \rgcn & 0.595$\pm$0.121 & 0.498$\pm$0.016 & 0.527$\pm$0.034 & 0.860$\pm$0.006 & N.A & N.A & 10.2 \\
    & \mediangcn & 0.609$\pm$0.102 & 0.650$\pm$0.141 & 0.575$\pm$0.040 & O.O.T & N.A & N.A & 10.5 \\
    & \gnnguard & 0.796$\pm$0.016 & 0.747$\pm$0.046 & 0.830$\pm$0.004 & 0.874$\pm$0.003 & N.A & N.A & 3.8 \\
    & \metagc & 0.739$\pm$0.007 & 0.727$\pm$0.023 & 0.732$\pm$0.041 & 0.837$\pm$0.008 & N.A & N.A & 7.8 \\
    \cline{2-9}
    & \model(Proposed) & {\setlength{\fboxsep}{1pt}\colorbox{Red!40}{0.924$\pm$0.005}} & {\setlength{\fboxsep}{1pt}\colorbox{Red!40}{0.950$\pm$0.007}} & {\setlength{\fboxsep}{1pt}\colorbox{Red!40}{0.945$\pm$0.012}} & {\setlength{\fboxsep}{1pt}\colorbox{Red!40}{0.928$\pm$0.002}} & N.A & N.A & {\setlength{\fboxsep}{1pt}\colorbox{Red!40}{\textbf{1.0}}} \\
    \hline
    \hline
    \multirow{12}{*}{\rotatebox[origin=c]{90}{\metattack}}
    & \svd & 0.598$\pm$0.009 & 0.523$\pm$0.011 & 0.695$\pm$0.013 & O.O.M & 0.895$\pm$0.008 & 0.900$\pm$0.011 & 7.4 \\
    & \cosine & {\setlength{\fboxsep}{1pt}\colorbox{Blue!40}{0.841$\pm$0.003}} & {\setlength{\fboxsep}{1pt}\colorbox{Red!40}{0.895$\pm$0.005}} & {\setlength{\fboxsep}{1pt}\colorbox{Blue!40}{0.789$\pm$0.009}} & O.O.M & 0.554$\pm$0.004 & 0.441$\pm$0.005 & 5.6 \\
    \cline{2-9}
    & \degreelg & 0.438$\pm$0.010 & 0.313$\pm$0.006 & 0.575$\pm$0.009 & O.O.M & 0.908$\pm$0.005 & 0.932$\pm$0.002 & 8.6 \\
    & \lclg & 0.698$\pm$0.007 & 0.697$\pm$0.015 & 0.586$\pm$0.224 & O.O.M & 0.910$\pm$0.005 & {\setlength{\fboxsep}{1pt}\colorbox{Red!40}{0.964$\pm$0.002}} & 4.2 \\
    & \homophilylg & 0.695$\pm$0.006 & 0.663$\pm$0.009 & 0.749$\pm$0.012 & O.O.M & 0.743$\pm$0.015 & 0.568$\pm$0.008 & 6.4 \\
    \cline{2-9}
    & \gcn & 0.624$\pm$0.029 & 0.529$\pm$0.047 & 0.570$\pm$0.029 & O.O.M & 0.911$\pm$0.006 & 0.854$\pm$0.007 & 7.8 \\
    & \gcnsvd & 0.550$\pm$0.027 & 0.636$\pm$0.028 & 0.624$\pm$0.010 & O.O.M & 0.919$\pm$0.008 & 0.917$\pm$0.002 & 6.6 \\
    & \rgcn & 0.693$\pm$0.019 & 0.652$\pm$0.087 & 0.573$\pm$0.086 & O.O.M & 0.578$\pm$0.023 & 0.538$\pm$0.009 & 8.8 \\
    & \mediangcn & 0.592$\pm$0.101 & 0.683$\pm$0.081 & 0.618$\pm$0.030 & O.O.M & 0.583$\pm$0.128 & O.O.T & 8.8 \\
    & \gnnguard & 0.662$\pm$0.005 & 0.417$\pm$0.121 & 0.468$\pm$0.040 & O.O.M & 0.910$\pm$0.008 & 0.841$\pm$0.008 & 8.6 \\
    & \metagc & 0.701$\pm$0.017 & 0.690$\pm$0.023 & 0.660$\pm$0.054 & O.O.M & {\setlength{\fboxsep}{1pt}\colorbox{Blue!40}{0.930$\pm$0.003}} & 0.920$\pm$0.013 & {\setlength{\fboxsep}{1pt}\colorbox{Blue!40}{3.6}} \\
    \cline{2-9}
    & \model(Proposed) & {\setlength{\fboxsep}{1pt}\colorbox{Red!40}{0.860$\pm$0.009}} & {\setlength{\fboxsep}{1pt}\colorbox{Blue!40}{0.869$\pm$0.003}} & {\setlength{\fboxsep}{1pt}\colorbox{Red!40}{0.820$\pm$0.023}} & O.O.M & {\setlength{\fboxsep}{1pt}\colorbox{Red!40}{0.942$\pm$0.006}} & {\setlength{\fboxsep}{1pt}\colorbox{Blue!40}{0.939$\pm$0.002}} & {\setlength{\fboxsep}{1pt}\colorbox{Red!40}{\textbf{1.4}}} \\
    \hline
    \hline
    \end{tabular}
}
\end{table*}
