# Supplementary material for: On Measuring Unnoticeability of Graph Adversarial Attacks: Observations, New Measure, and Applications
Source: arXiv:2501.05015 source file (2025-01-09)
Supplement: Supplementary file 3 [file 05_q2_appendix.tex]

\newcolumntype{C}{>{\centering\arraybackslash}m{0.15\linewidth}}
\begin{table*}
    \centering
    \caption{The additional experimental results regarding Q2 \& Q3 on \random.}
    \resizebox{0.8\textwidth}{!}{
    \begin{tabular}{l||C|C|C|C||C}
        \hline
        % & \multicolumn{4}{c||}{Existing Measures} & \multirow{3}{*}{\textbf{\measure}} \\ 
        % \cline{2-5}
        % & Degree Dist. & Clustering Coeff. & Degree Dist. & Homophily Dist. & \\
        % & (KS test) & (KS test) & (LR test)& (KS test) & \\
        & \textsc{DegreeKS} & \textsc{ClsCoefKS} & \textsc{DegreeLR} & \textsc{HomophKS} & \textbf{\measure} \\
        \hline\hline
        \rotatebox[origin=c]{90}{\cora} & 
        \includegraphics[width=\linewidth]{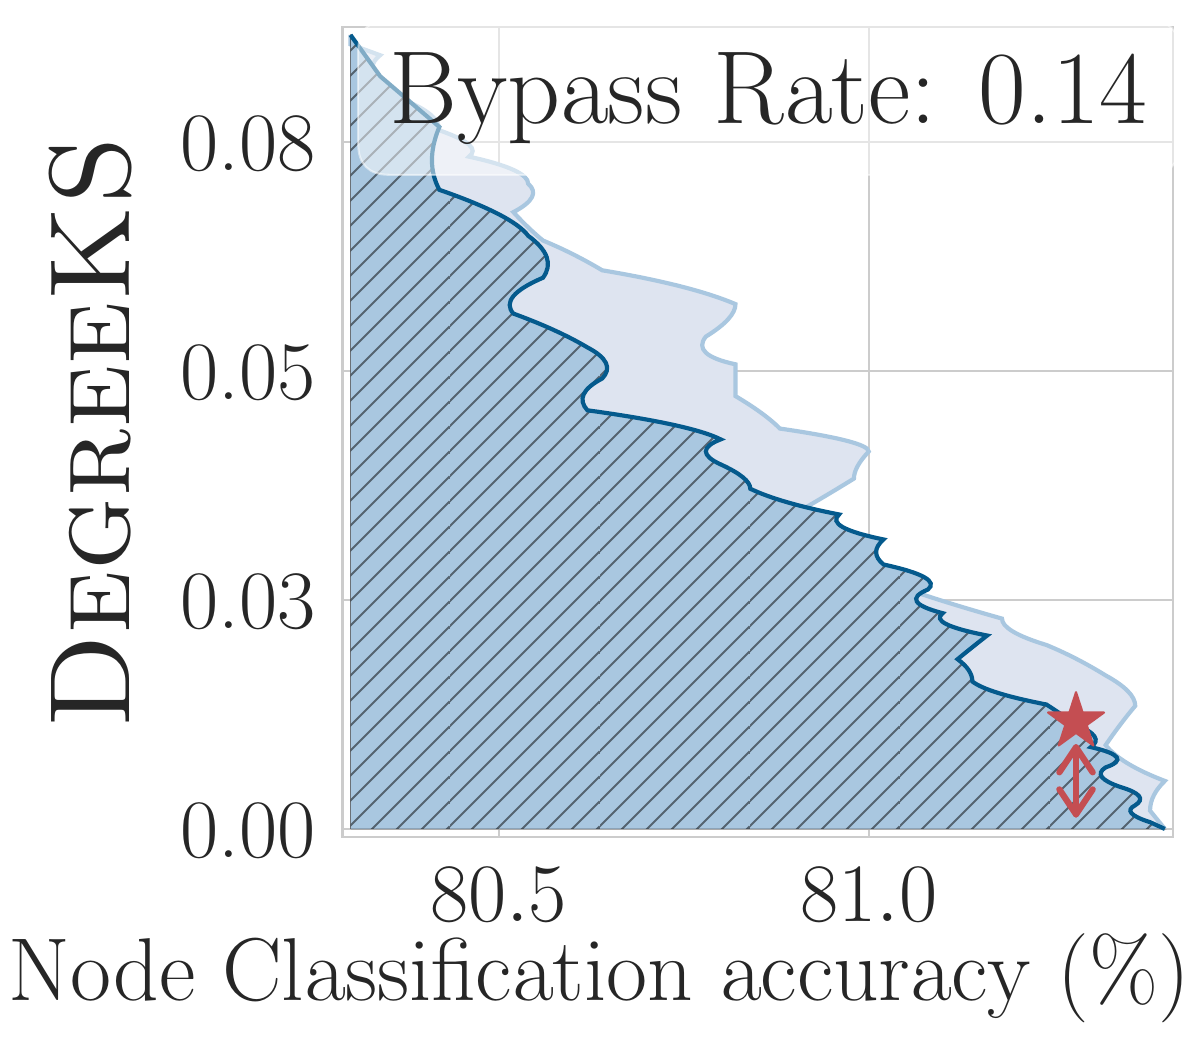} & 
        \includegraphics[width=\linewidth]{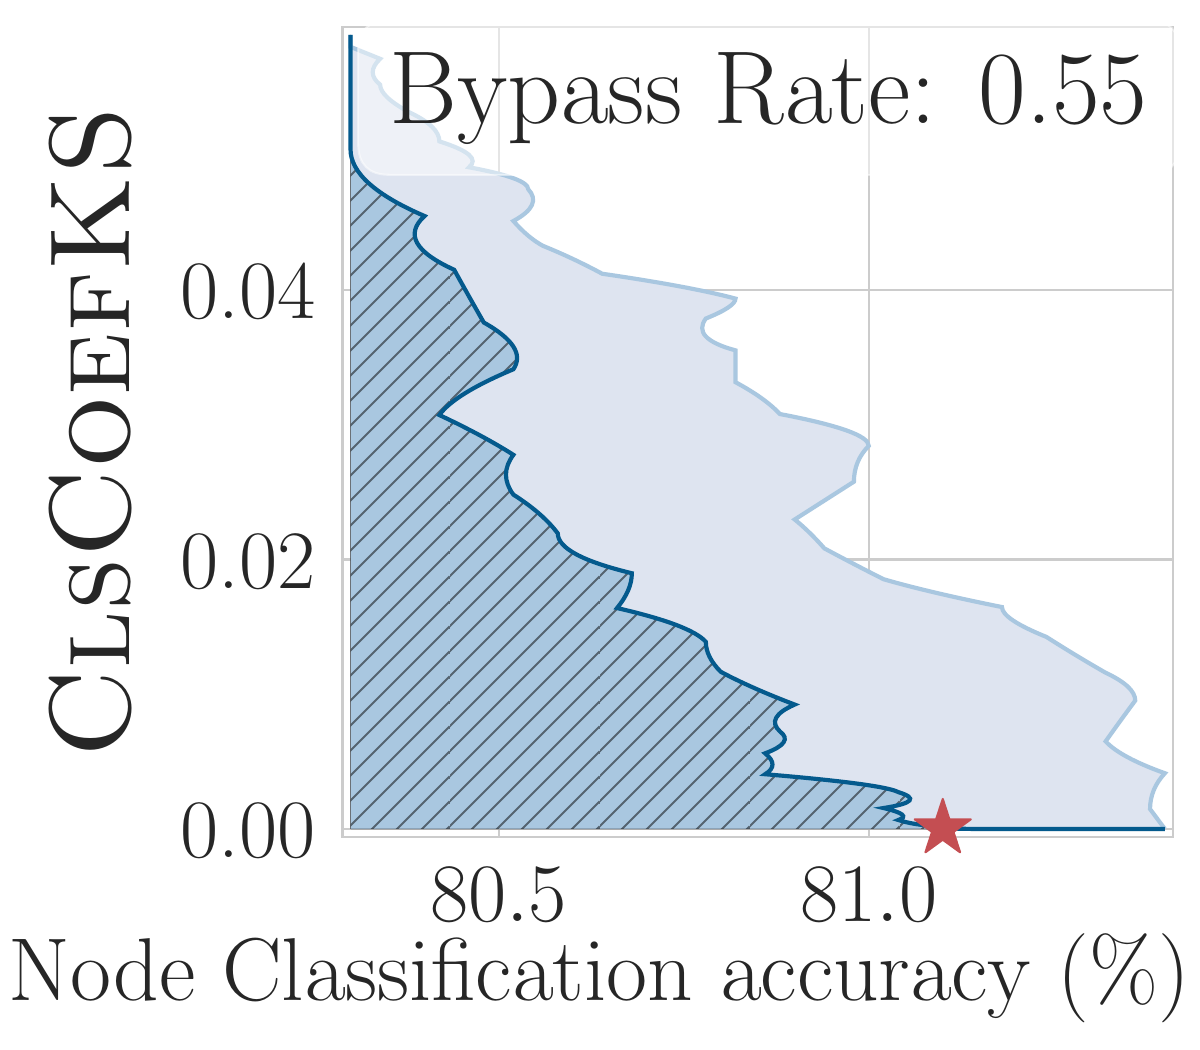} & 
        \includegraphics[width=\linewidth]{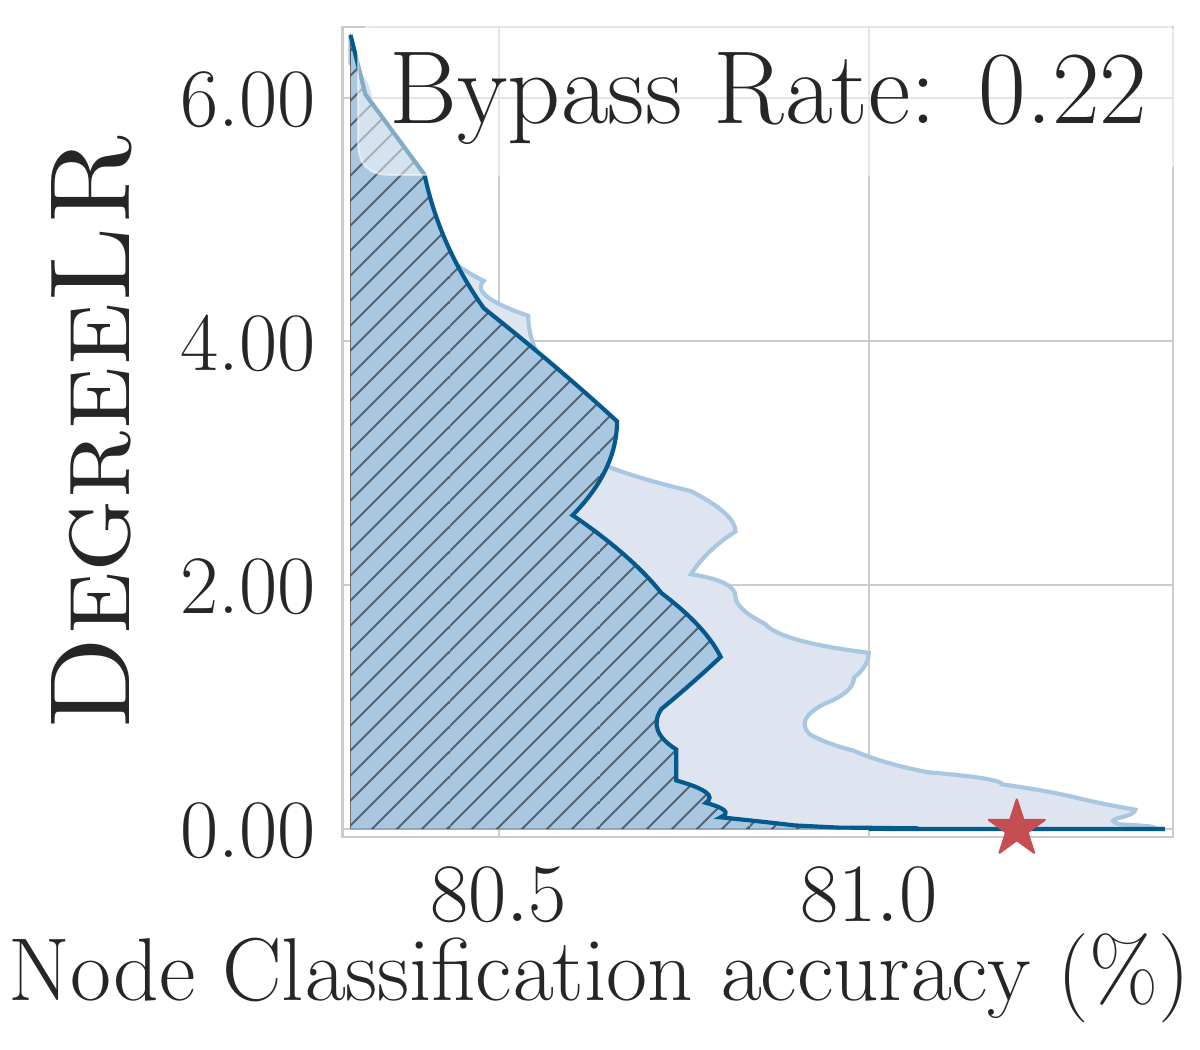} & 
        \includegraphics[width=\linewidth]{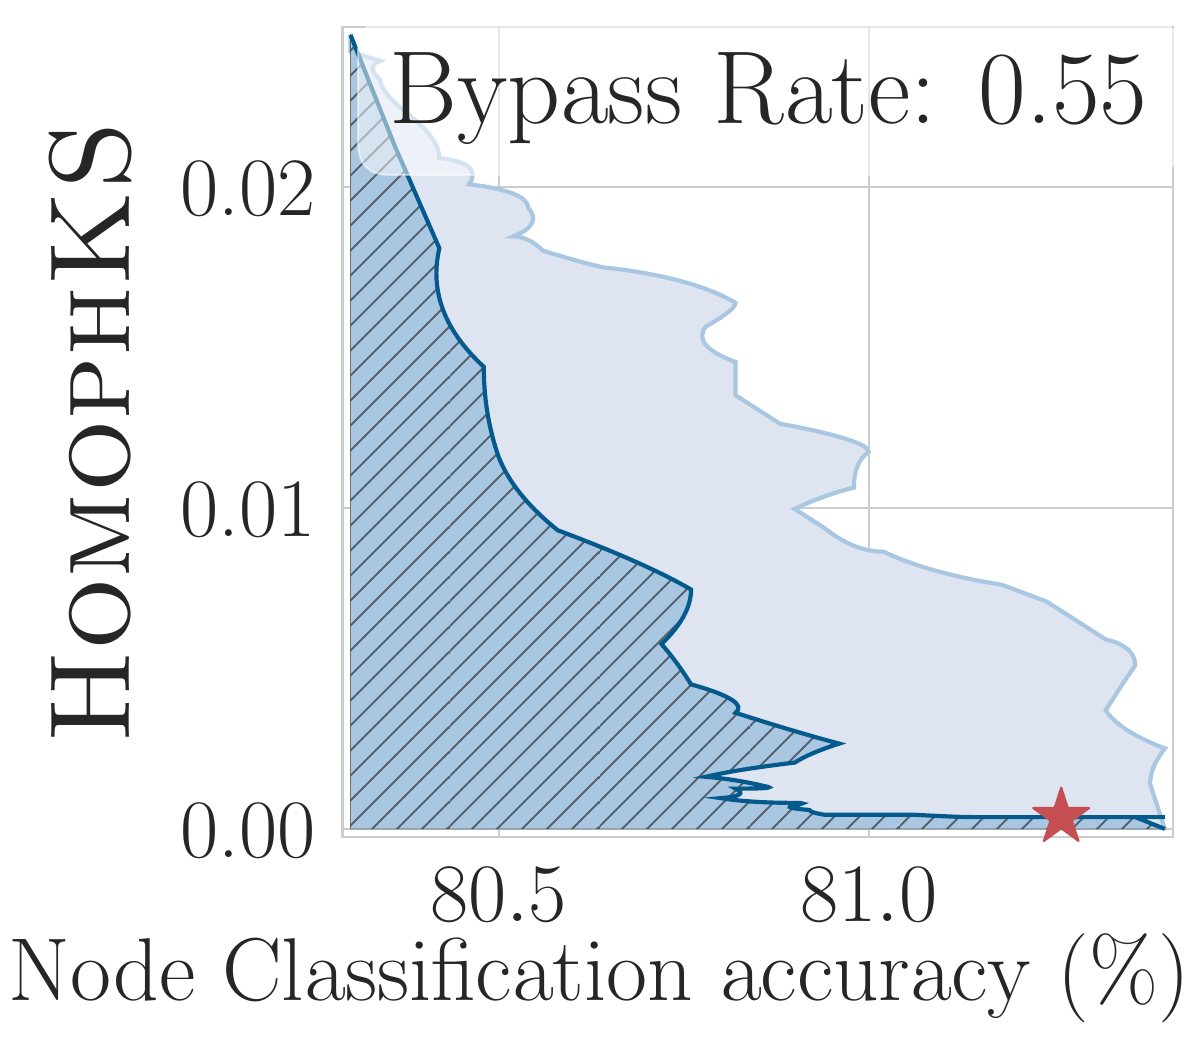} &
        \includegraphics[width=\linewidth]{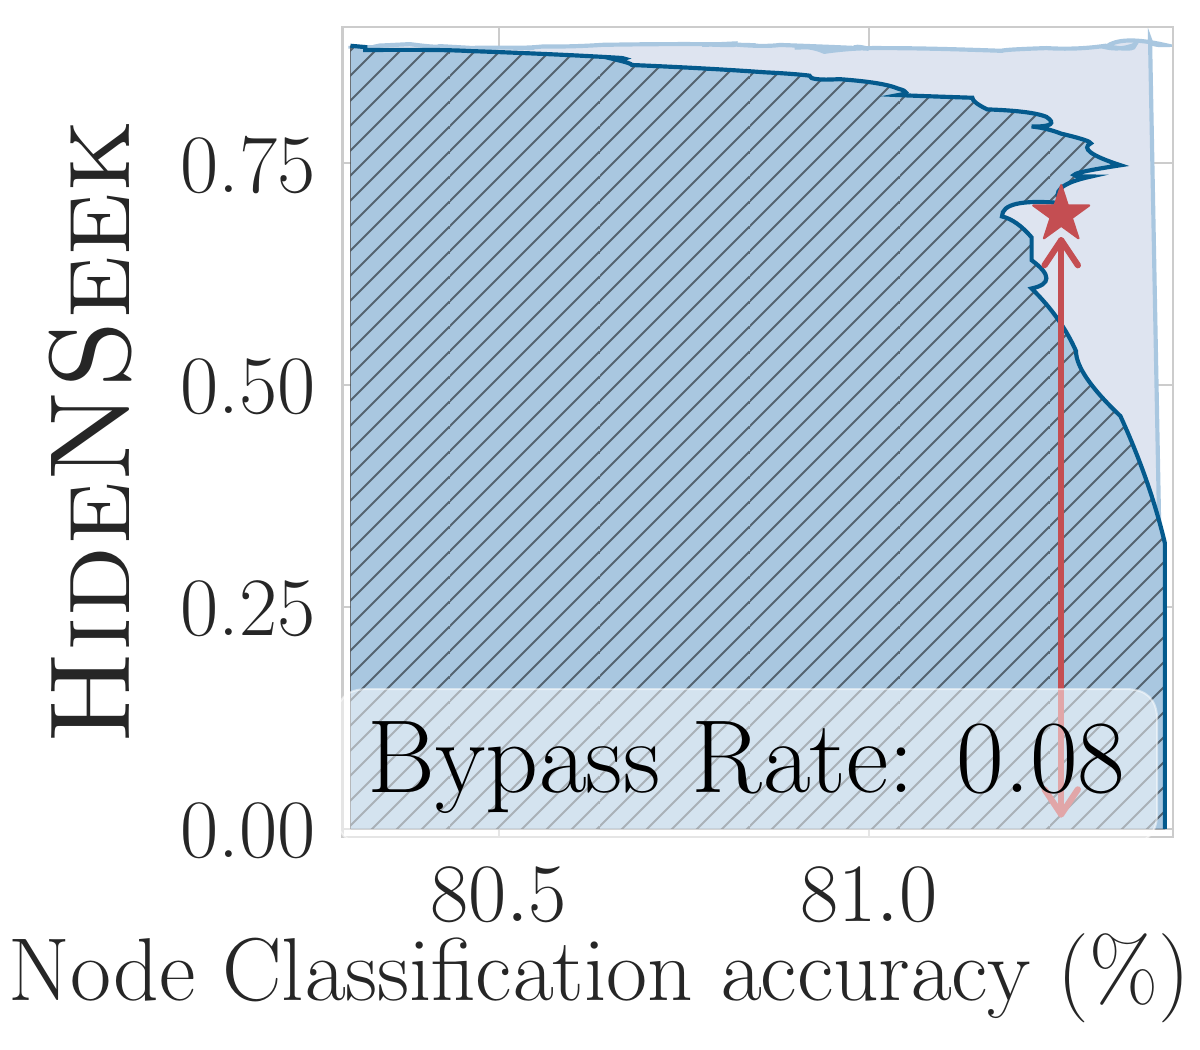} \\
        \hline
        \rotatebox[origin=c]{90}{\citeseer} & 
        \includegraphics[width=\linewidth]{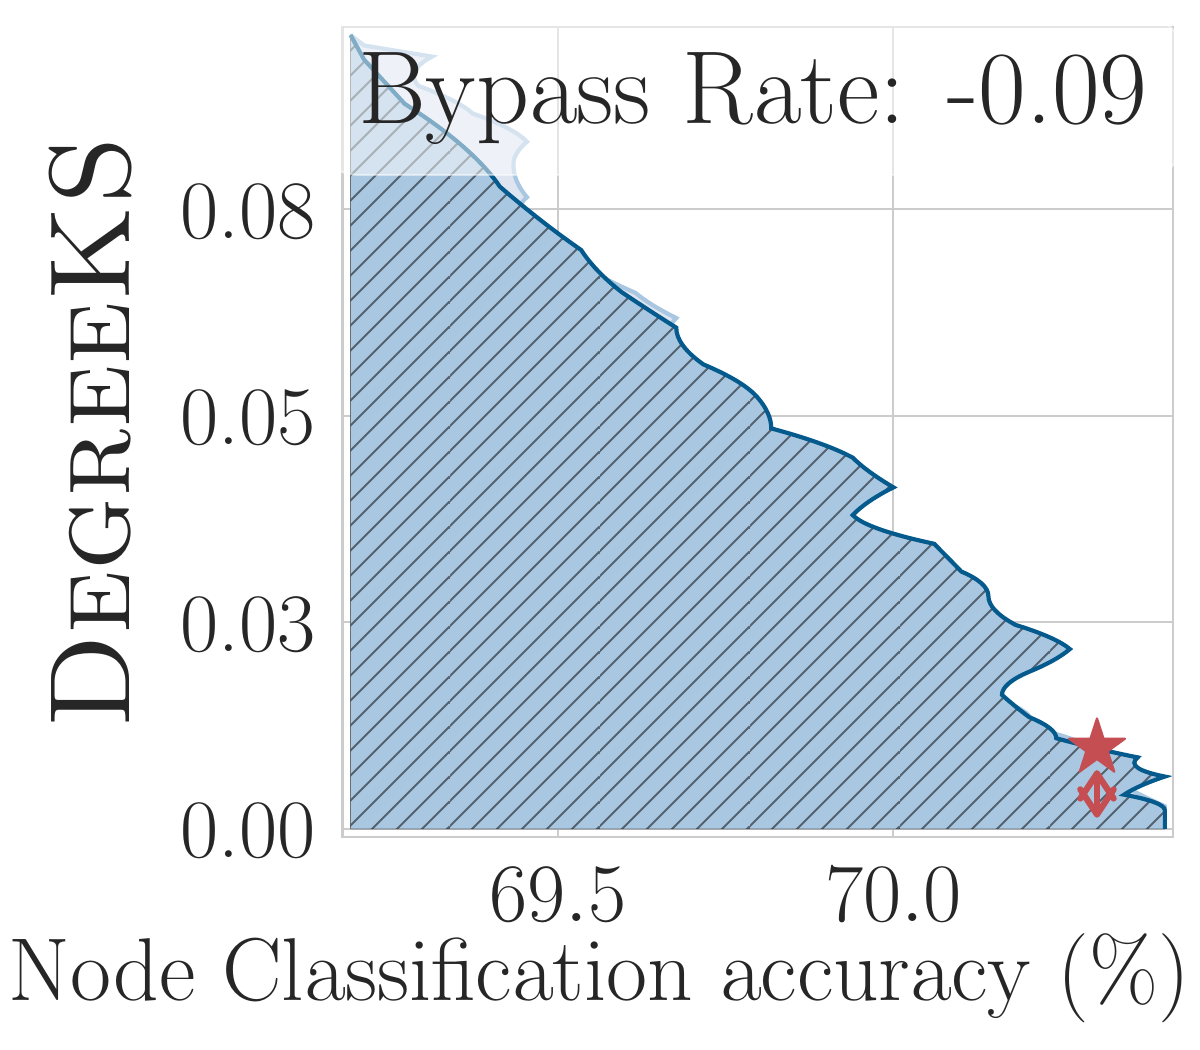} & 
        \includegraphics[width=\linewidth]{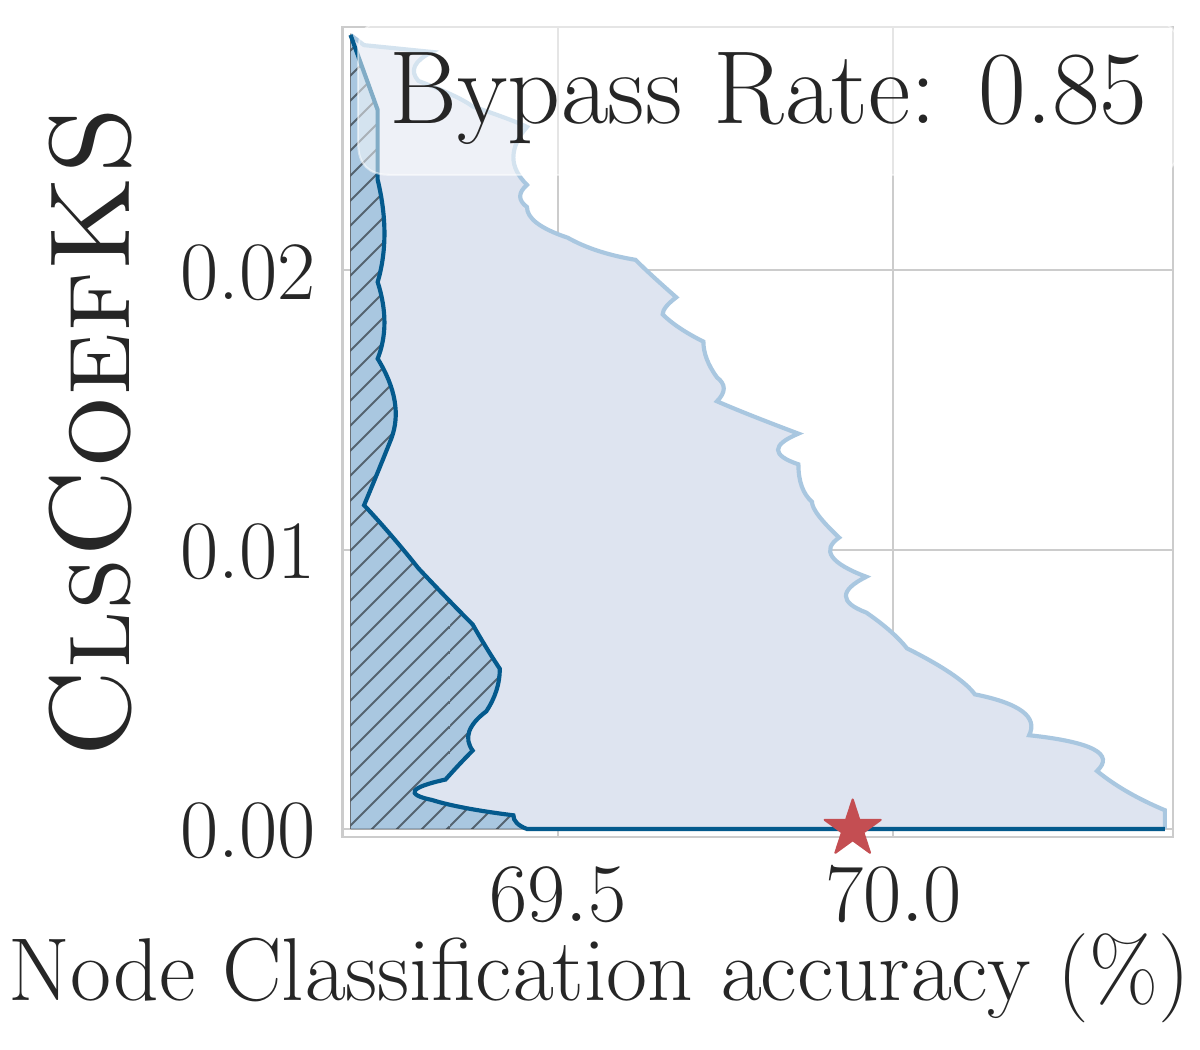} & 
        \includegraphics[width=\linewidth]{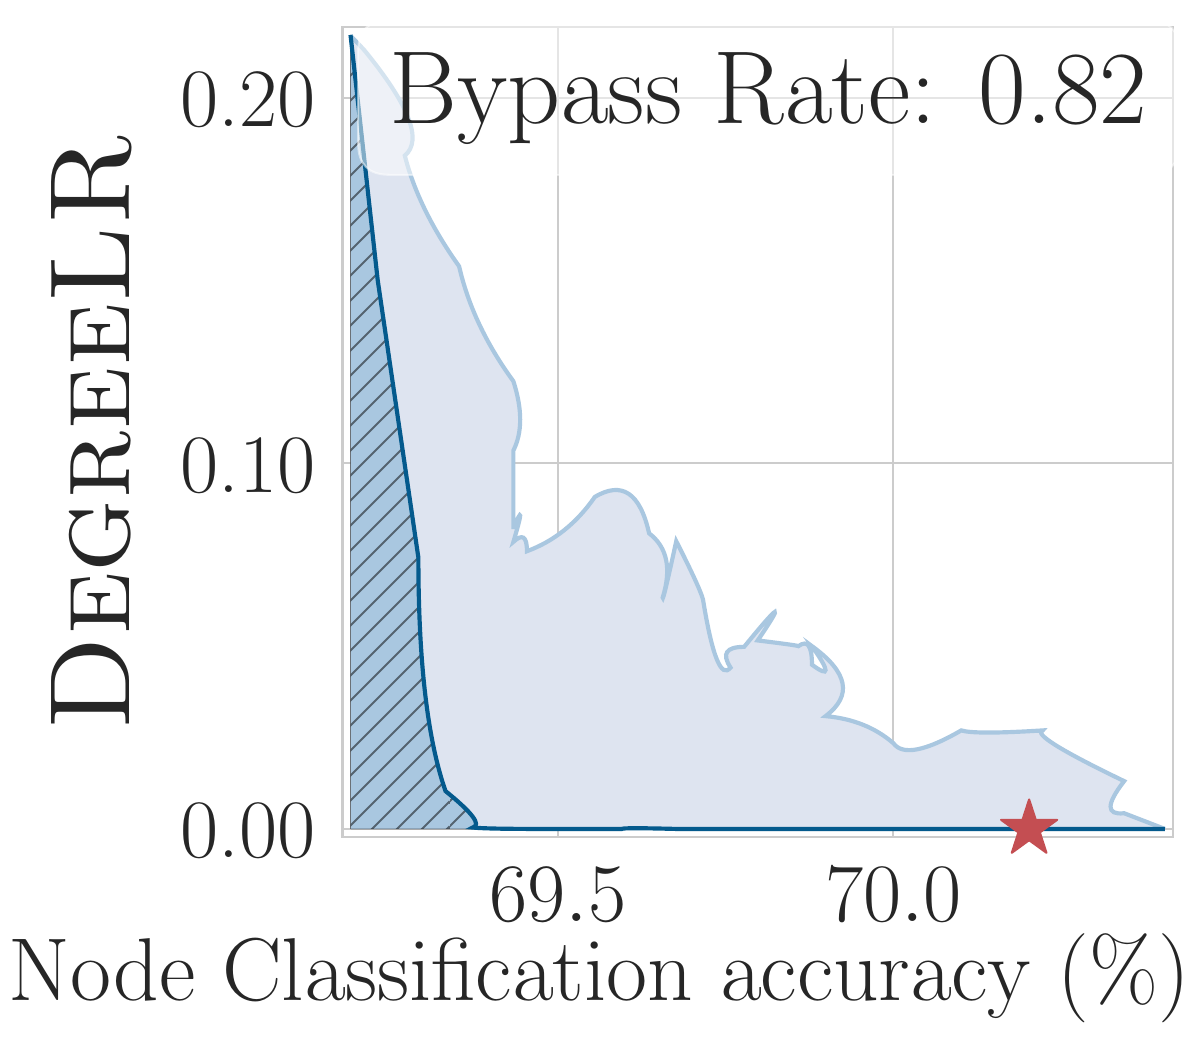} & 
        \includegraphics[width=\linewidth]{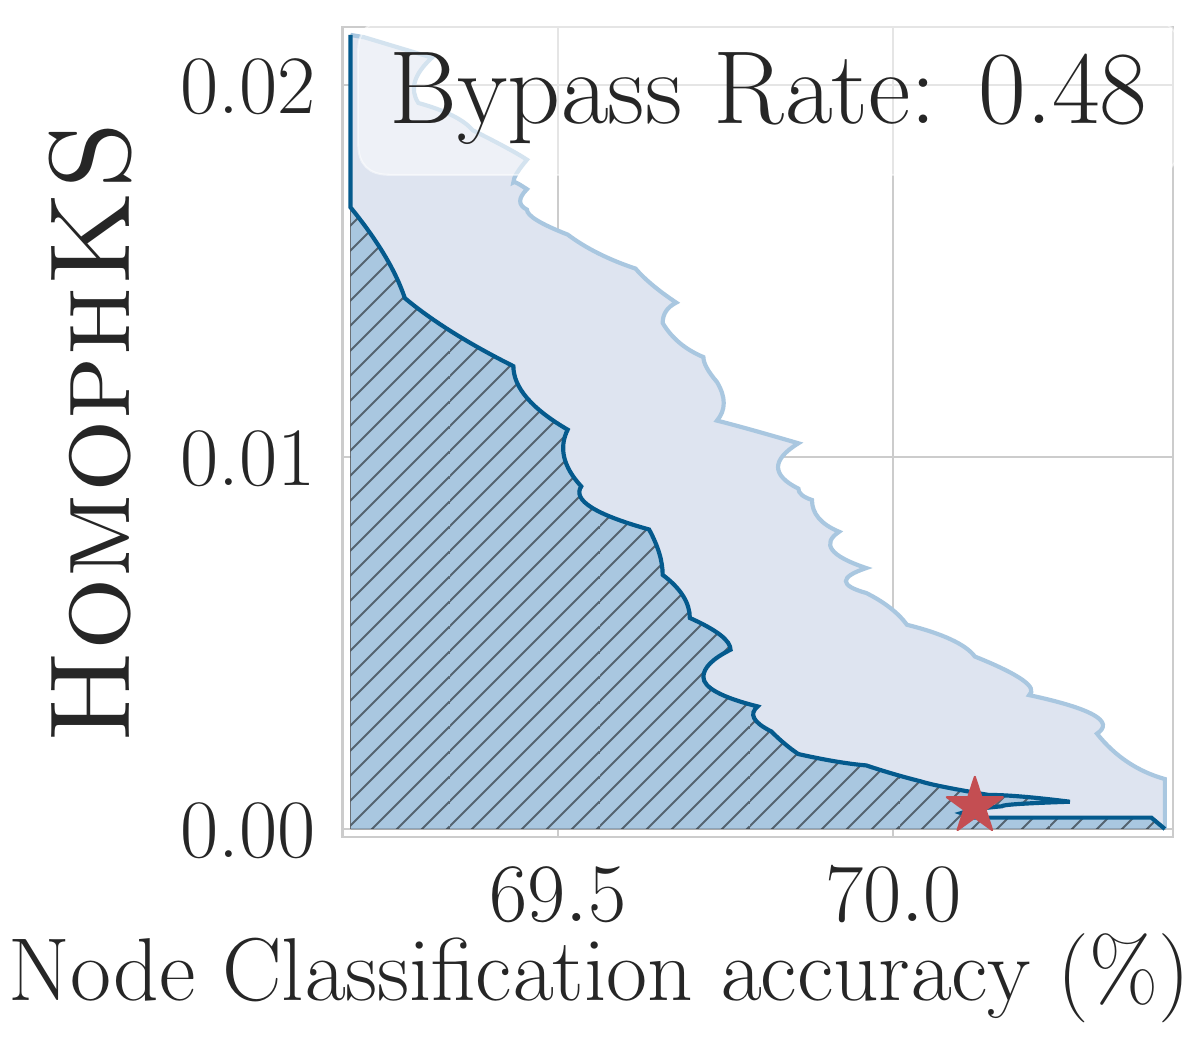} &
        \includegraphics[width=\linewidth]{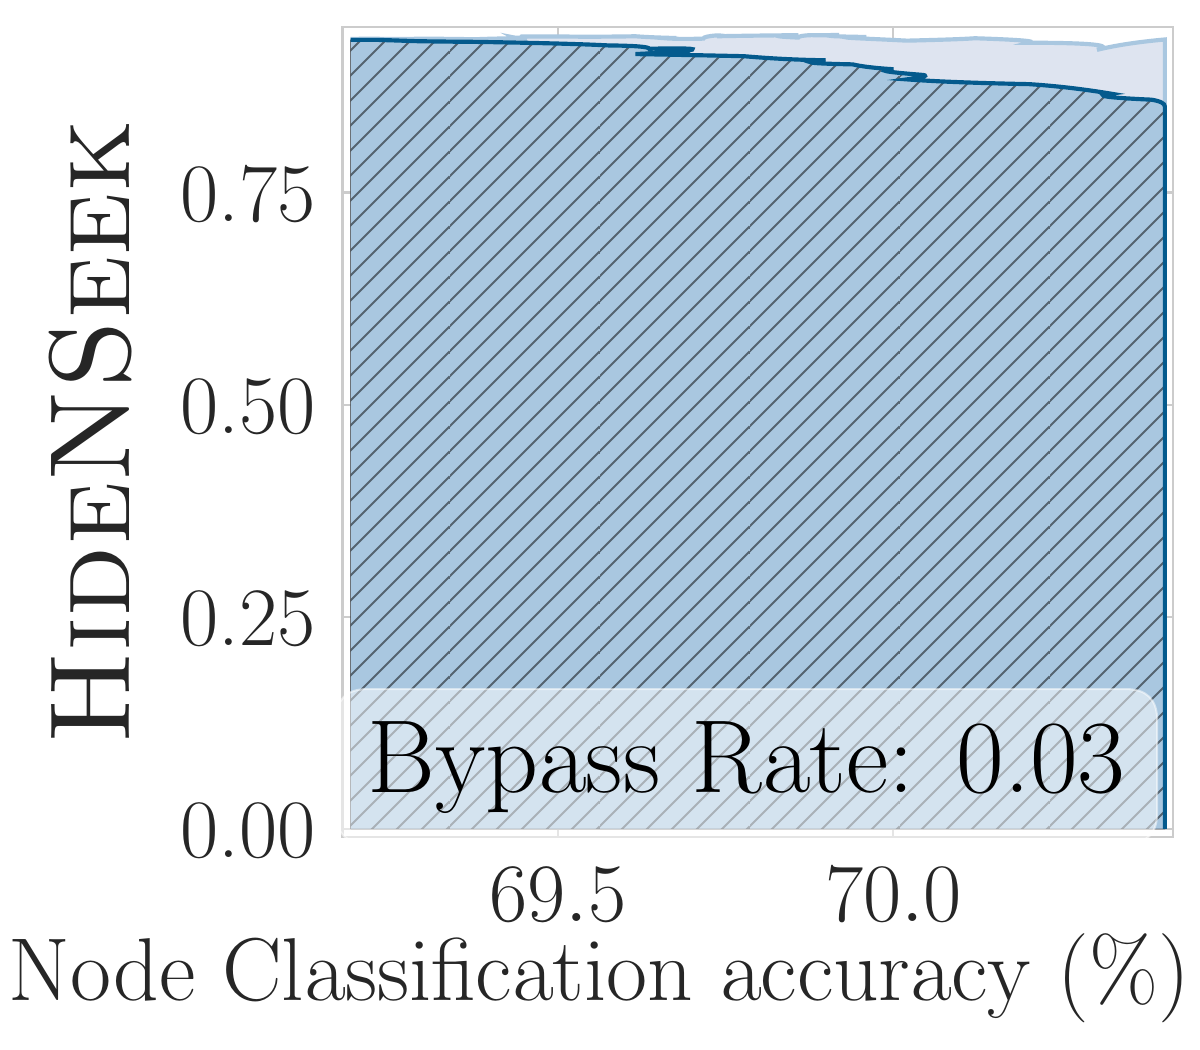} \\
        \hline
        \rotatebox[origin=c]{90}{\coraml} & 
        \includegraphics[width=\linewidth]{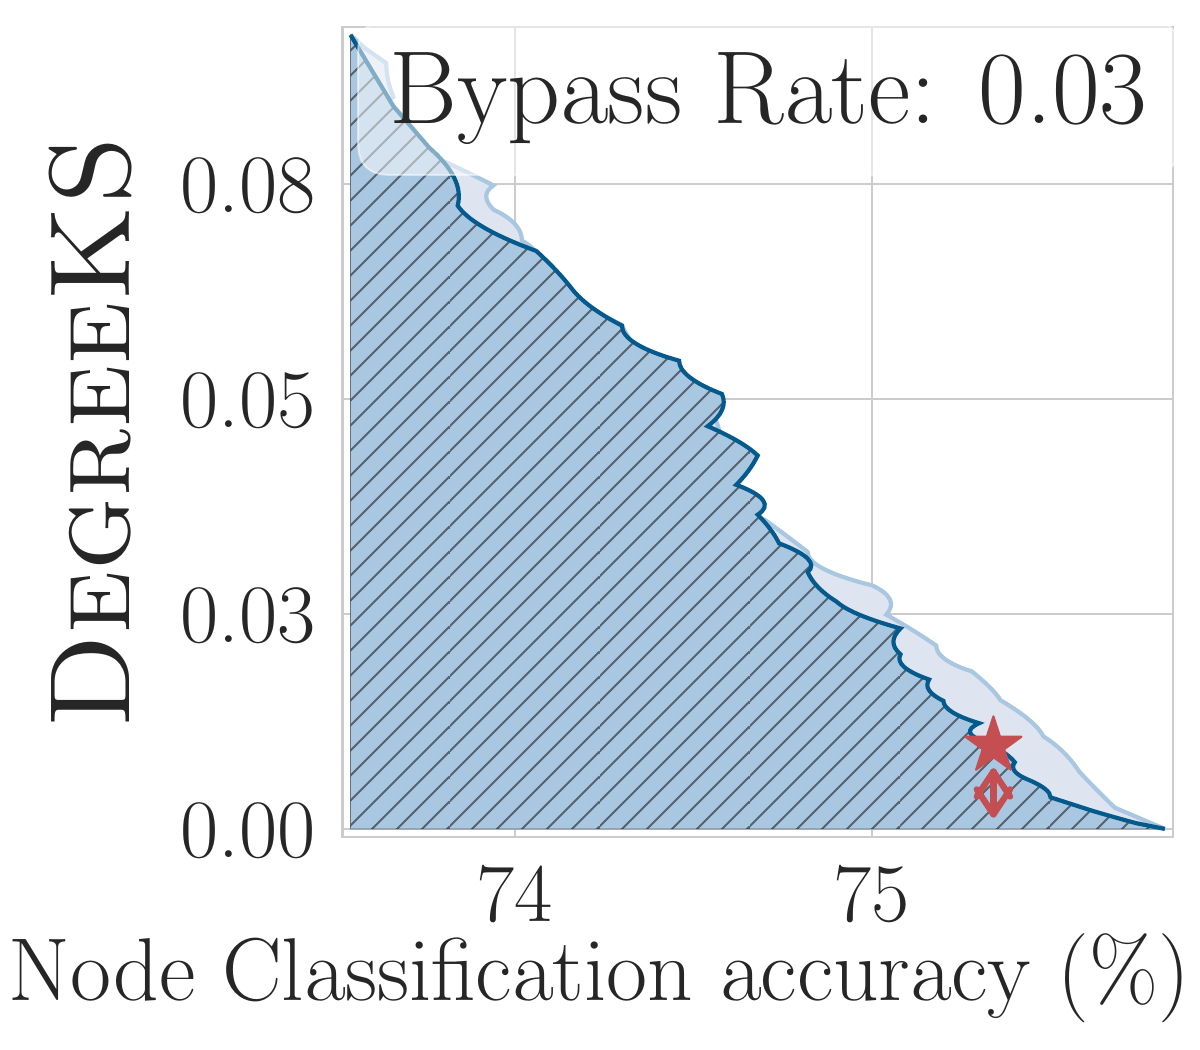} & 
        \includegraphics[width=\linewidth]{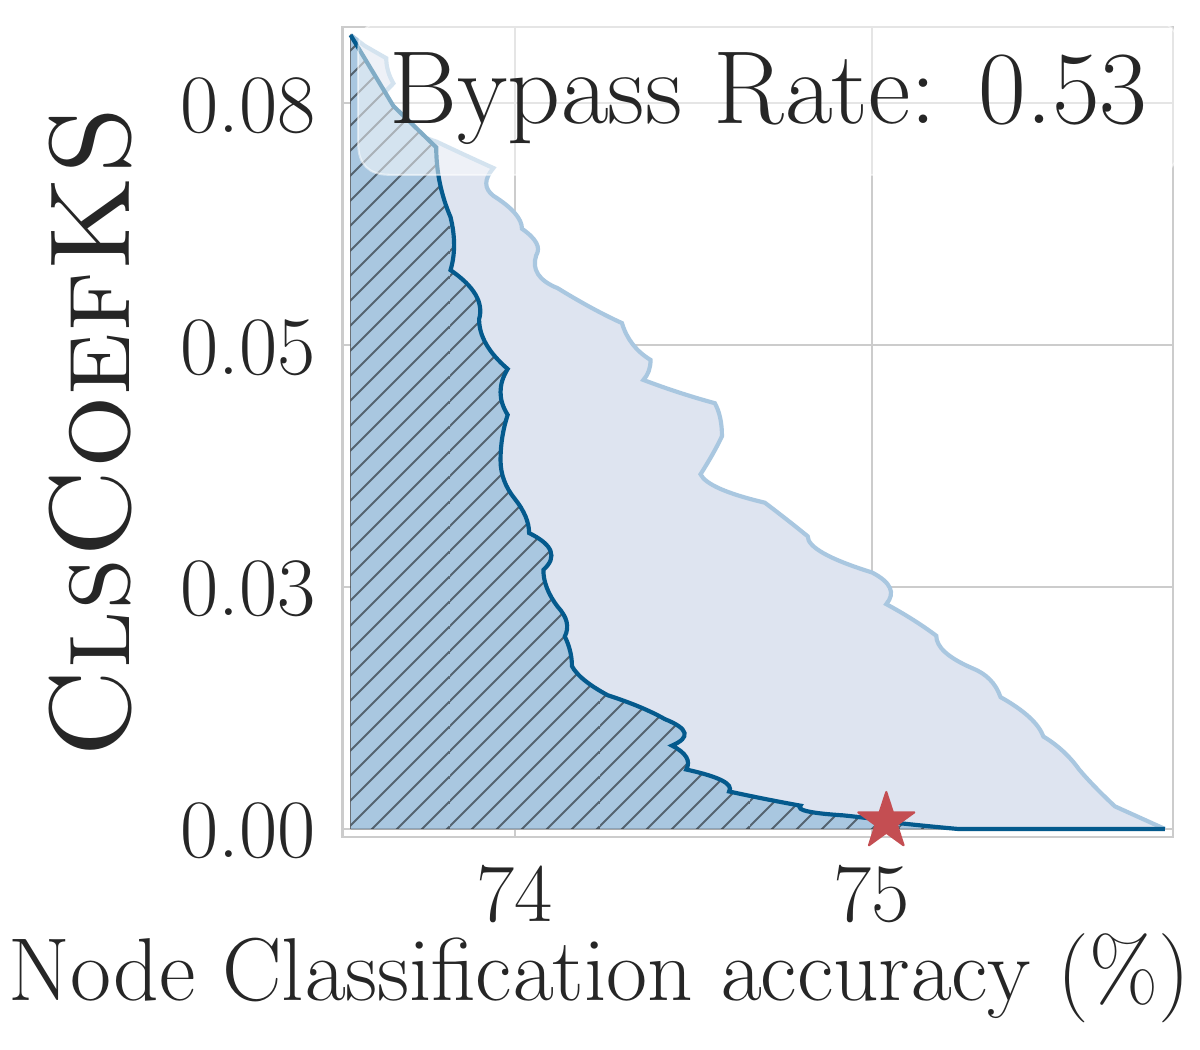} & 
        \includegraphics[width=\linewidth]{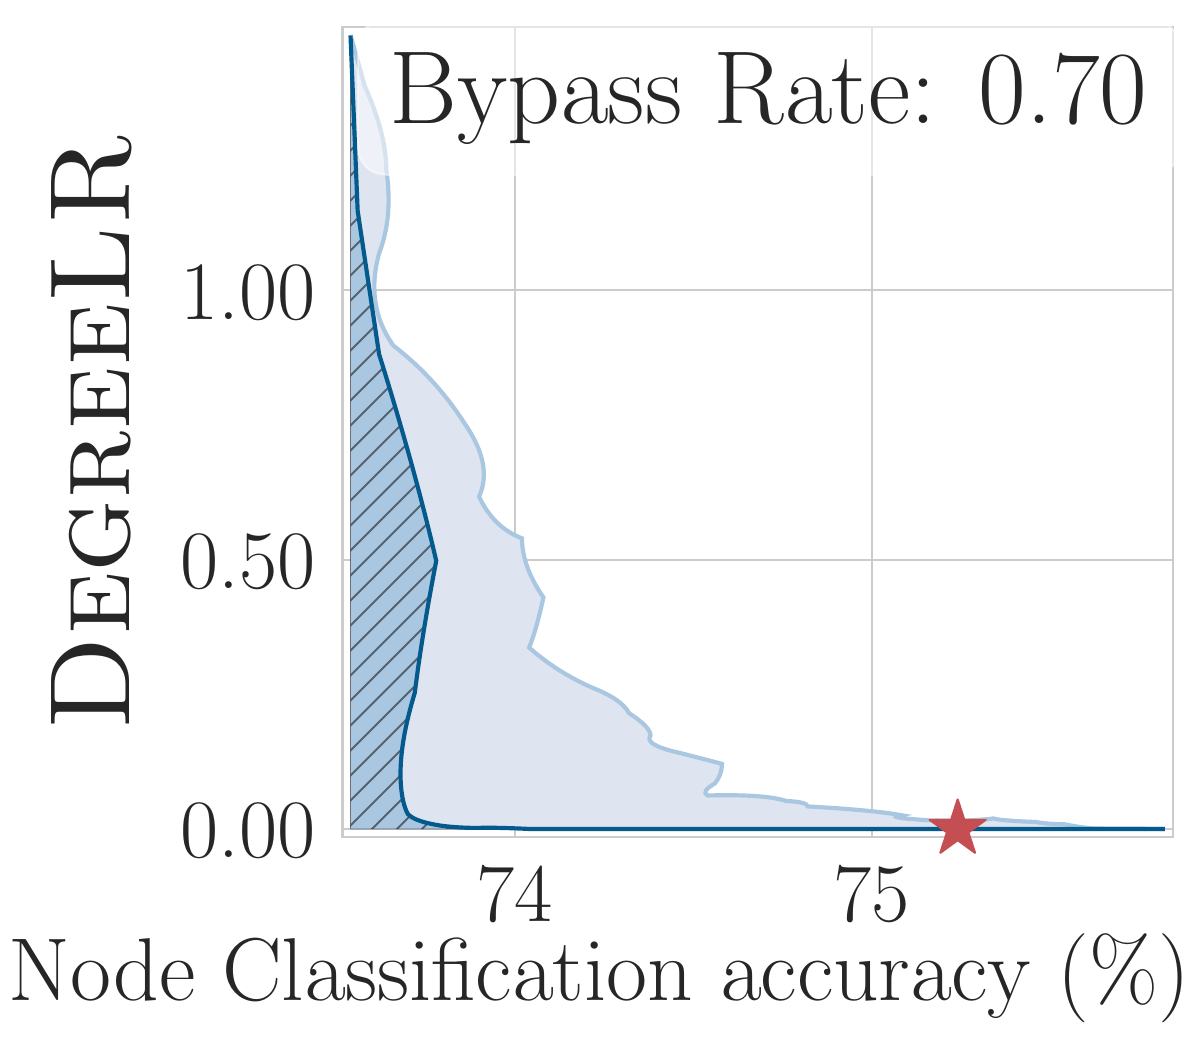} & 
        \includegraphics[width=\linewidth]{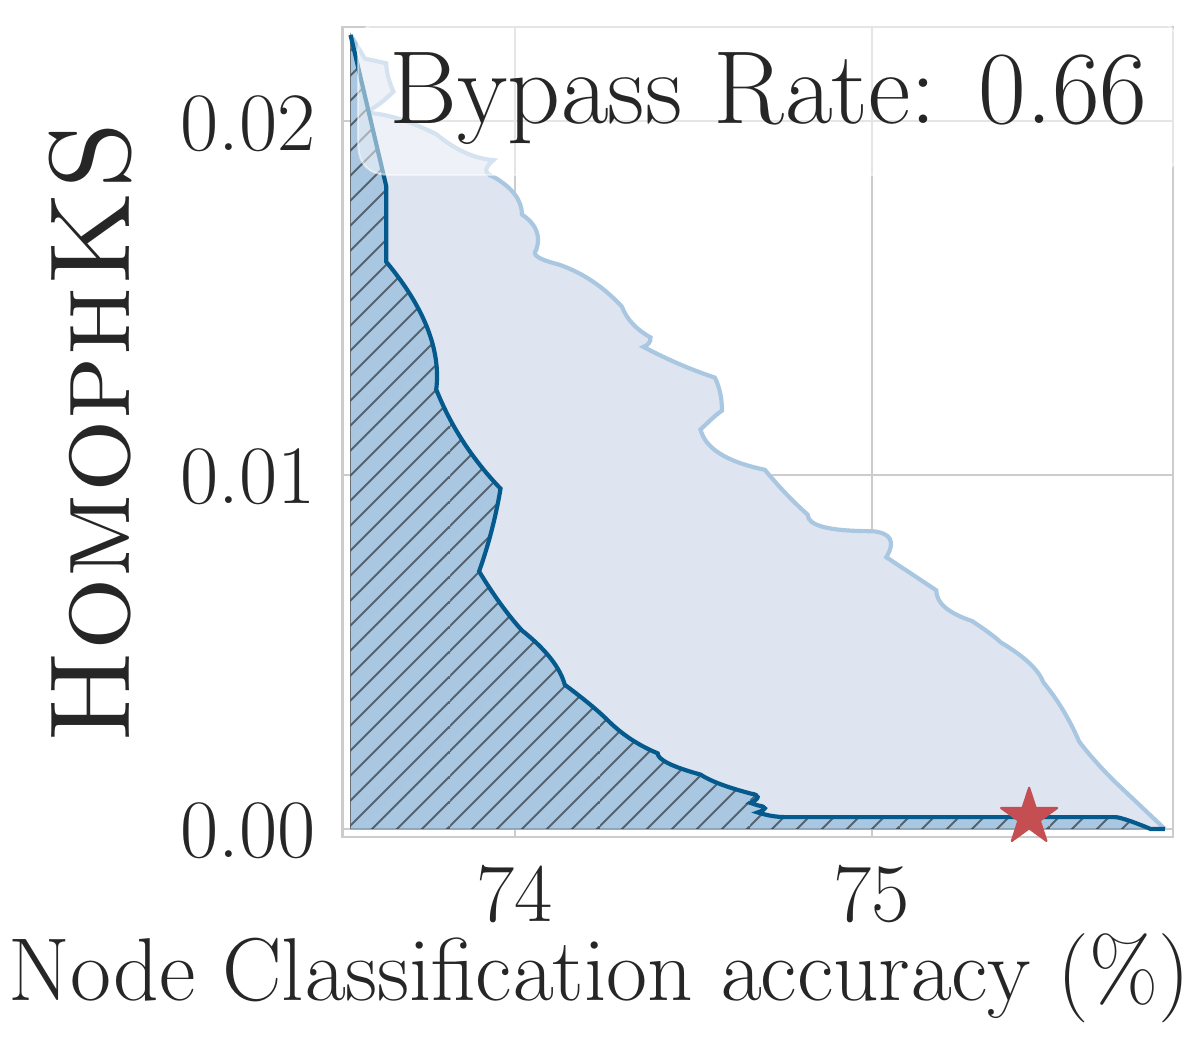} &
        \includegraphics[width=\linewidth]{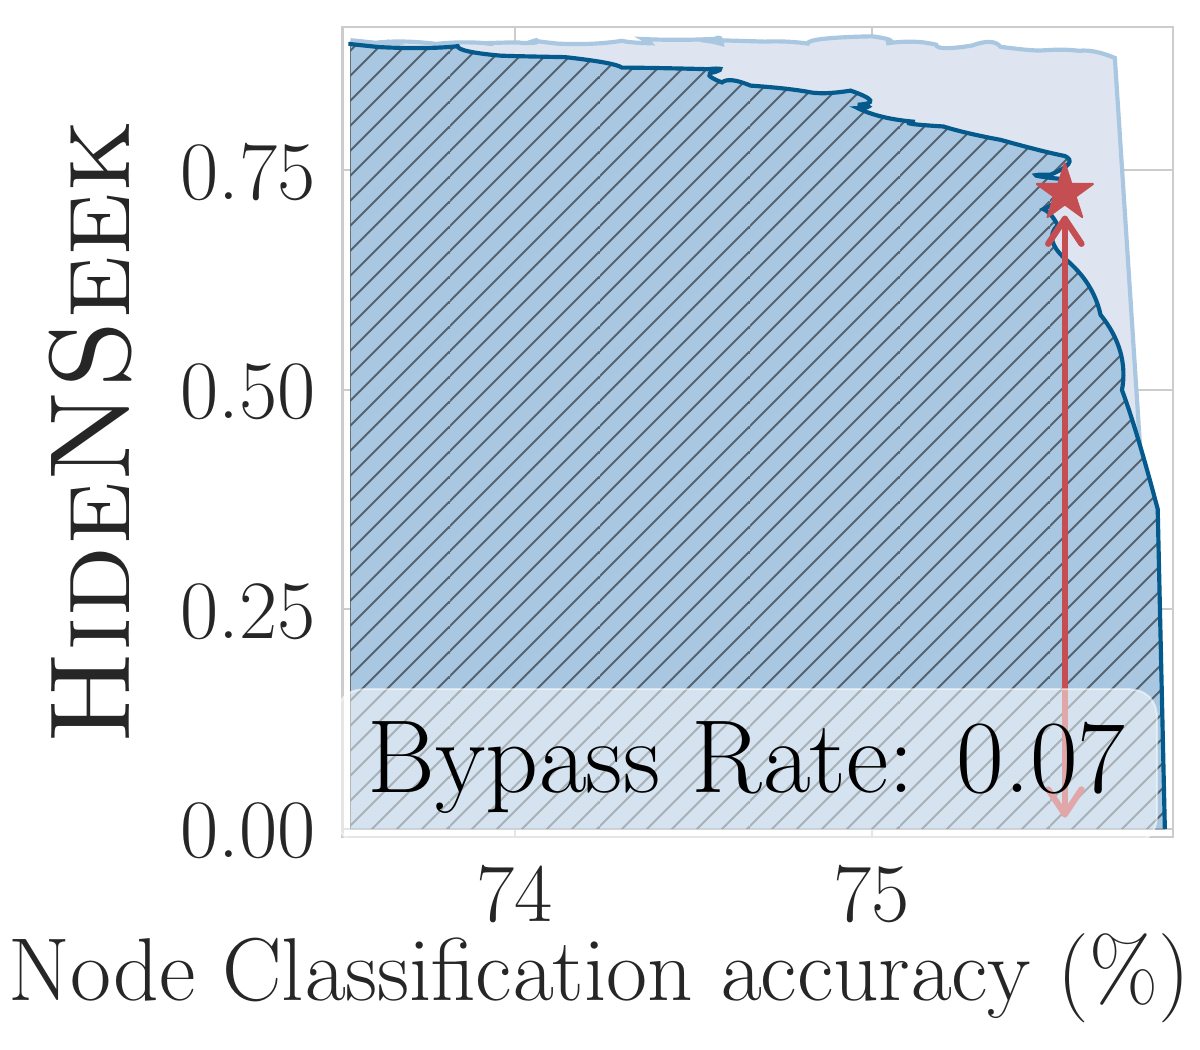} \\
        \hline
        \rotatebox[origin=c]{90}{\lastfmasia} & 
        \includegraphics[width=\linewidth]{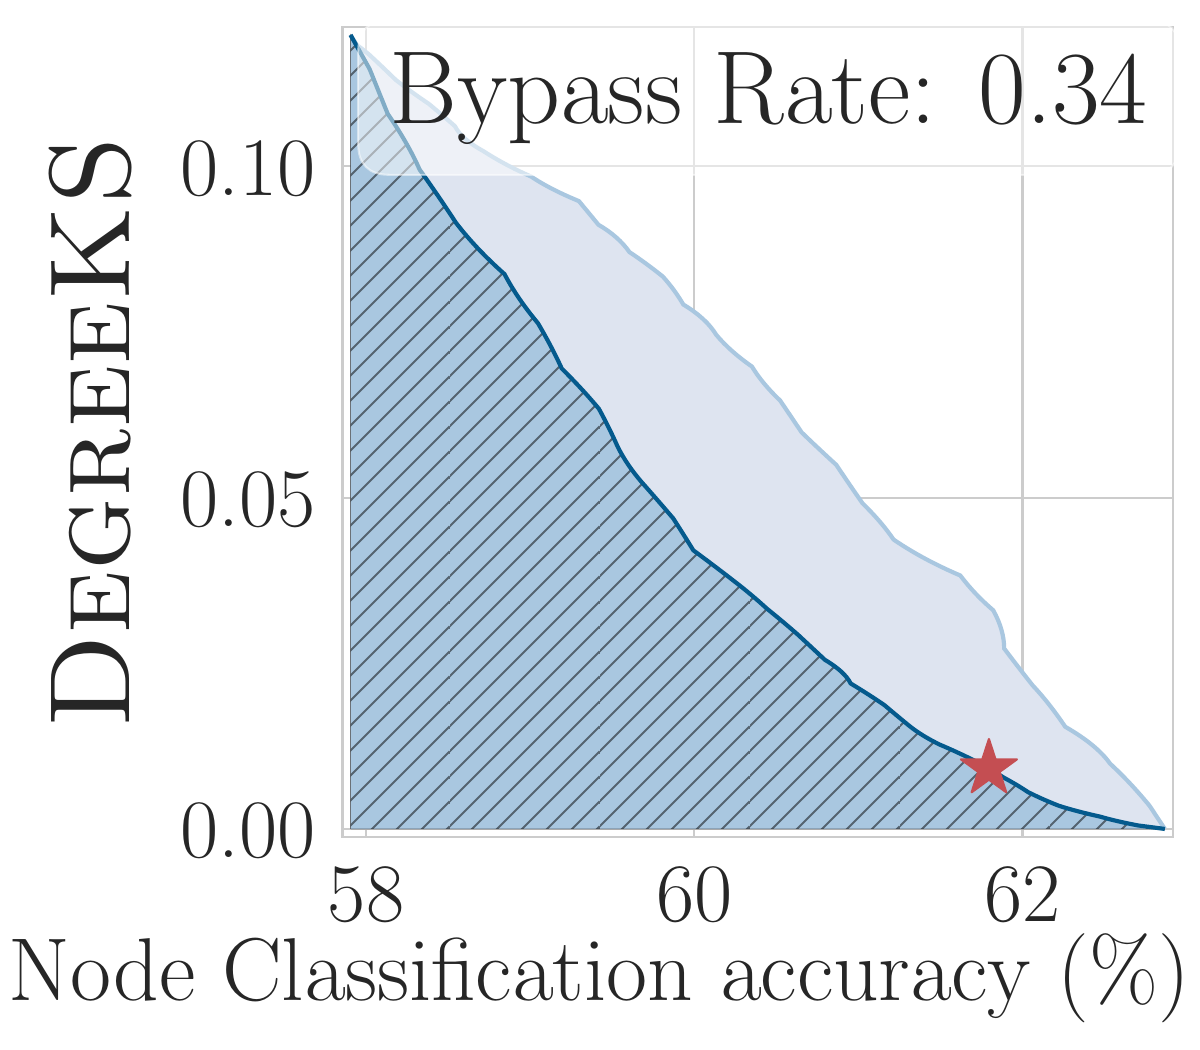} & 
        \includegraphics[width=\linewidth]{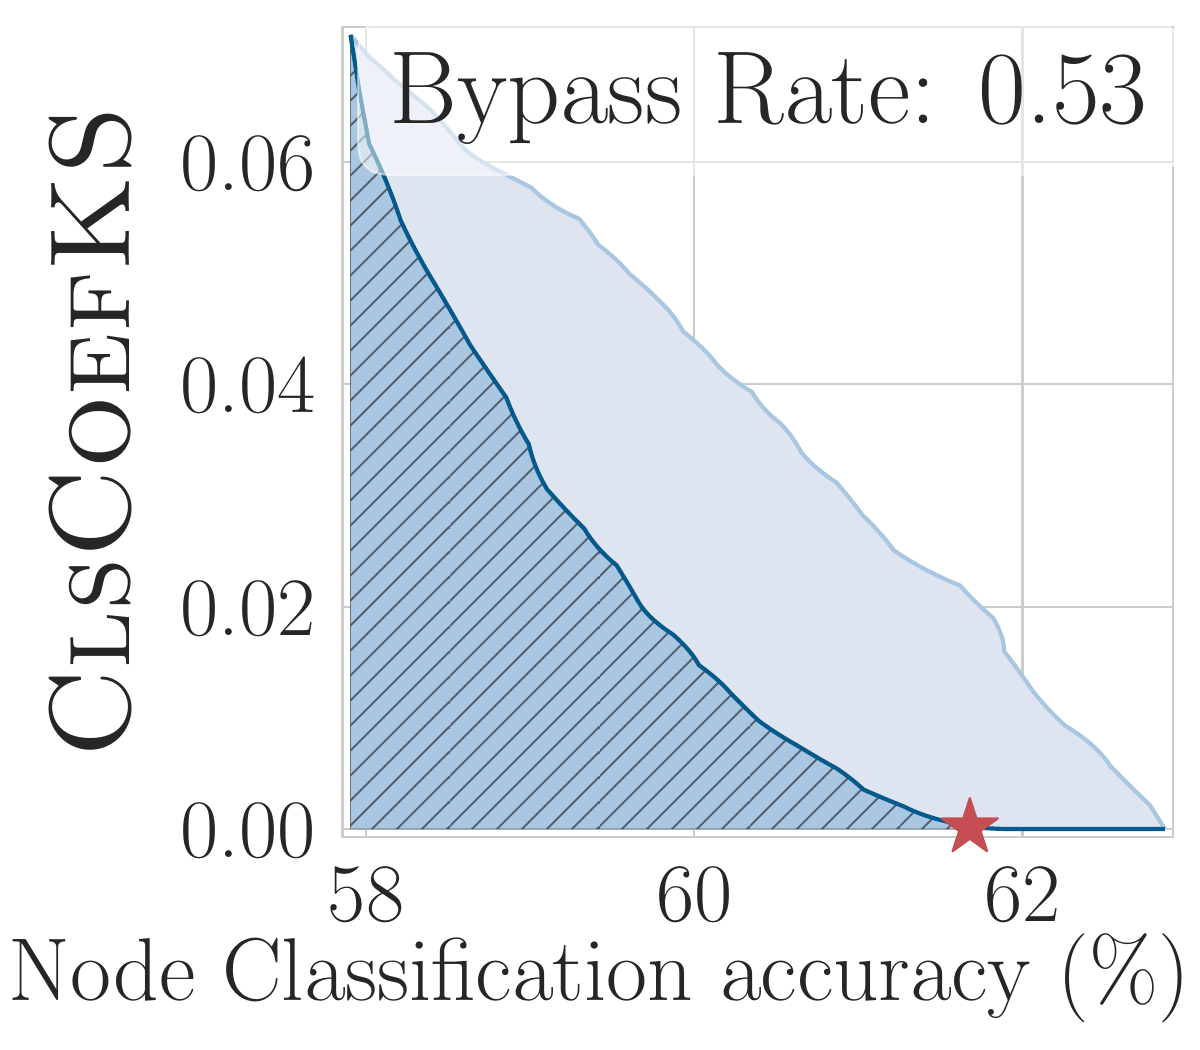} & 
        \includegraphics[width=\linewidth]{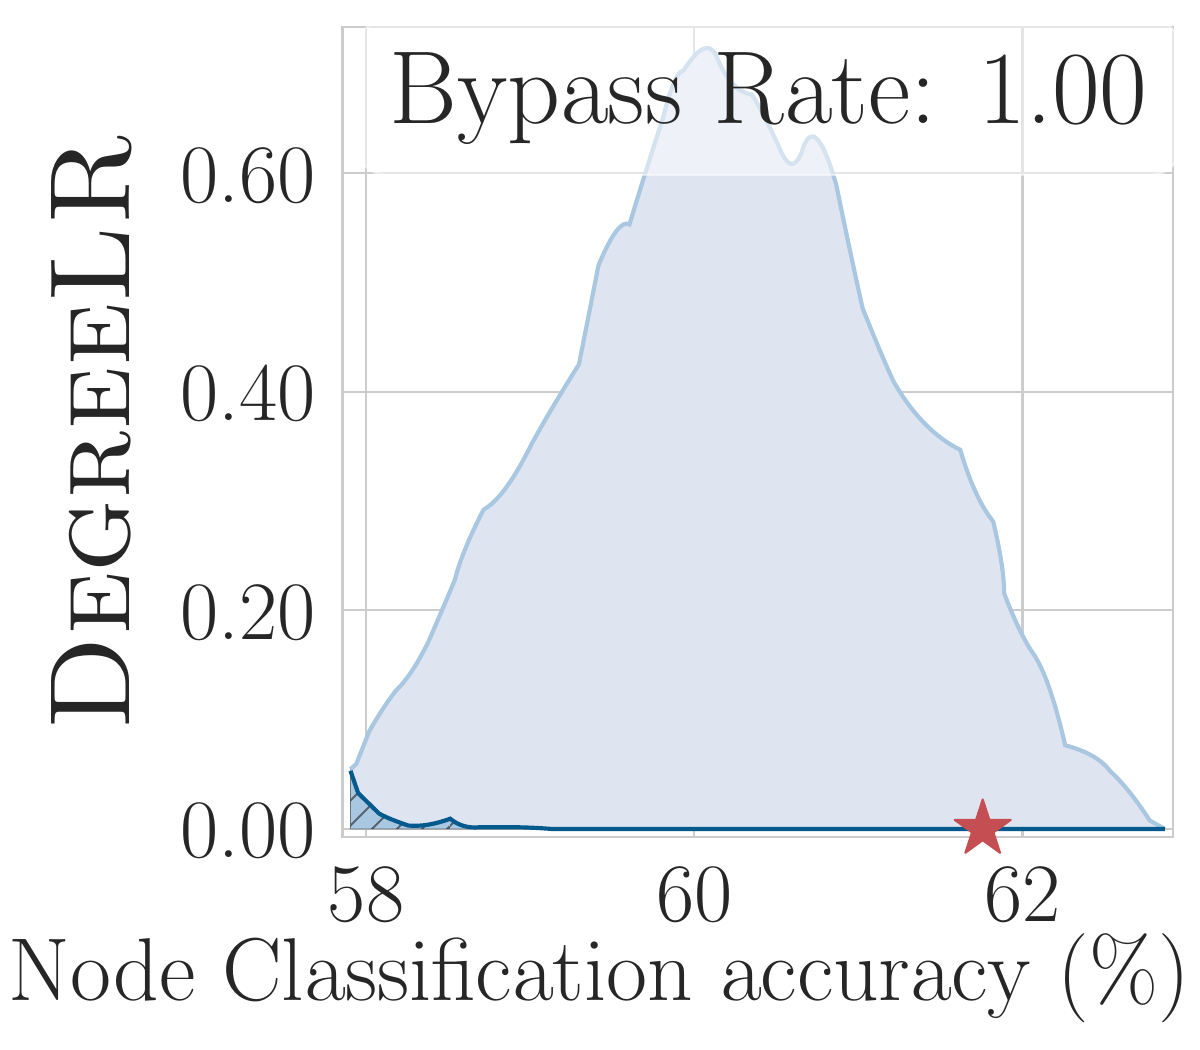} & 
        \includegraphics[width=\linewidth]{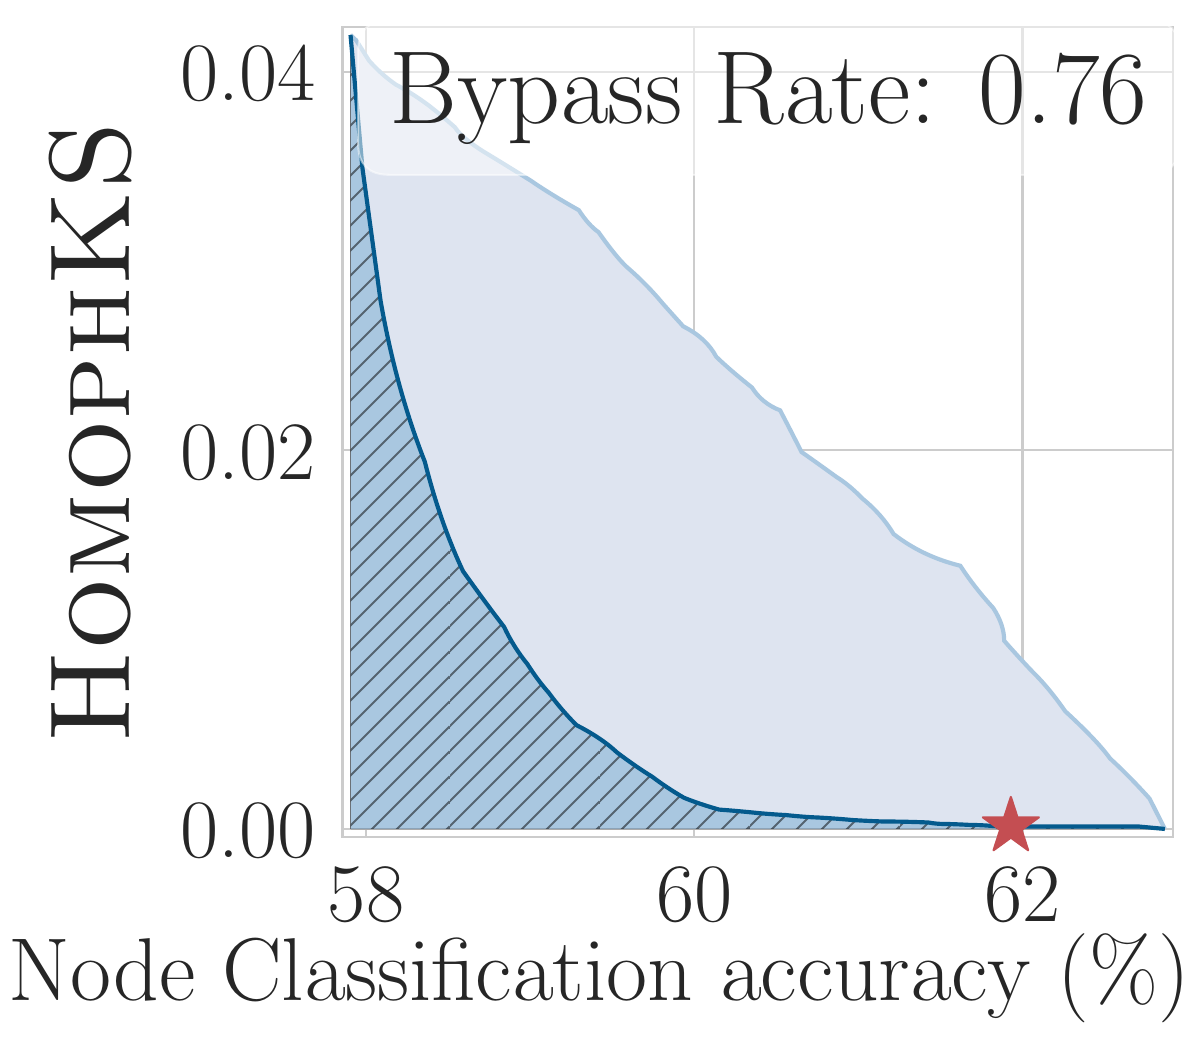} &
        \includegraphics[width=\linewidth]{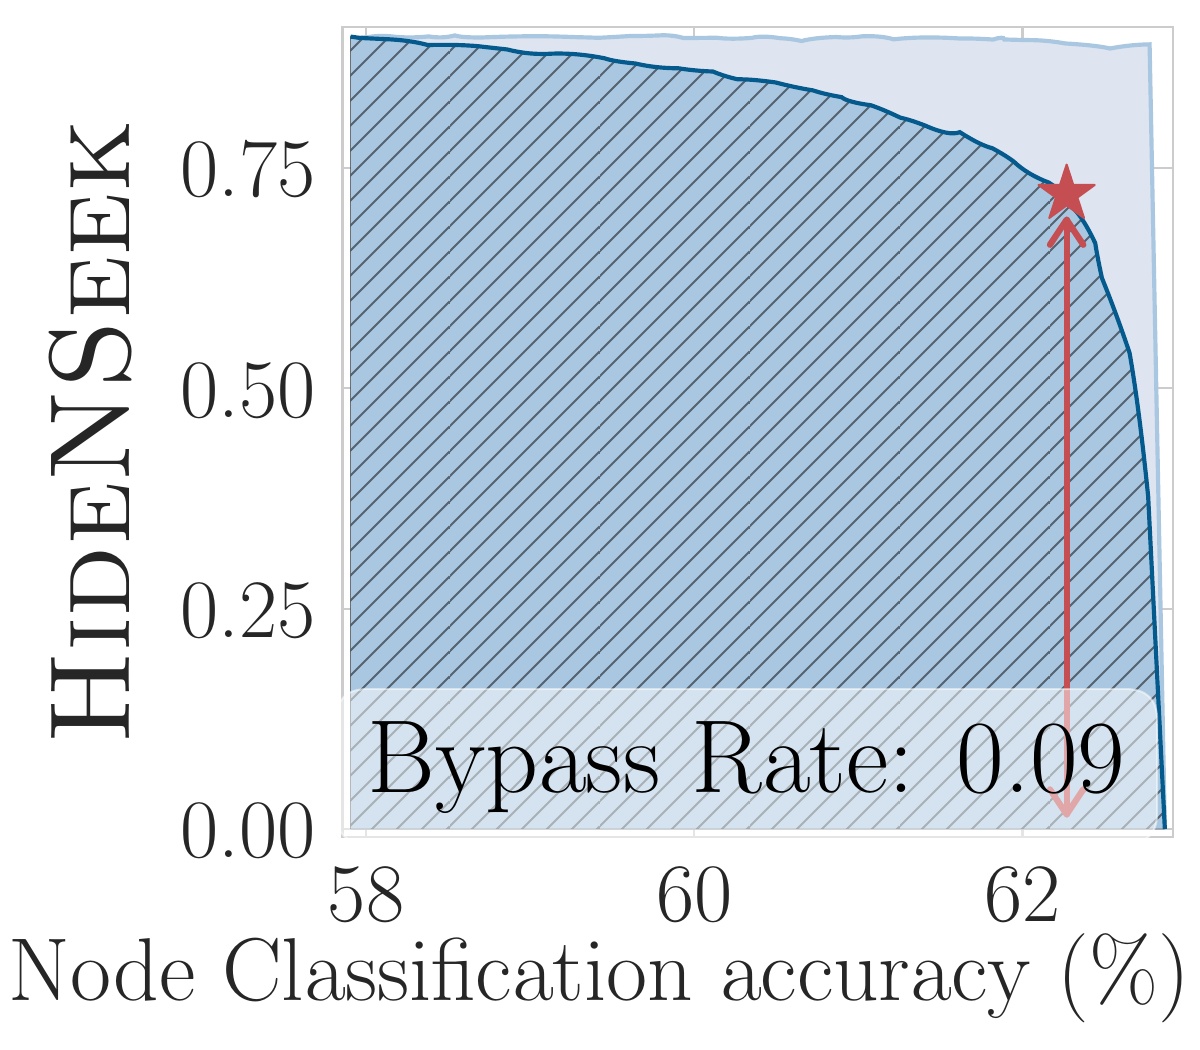} \\
        \hline
        % \rotatebox[origin=c]{90}{\chameleon} & 
        % \includegraphics[width=\linewidth]{FIG/EXP/chameleon/chameleon_random_degree_q2.pdf} & 
        % \includegraphics[width=\linewidth]{FIG/EXP/chameleon/chameleon_random_lc_q2.pdf} & 
        % \includegraphics[width=\linewidth]{FIG/EXP/chameleon/chameleon_random_llr_q2.pdf} & 
        % \includegraphics[width=\linewidth]{FIG/EXP/chameleon/chameleon_random_homophily_q2.pdf} &
        % \includegraphics[width=\linewidth]{FIG/EXP/chameleon/chameleon_random_our_q2.pdf} \\
        % \hline
        % \rotatebox[origin=c]{90}{\squirrel} & 
        % \includegraphics[width=\linewidth]{FIG/EXP/squirrel/squirrel_random_degree_q2.pdf} & 
        % \includegraphics[width=\linewidth]{FIG/EXP/squirrel/squirrel_random_lc_q2.pdf} & 
        % \includegraphics[width=\linewidth]{FIG/EXP/squirrel/squirrel_random_llr_q2.pdf} & 
        % \includegraphics[width=\linewidth]{FIG/EXP/squirrel/squirrel_random_homophily_q2.pdf} &
        % \includegraphics[width=\linewidth]{FIG/EXP/squirrel/squirrel_random_our_q2.pdf} \\
        % \hline
    \end{tabular}
    }
    \label{tab:exp:q2_random}
\end{table*}

\newcolumntype{C}{>{\centering\arraybackslash}m{0.15\linewidth}}
\begin{table*}
    \centering
    \caption{The additional experimental results regarding Q2 \& Q3 on \dice.}
    \resizebox{0.8\textwidth}{!}{
    \begin{tabular}{l||C|C|C|C||C}
        \hline
        % & \multicolumn{4}{c||}{Existing Measures} & \multirow{3}{*}{\textbf{\measure}} \\ 
        % \cline{2-5}
        % & Degree Dist. & Clustering Coeff. & Degree Dist. & Homophily Dist. & \\
        % & (KS test) & (KS test) & (LR test)& (KS test) & \\
        & \textsc{DegreeKS} & \textsc{ClsCoefKS} & \textsc{DegreeLR} & \textsc{HomophKS} & \textbf{\measure} \\
        \hline\hline
        \rotatebox[origin=c]{90}{\cora} & 
        \includegraphics[width=\linewidth]{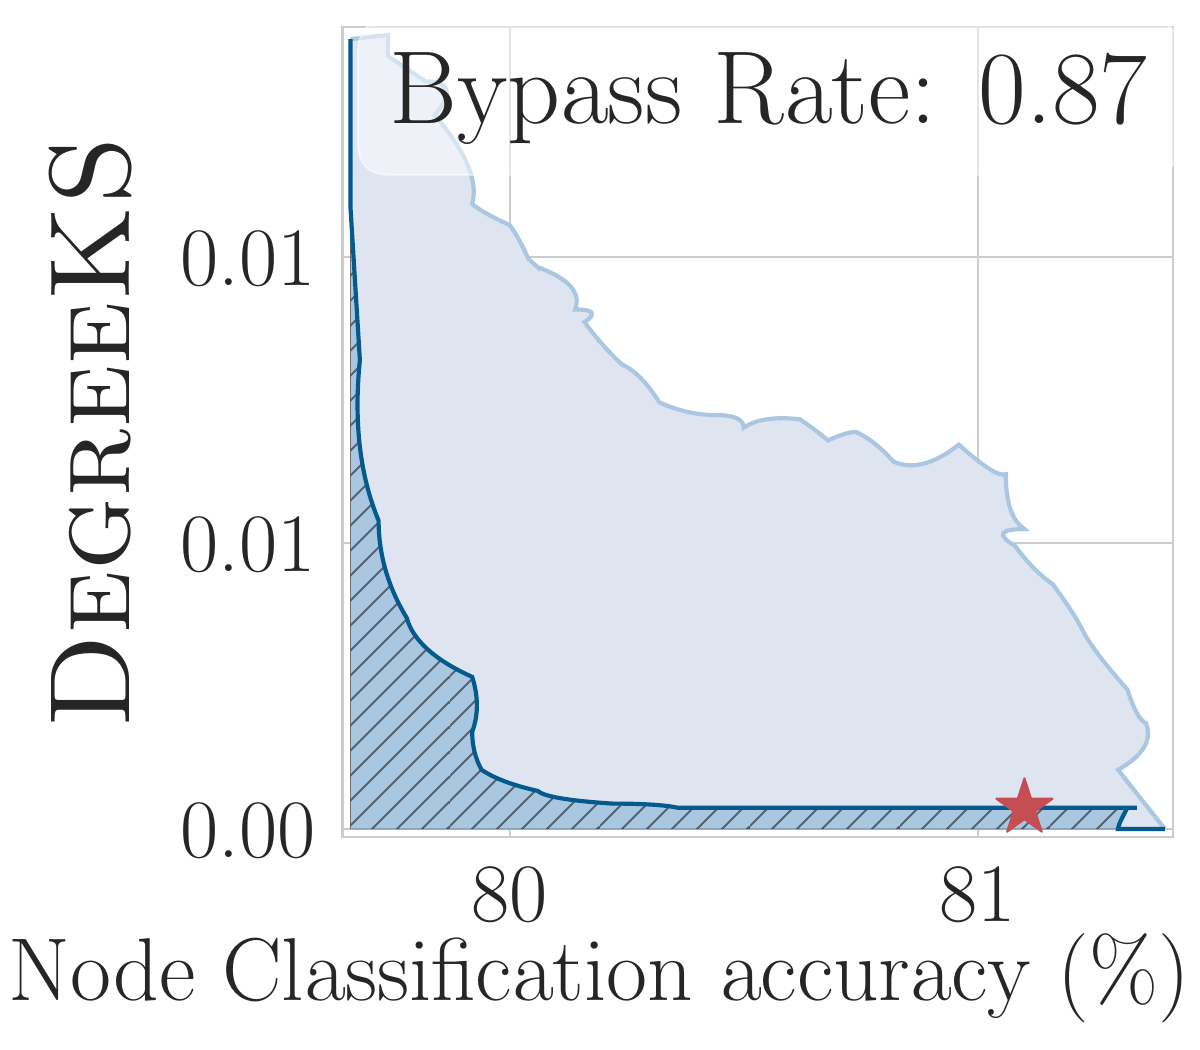} & 
        \includegraphics[width=\linewidth]{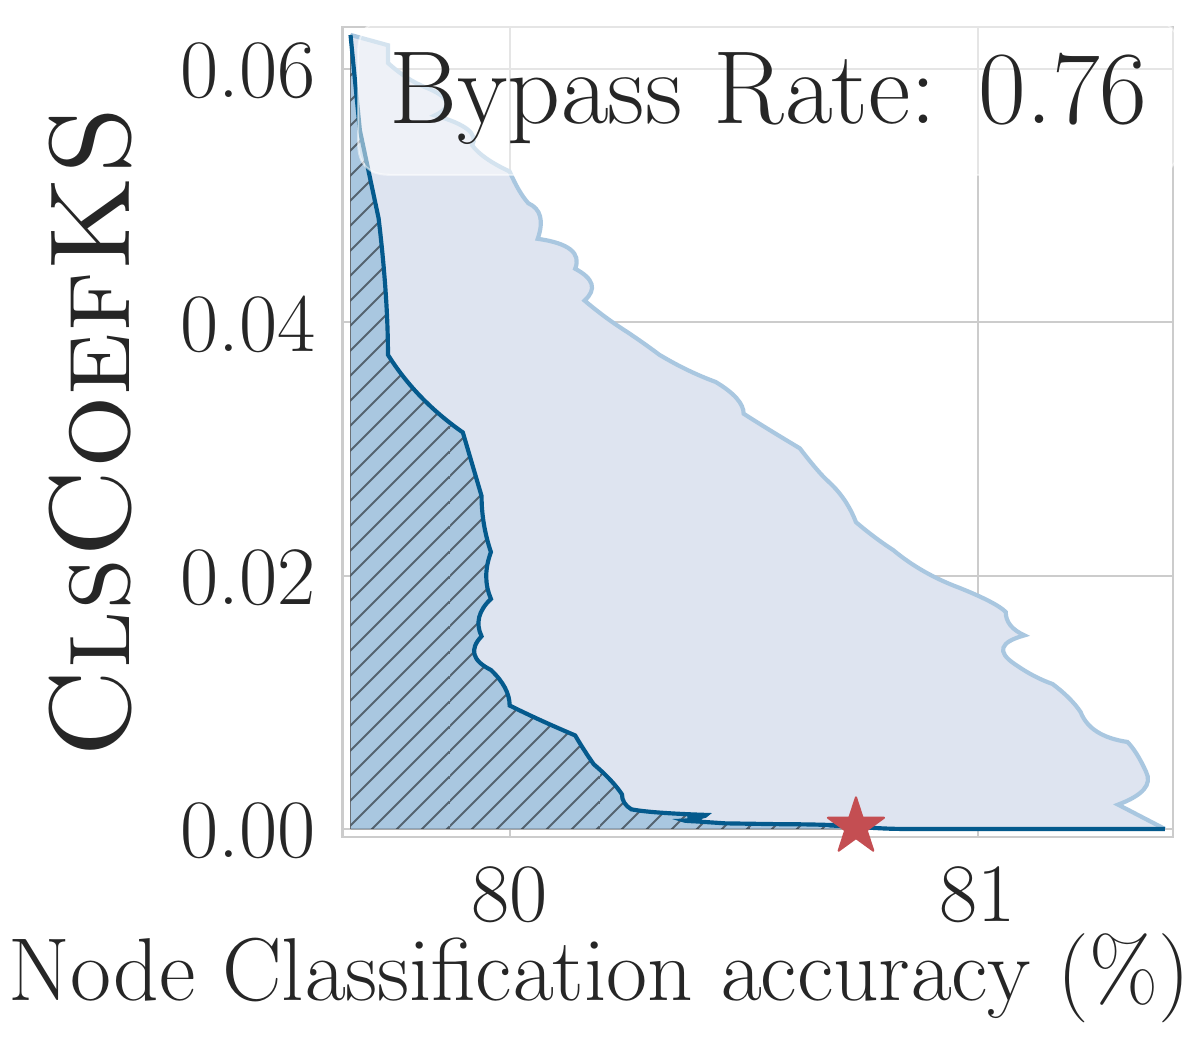} & 
        \includegraphics[width=\linewidth]{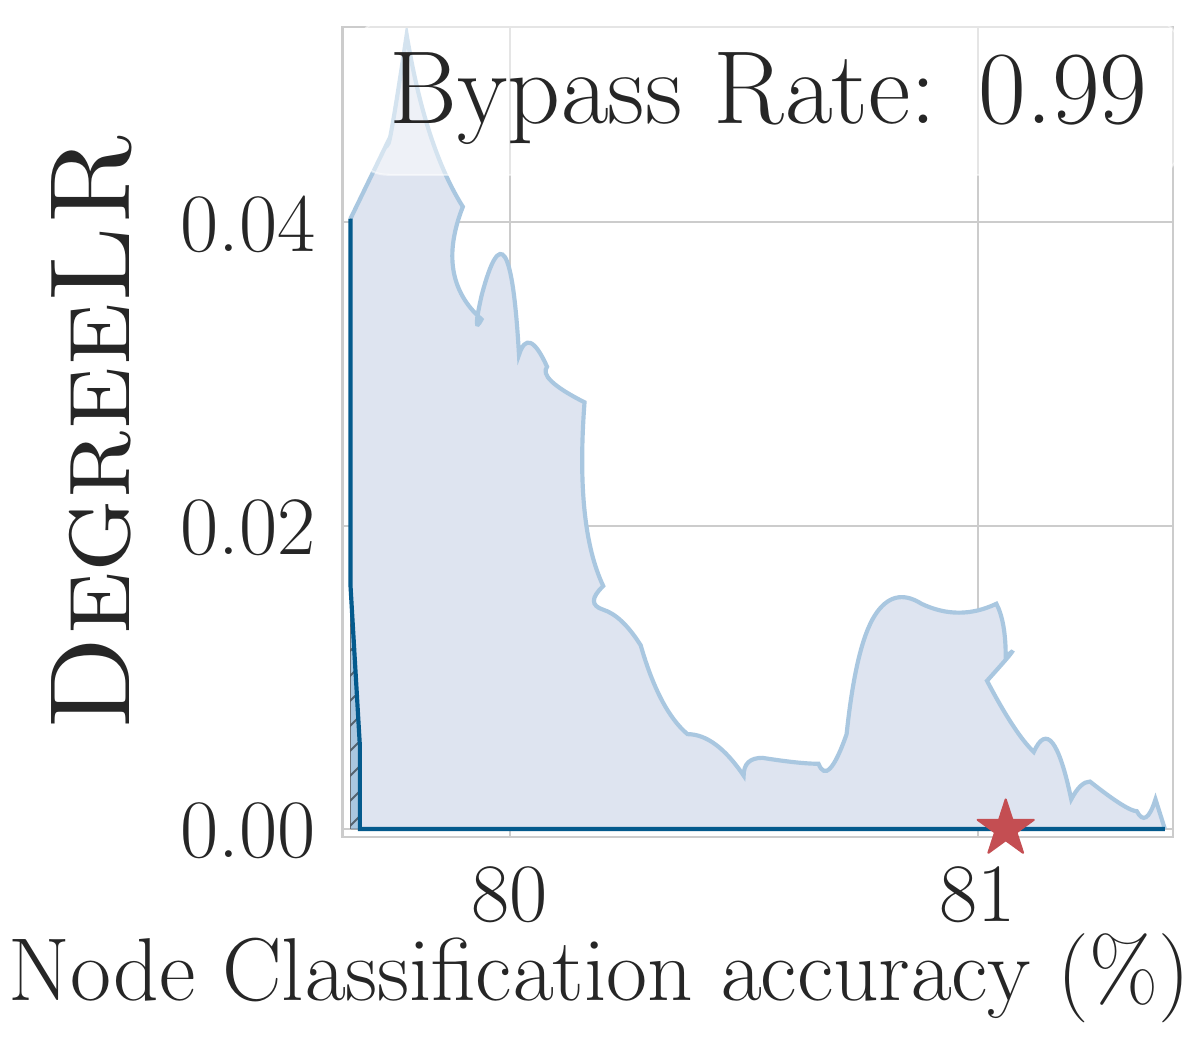} & 
        \includegraphics[width=\linewidth]{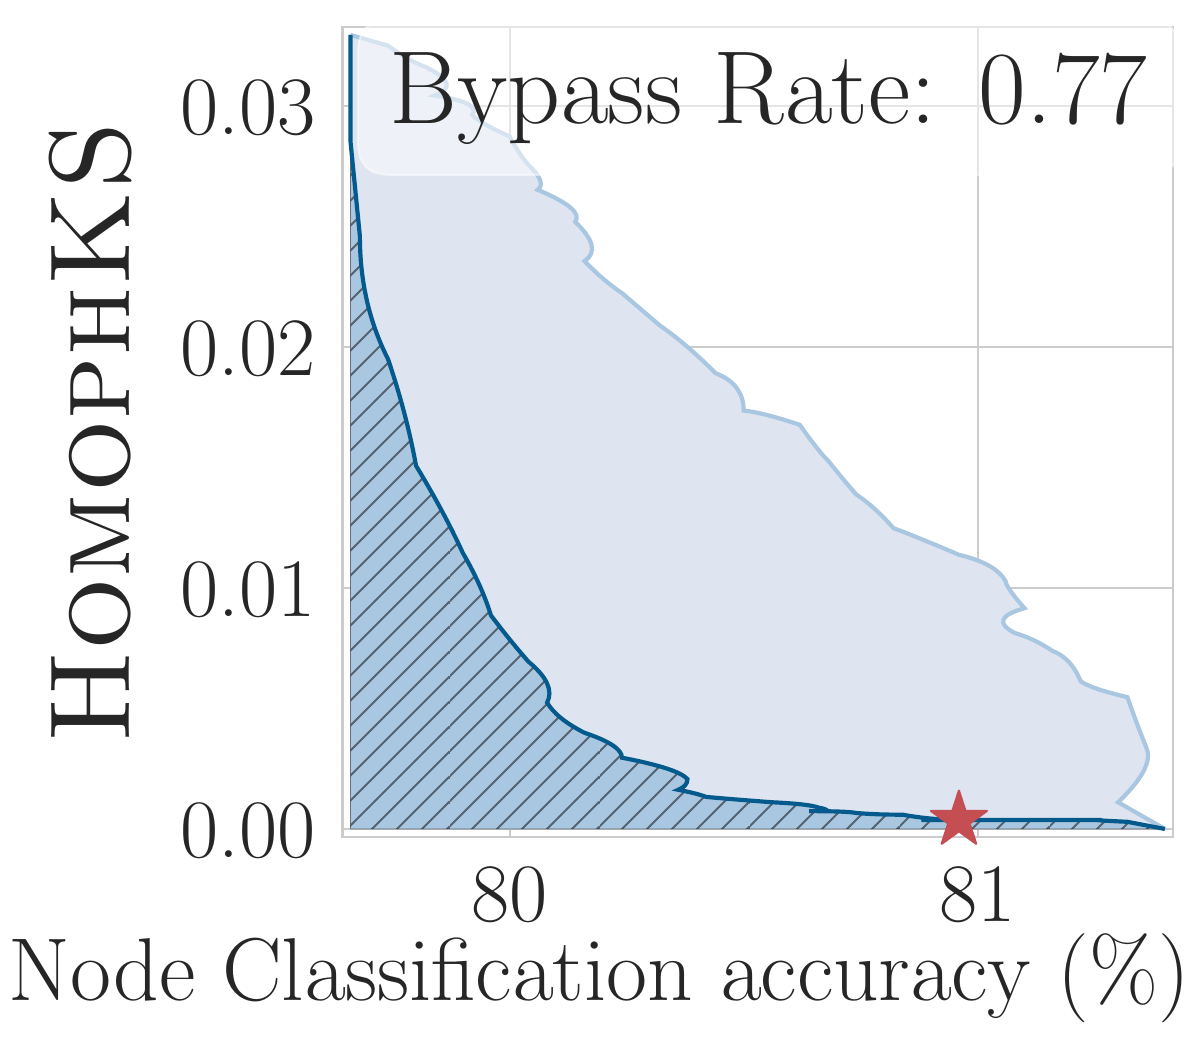} &
        \includegraphics[width=\linewidth]{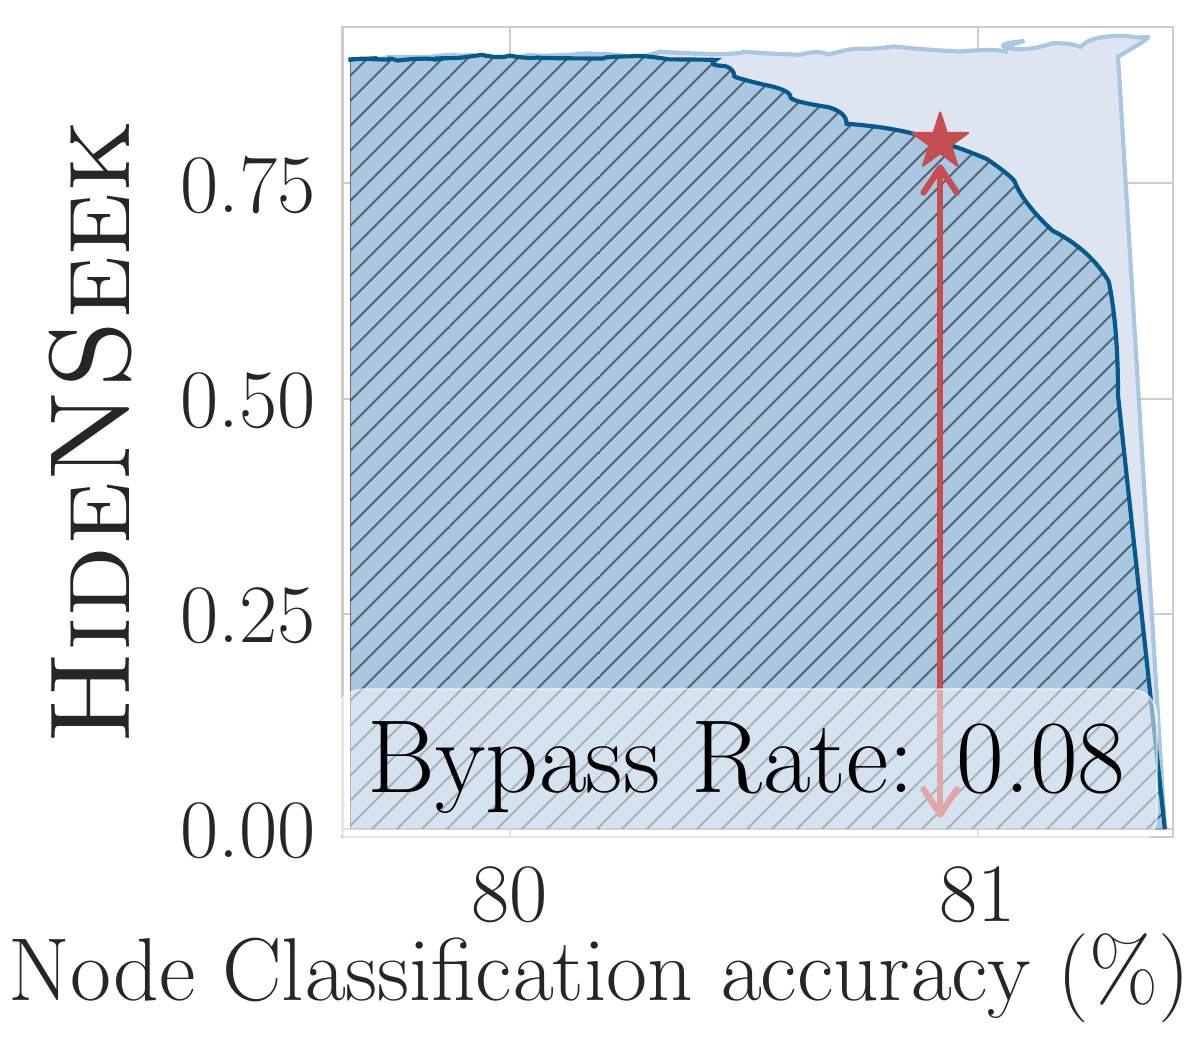} \\
        \hline
        \rotatebox[origin=c]{90}{\citeseer} & 
        \includegraphics[width=\linewidth]{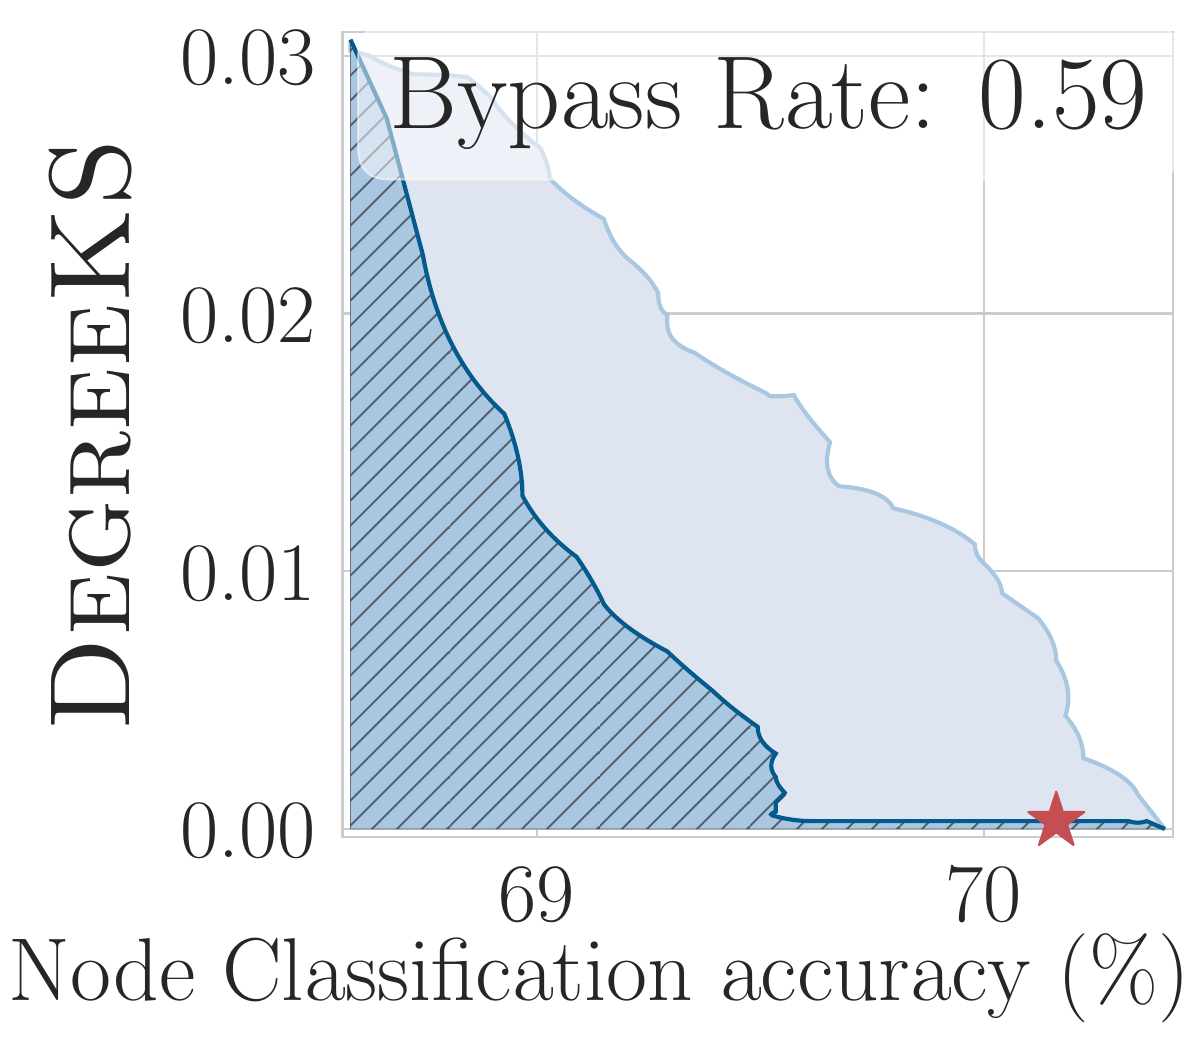} & 
        \includegraphics[width=\linewidth]{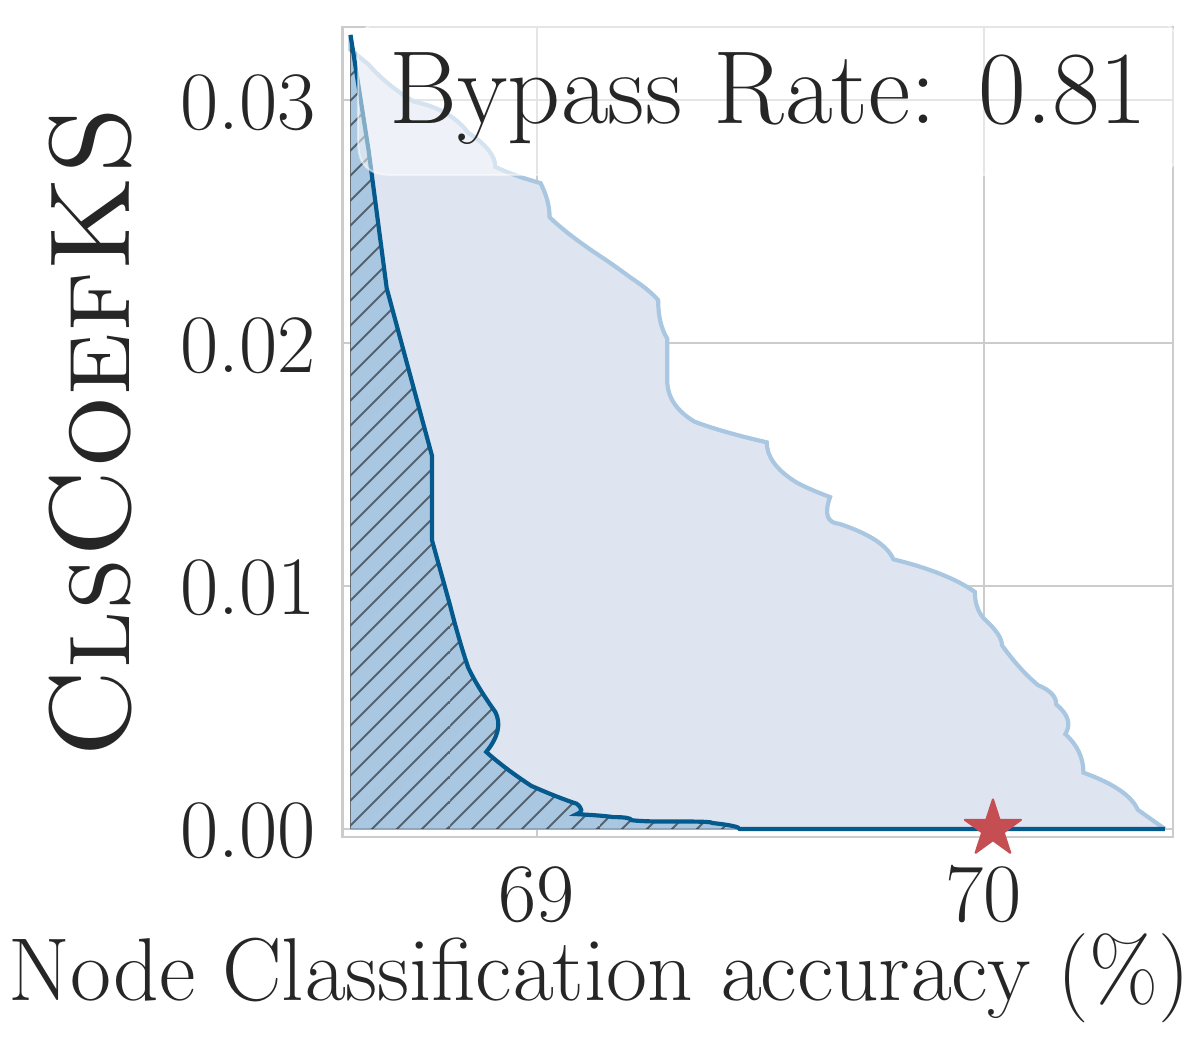} & 
        \includegraphics[width=\linewidth]{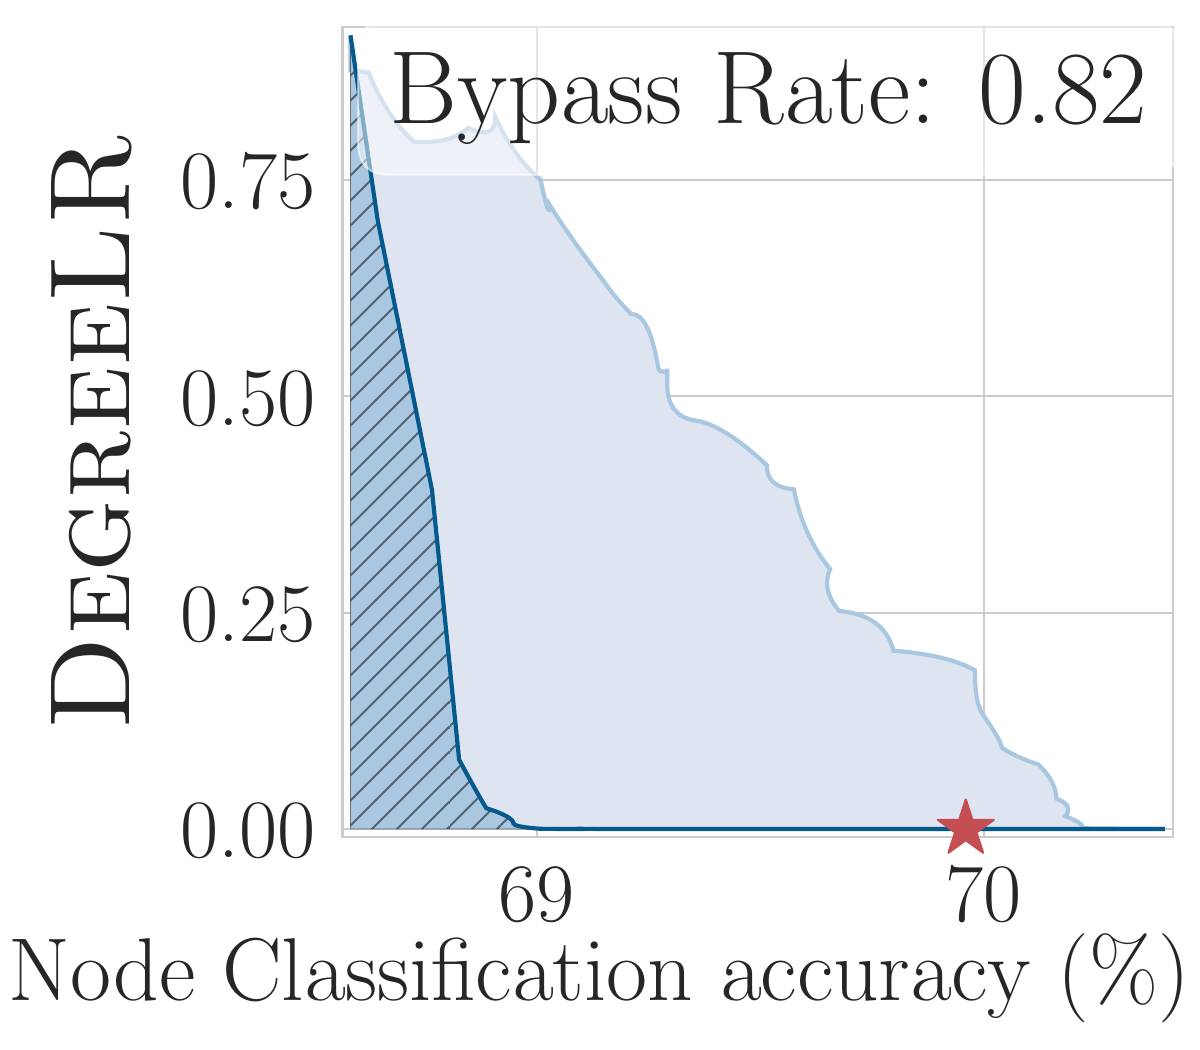} & 
        \includegraphics[width=\linewidth]{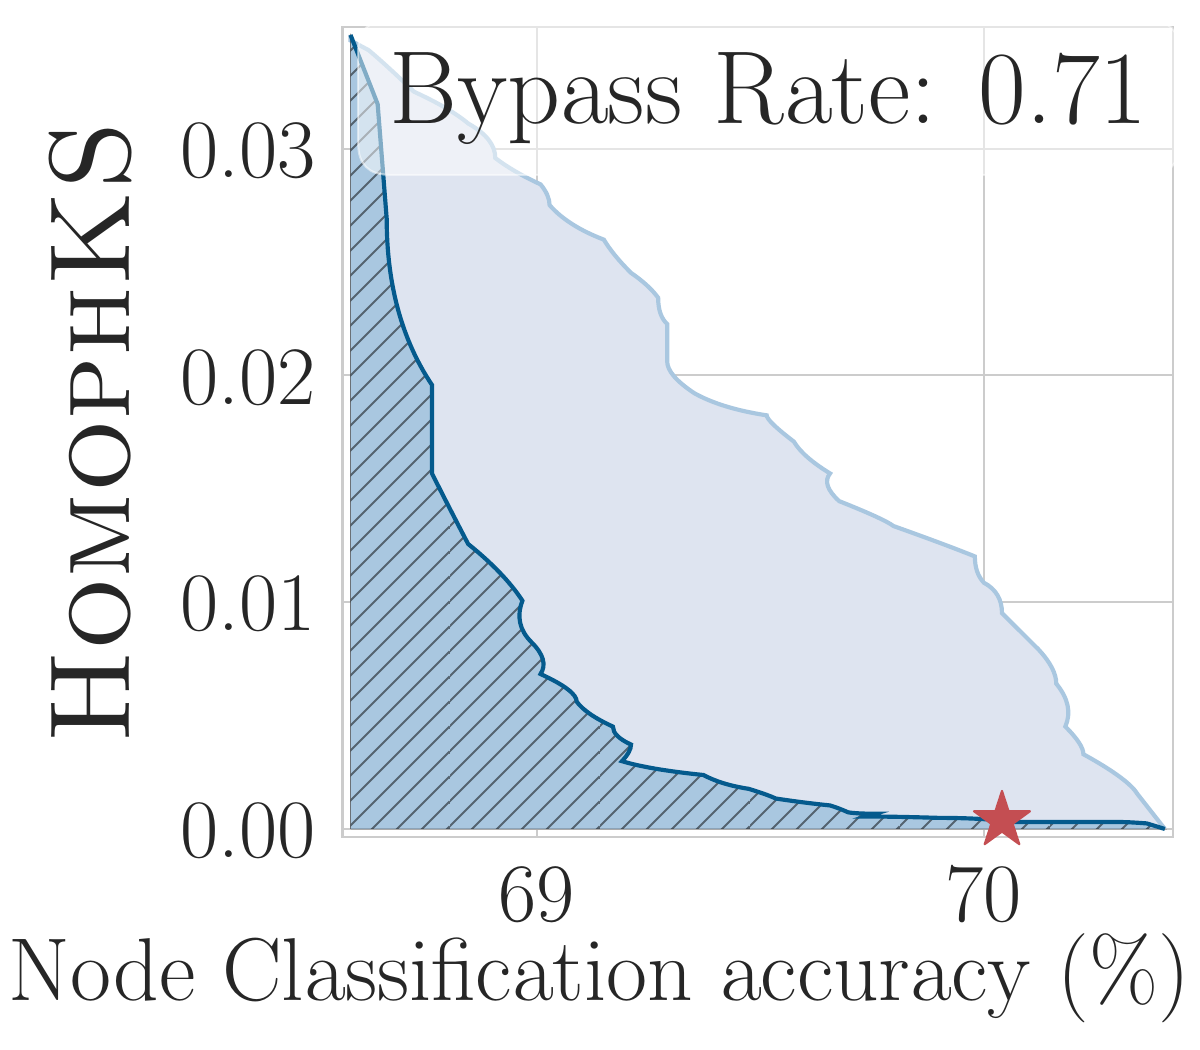} &
        \includegraphics[width=\linewidth]{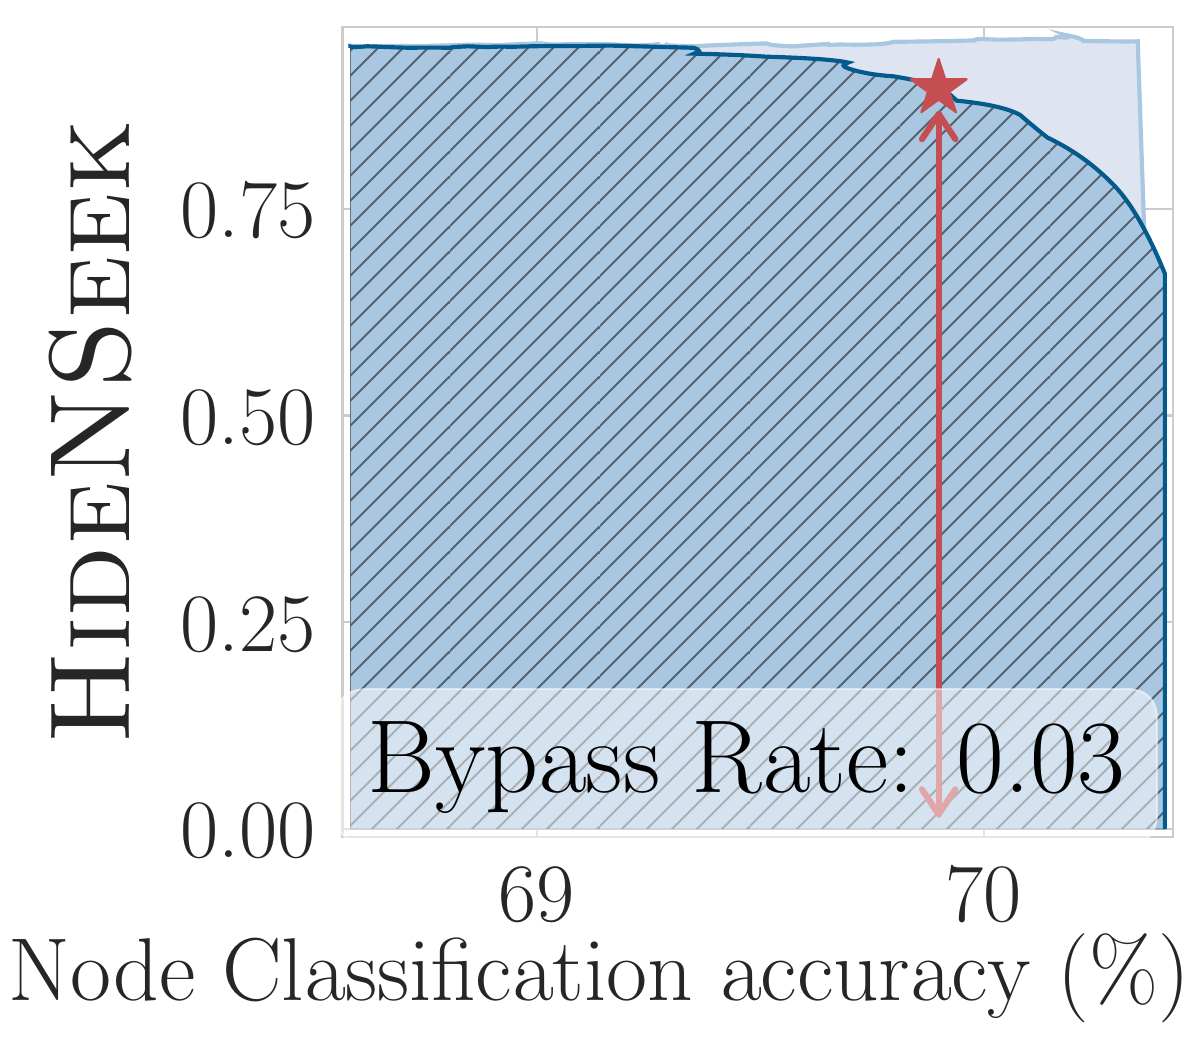} \\
        \hline
        \rotatebox[origin=c]{90}{\coraml} & 
        \includegraphics[width=\linewidth]{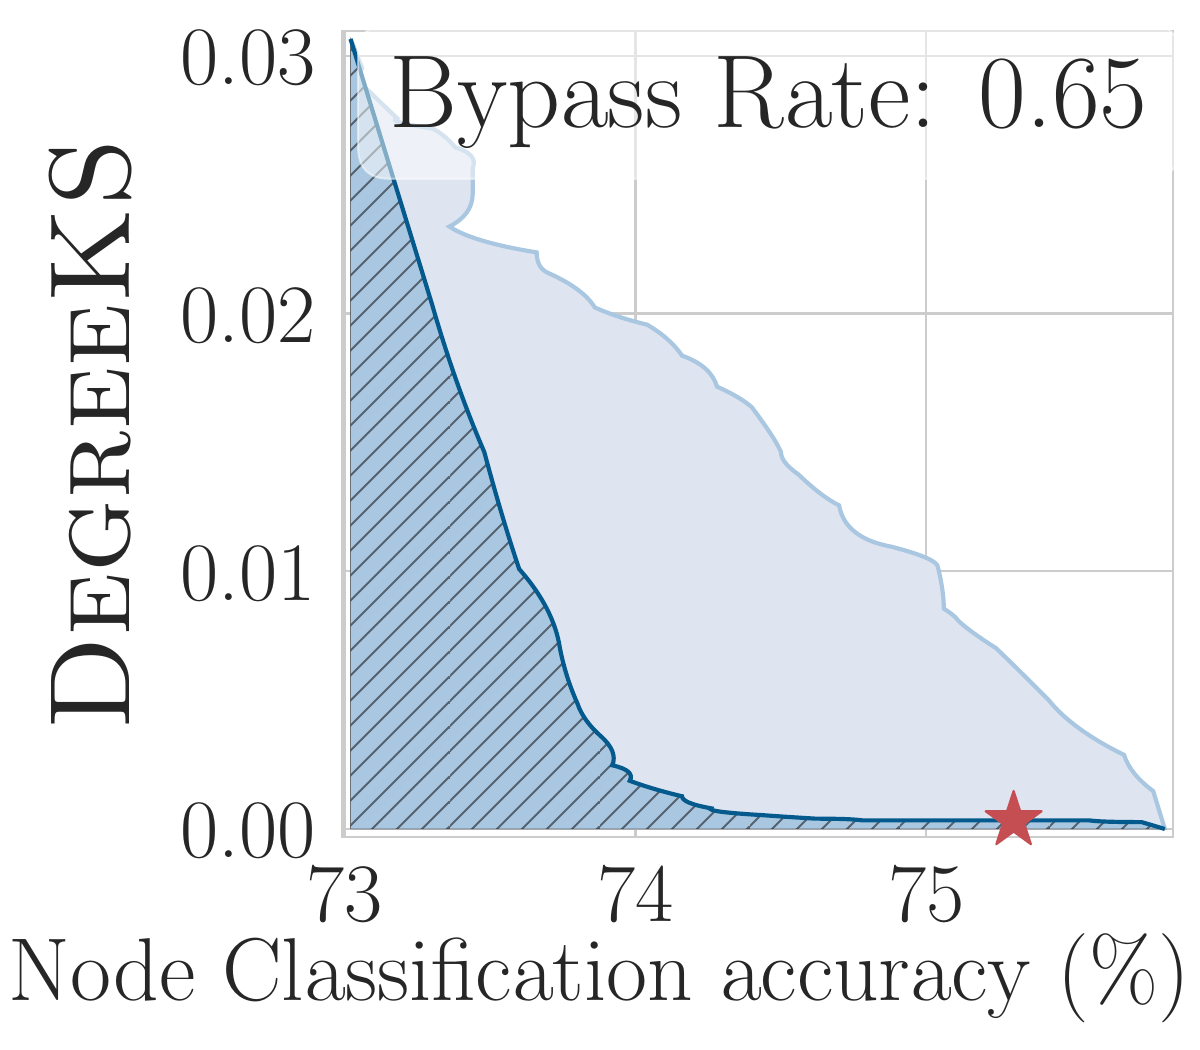} & 
        \includegraphics[width=\linewidth]{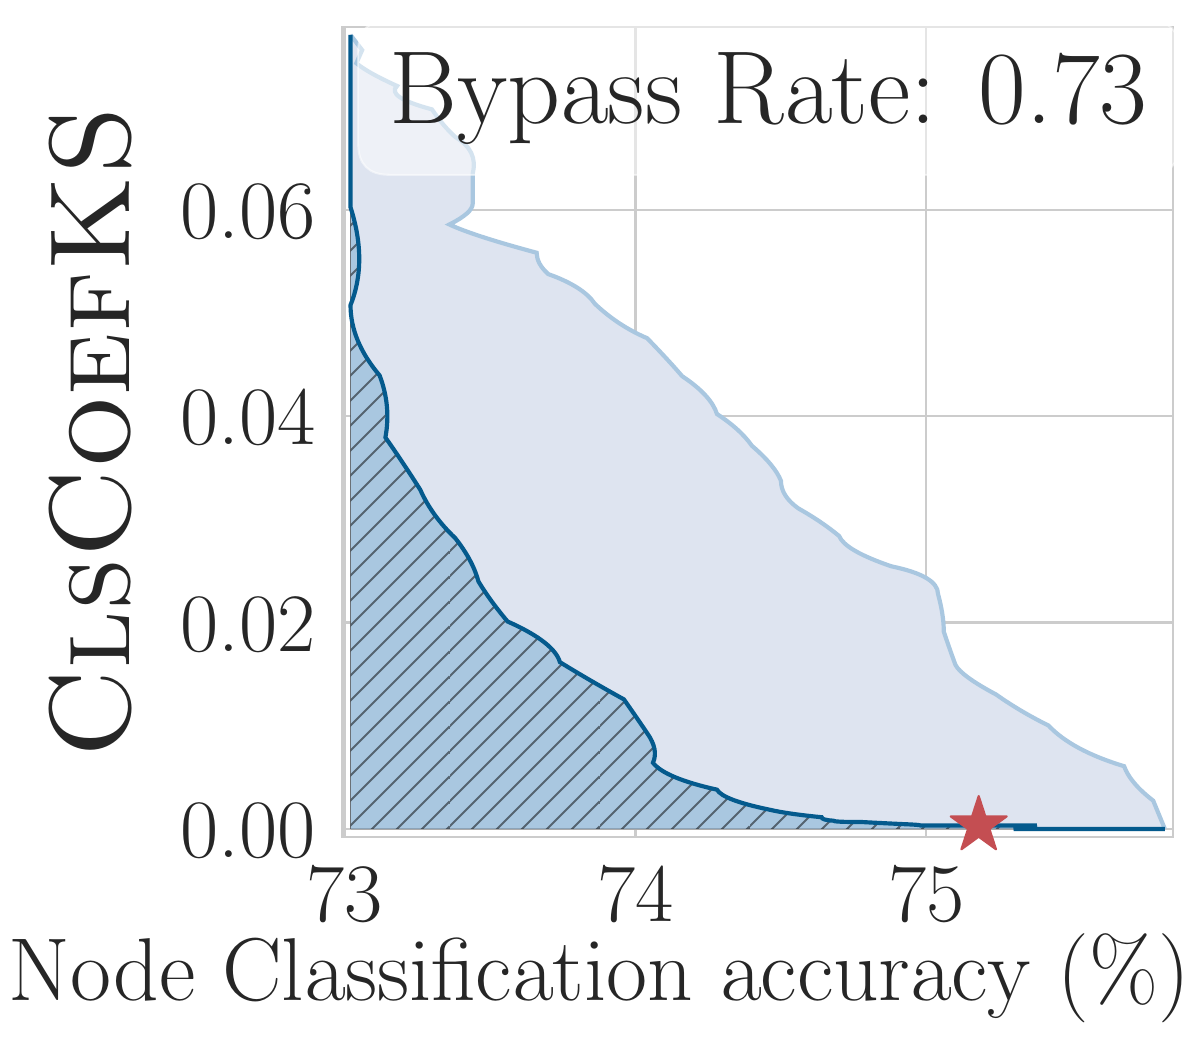} & 
        \includegraphics[width=\linewidth]{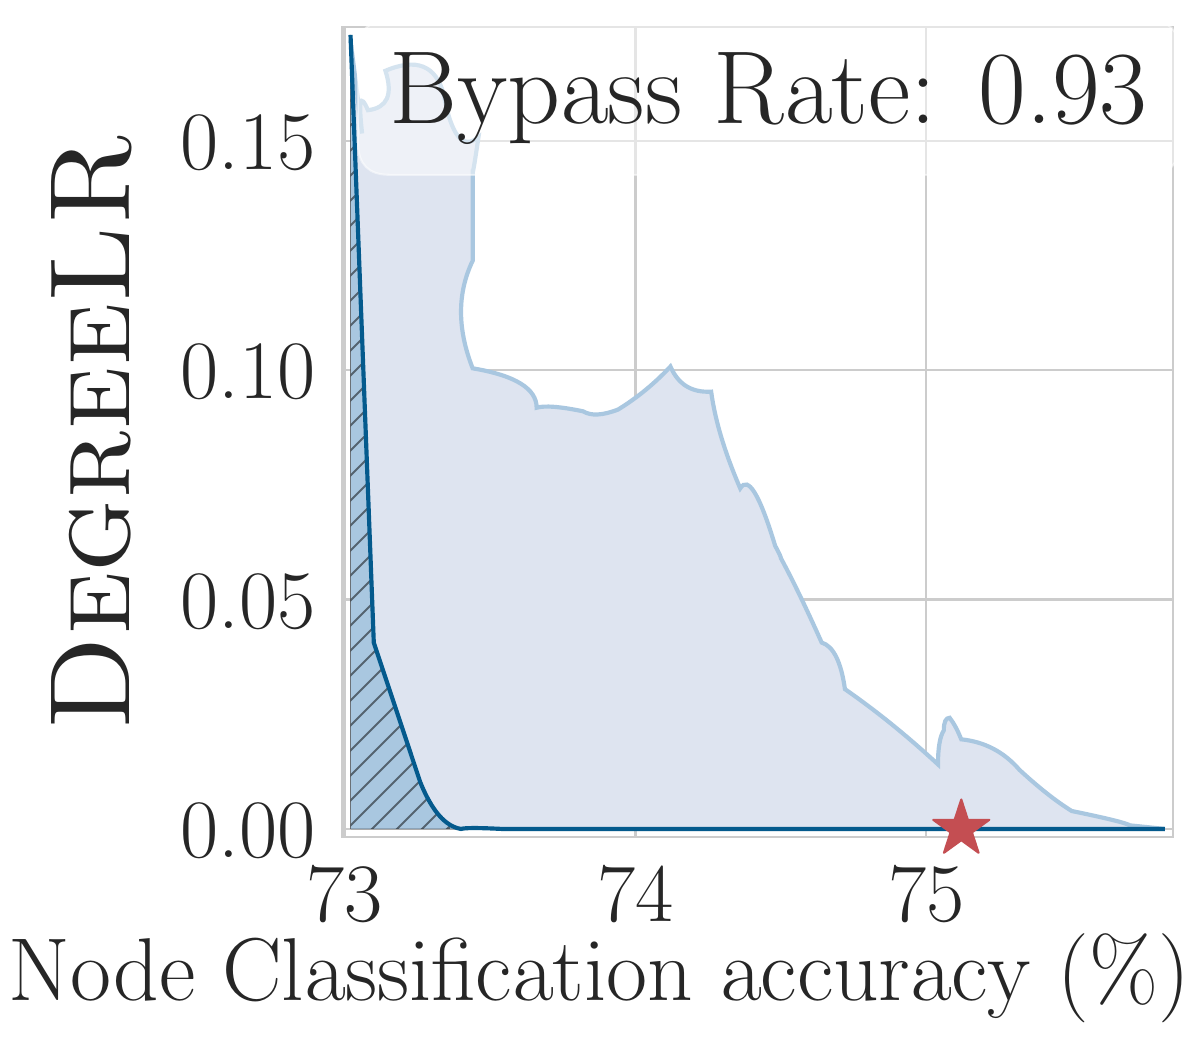} & 
        \includegraphics[width=\linewidth]{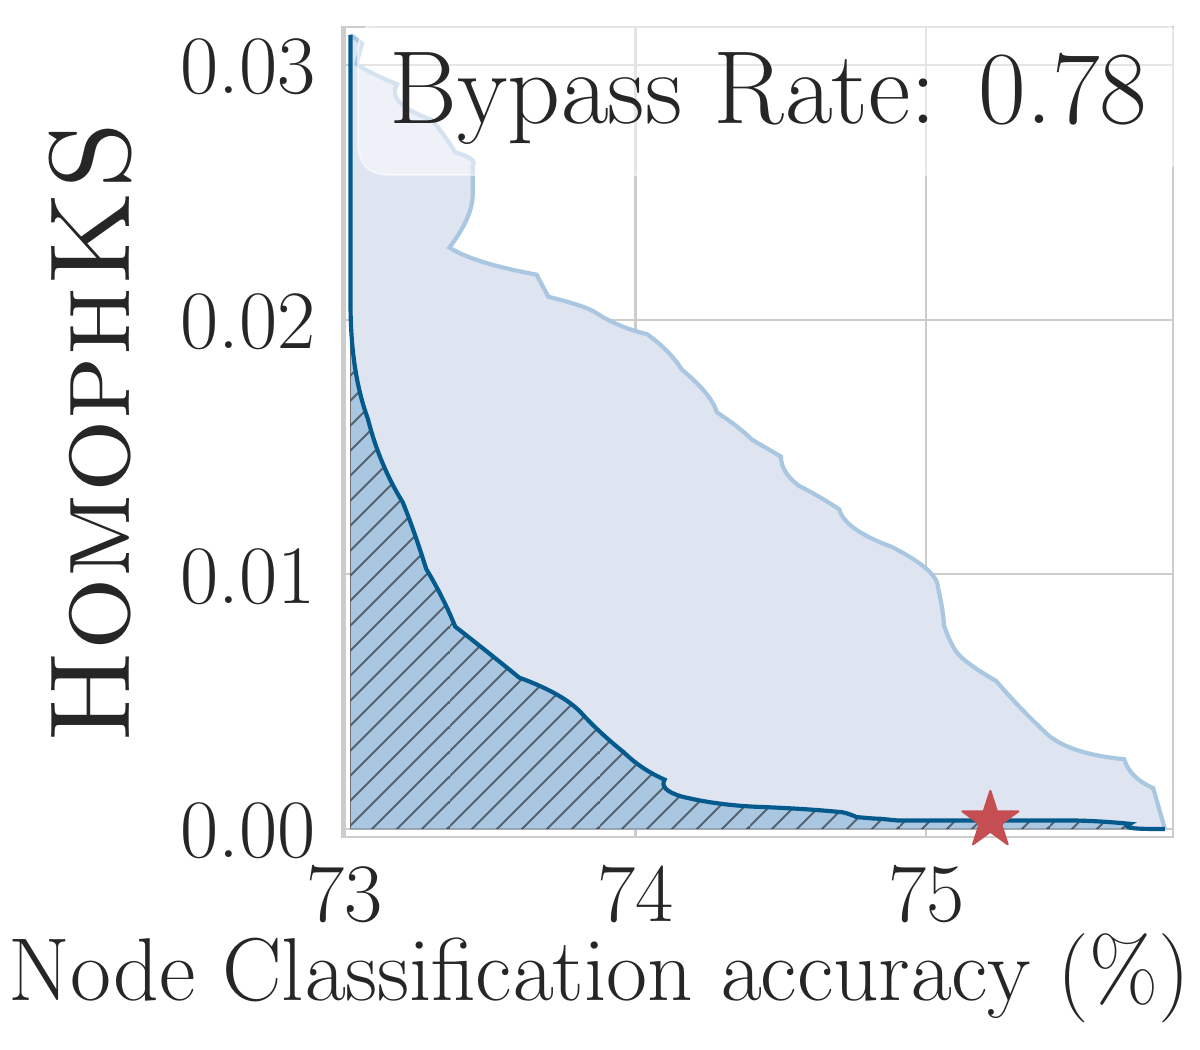} &
        \includegraphics[width=\linewidth]{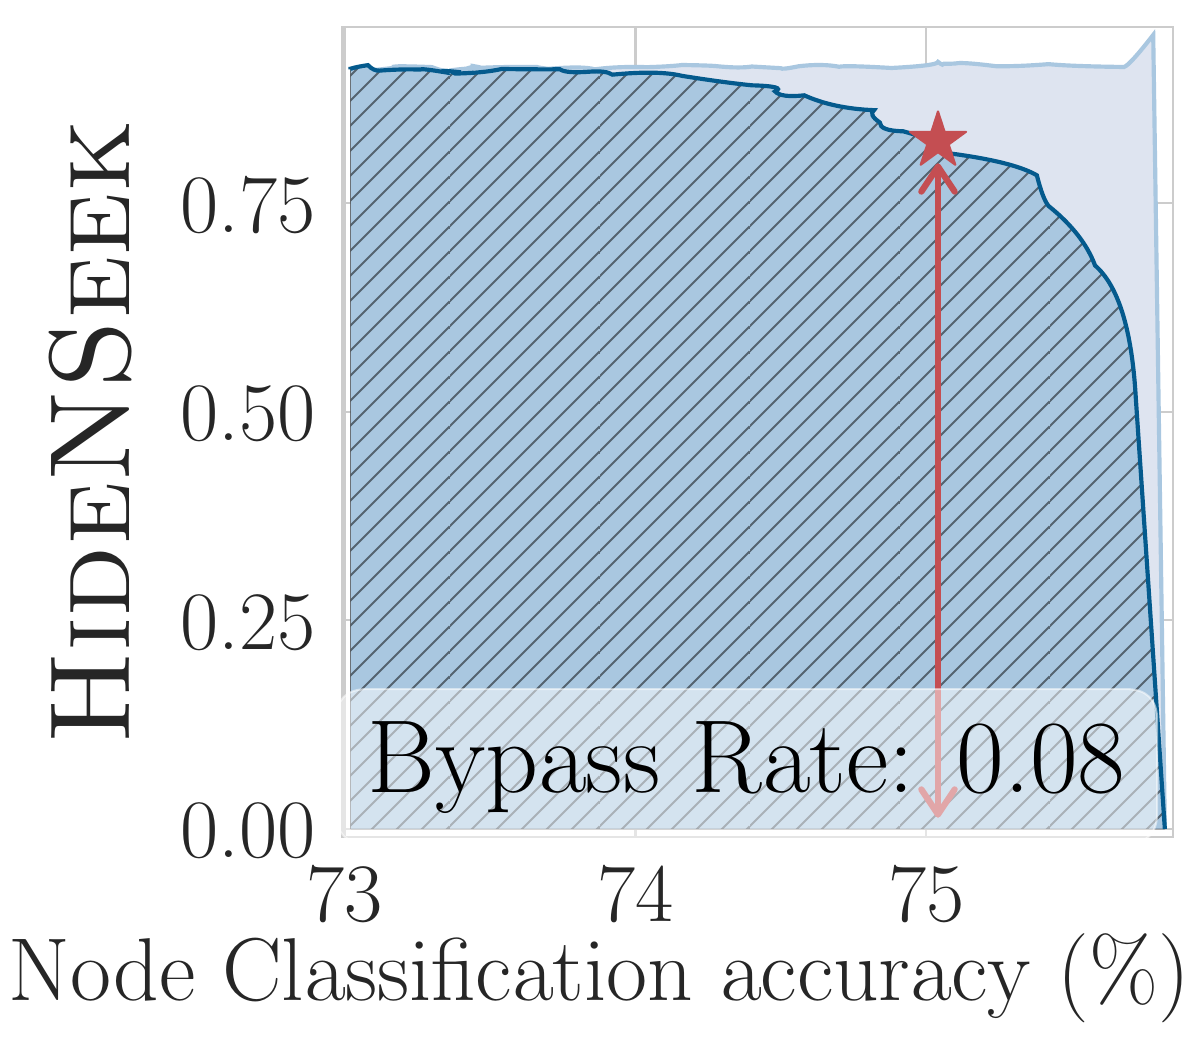} \\
        \hline
        \rotatebox[origin=c]{90}{\lastfmasia} & 
        \includegraphics[width=\linewidth]{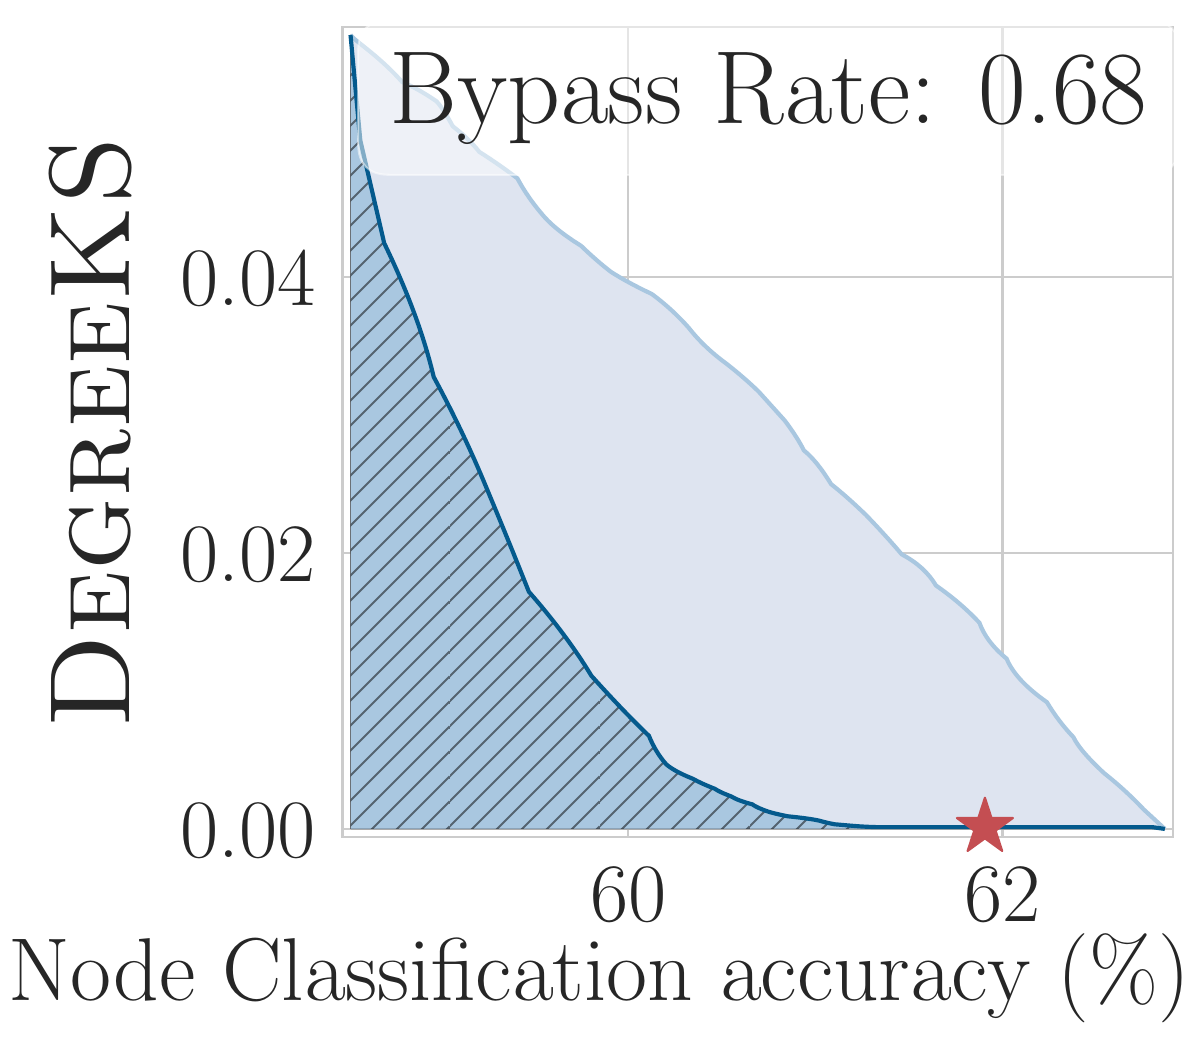} & 
        \includegraphics[width=\linewidth]{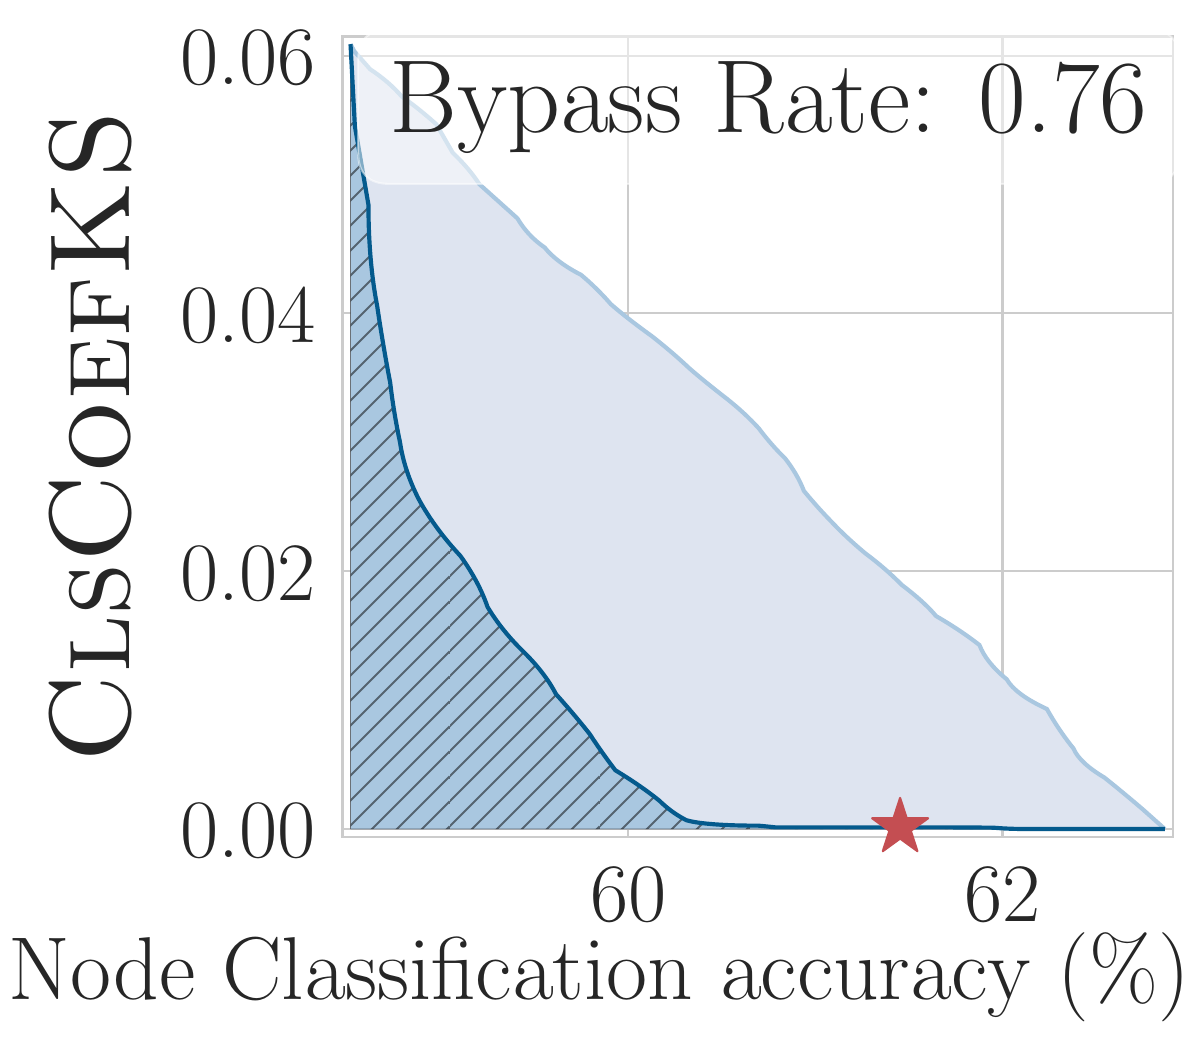} & 
        \includegraphics[width=\linewidth]{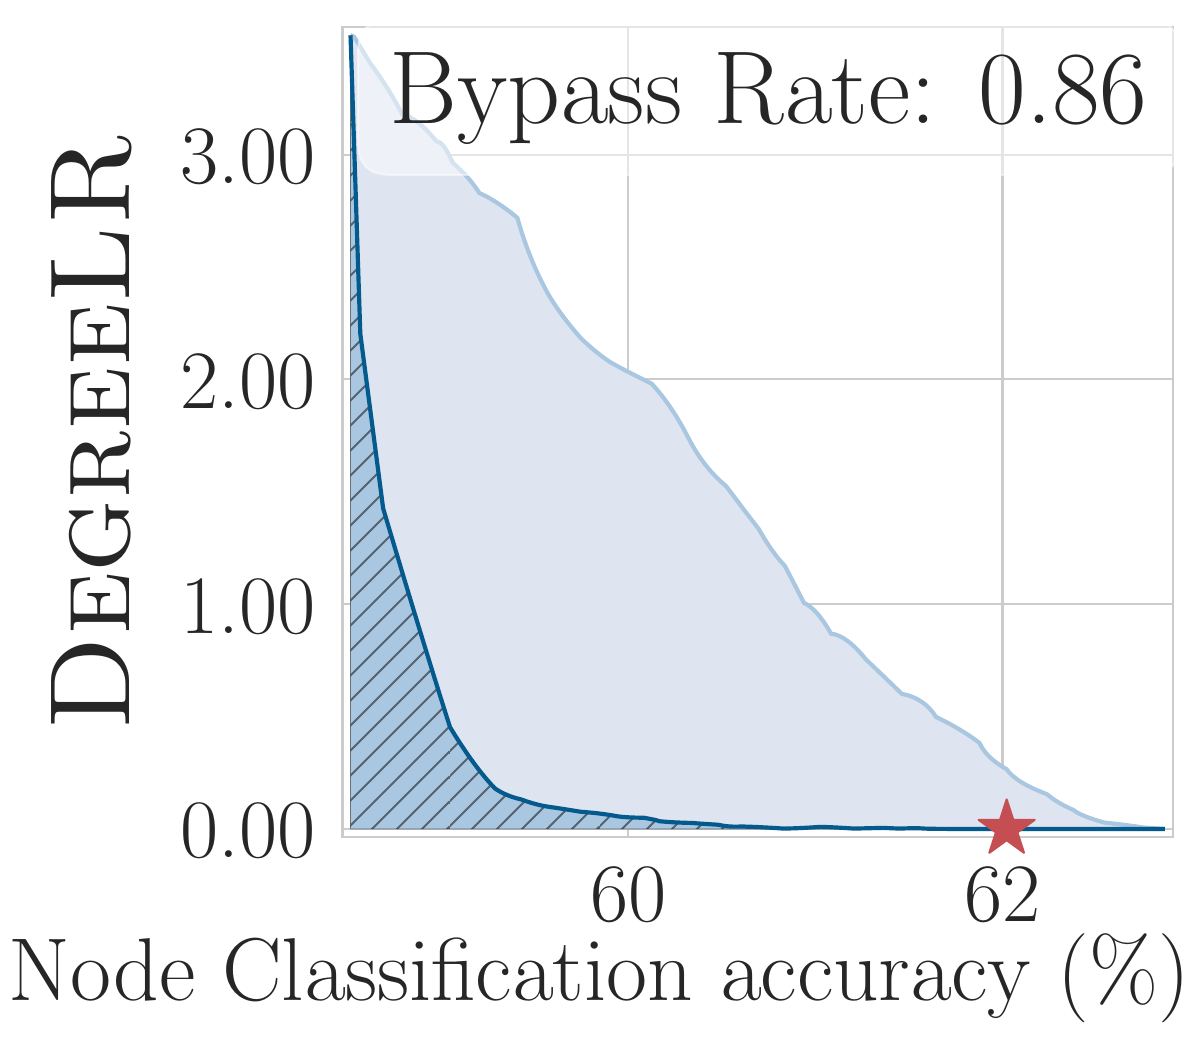} & 
        \includegraphics[width=\linewidth]{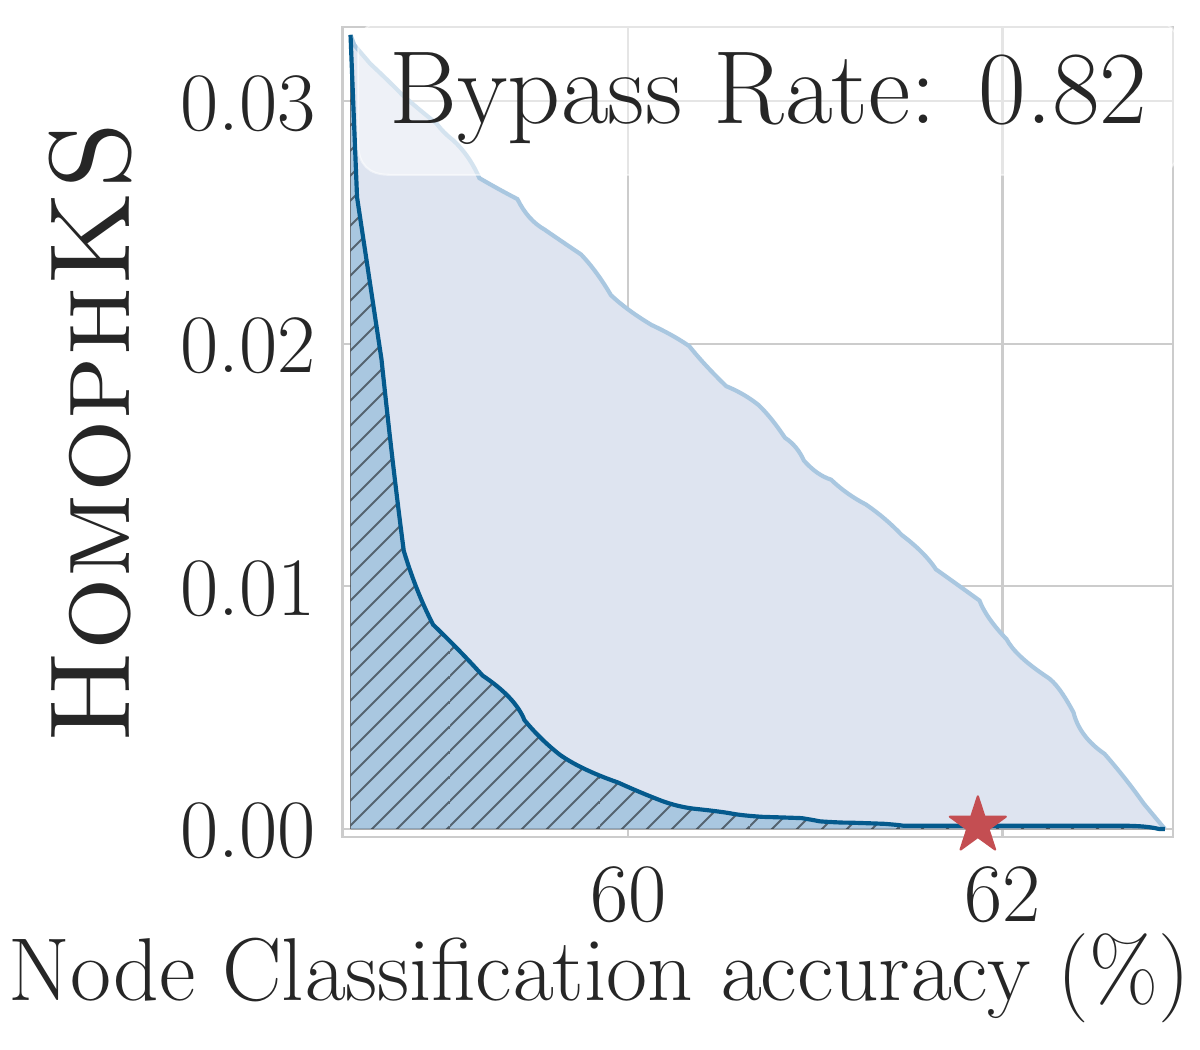} &
        \includegraphics[width=\linewidth]{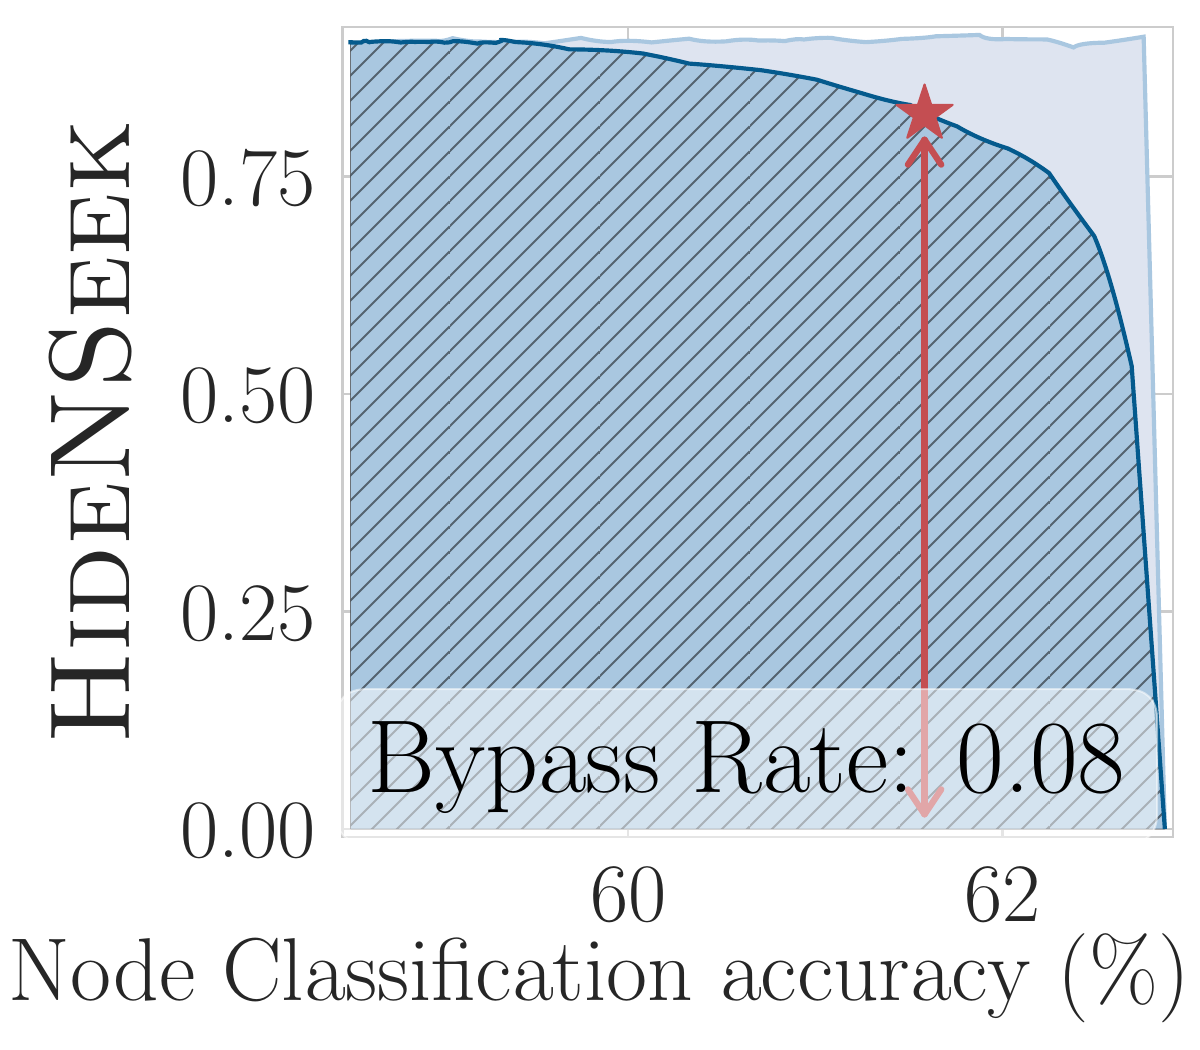} \\
        \hline
        % \rotatebox[origin=c]{90}{\chameleon} & 
        % \includegraphics[width=\linewidth]{FIG/EXP/chameleon/chameleon_dice_degree_q2.pdf} & 
        % \includegraphics[width=\linewidth]{FIG/EXP/chameleon/chameleon_dice_lc_q2.pdf} & 
        % \includegraphics[width=\linewidth]{FIG/EXP/chameleon/chameleon_dice_llr_q2.pdf} & 
        % \includegraphics[width=\linewidth]{FIG/EXP/chameleon/chameleon_dice_homophily_q2.pdf} &
        % \includegraphics[width=\linewidth]{FIG/EXP/chameleon/chameleon_dice_our_q2.pdf} \\
        % \hline
        % \rotatebox[origin=c]{90}{\squirrel} & 
        % \includegraphics[width=\linewidth]{FIG/EXP/squirrel/squirrel_dice_degree_q2.pdf} & 
        % \includegraphics[width=\linewidth]{FIG/EXP/squirrel/squirrel_dice_lc_q2.pdf} & 
        % \includegraphics[width=\linewidth]{FIG/EXP/squirrel/squirrel_dice_llr_q2.pdf} & 
        % \includegraphics[width=\linewidth]{FIG/EXP/squirrel/squirrel_dice_homophily_q2.pdf} &
        % \includegraphics[width=\linewidth]{FIG/EXP/squirrel/squirrel_dice_our_q2.pdf} \\
        % \hline
    \end{tabular}
    }
    \label{tab:exp:q2_dice}
\end{table*}

\newcolumntype{C}{>{\centering\arraybackslash}m{0.15\linewidth}}
\begin{table*}
    \centering
    \caption{The additional experimental results regarding Q2 \& Q3  on \structack.}
    \resizebox{0.8\textwidth}{!}{
    \begin{tabular}{l||C|C|C|C||C}
        \hline
        % & \multicolumn{4}{c||}{Existing Measures} & \multirow{3}{*}{\textbf{\measure}} \\ 
        % \cline{2-5}
        % & Degree Dist. & Clustering Coeff. & Degree Dist. & Homophily Dist. & \\
        % & (KS test) & (KS test) & (LR test)& (KS test) & \\
        & \textsc{DegreeKS} & \textsc{ClsCoefKS} & \textsc{DegreeLR} & \textsc{HomophKS} & \textbf{\measure} \\
        \hline\hline
        \rotatebox[origin=c]{90}{\cora} & 
        \includegraphics[width=\linewidth]{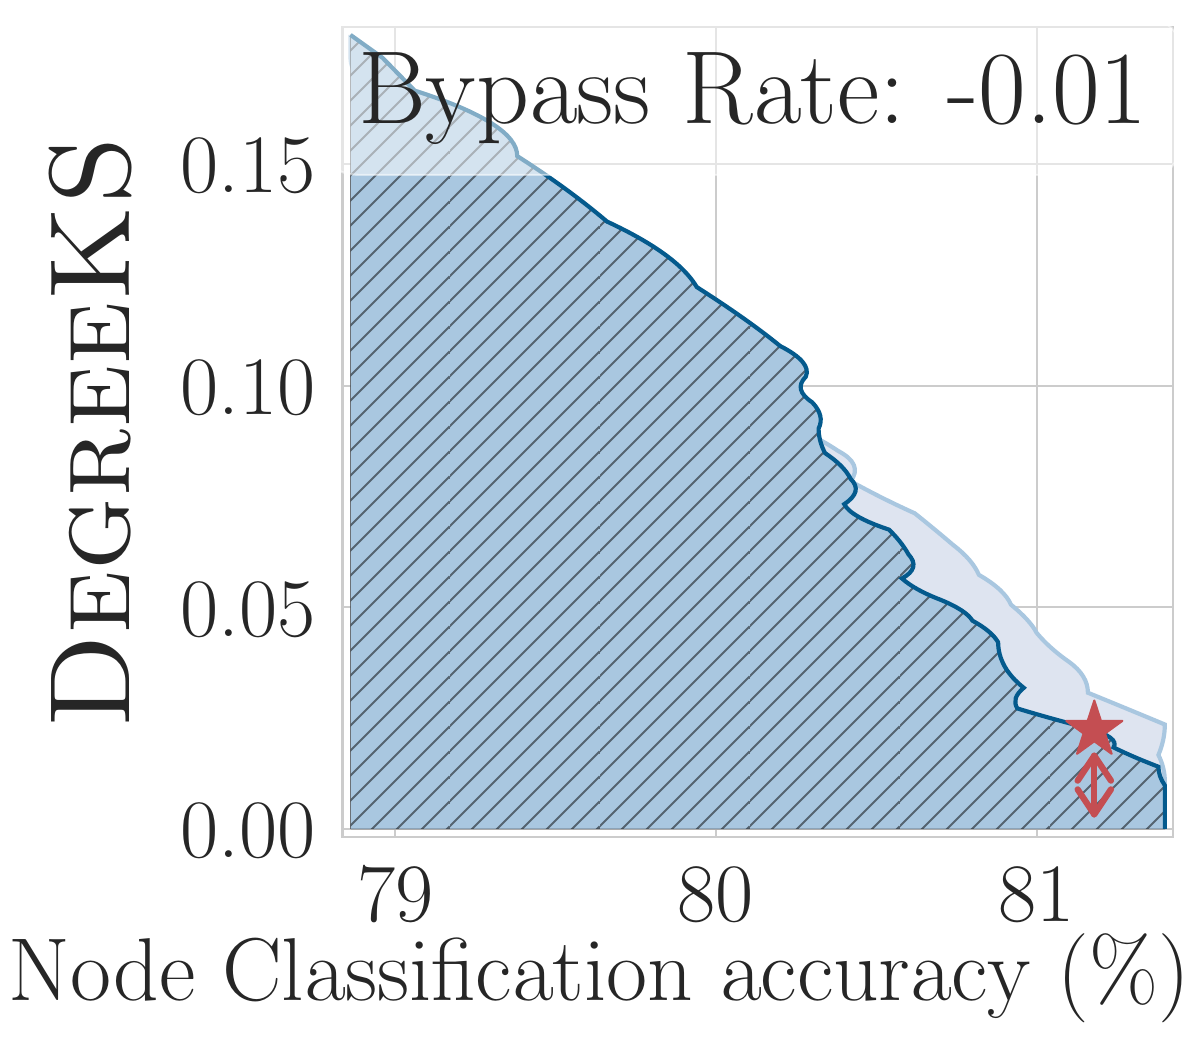} & 
        \includegraphics[width=\linewidth]{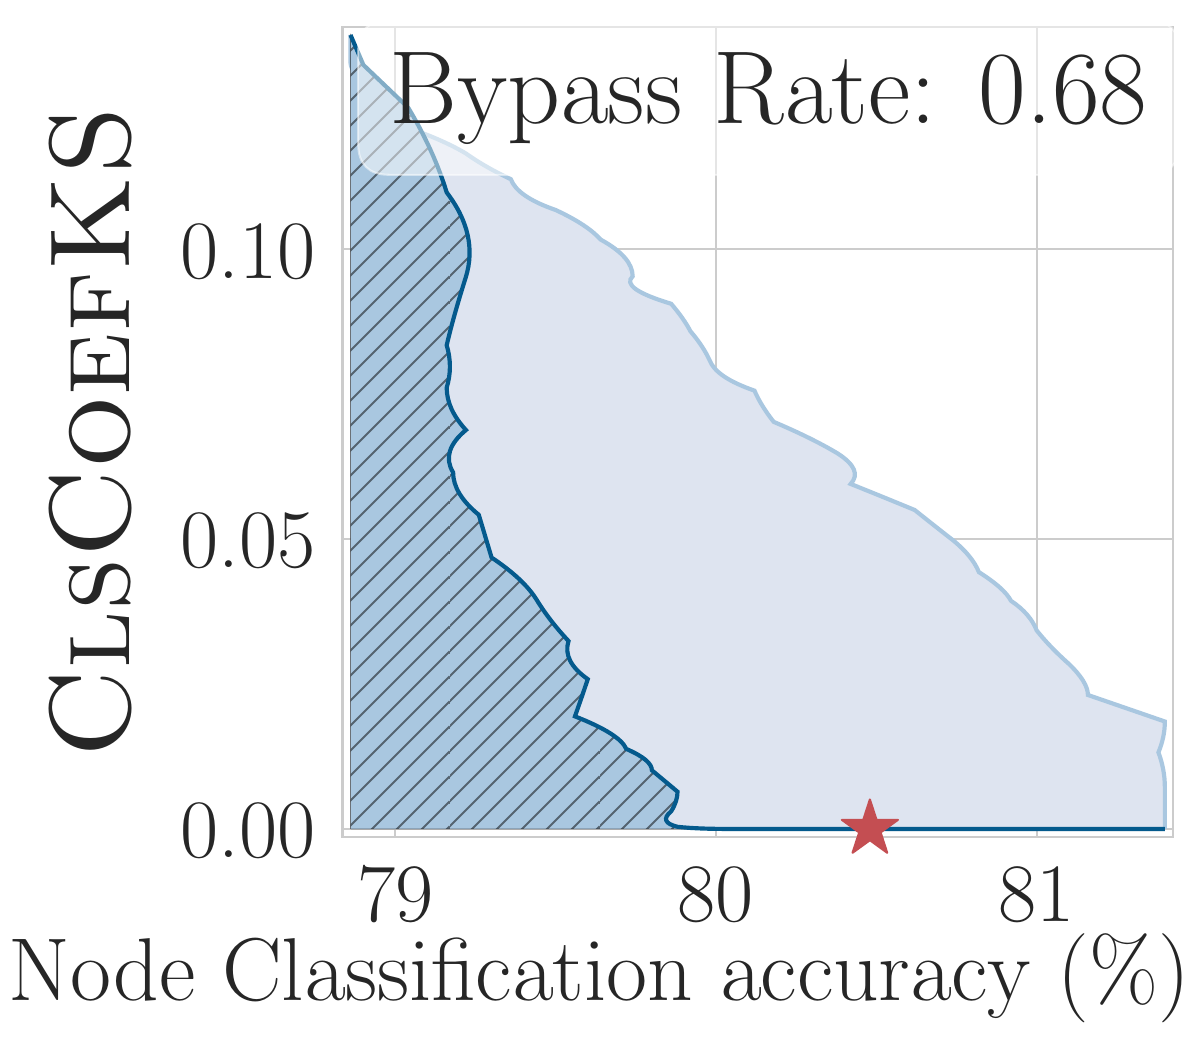} & 
        \includegraphics[width=\linewidth]{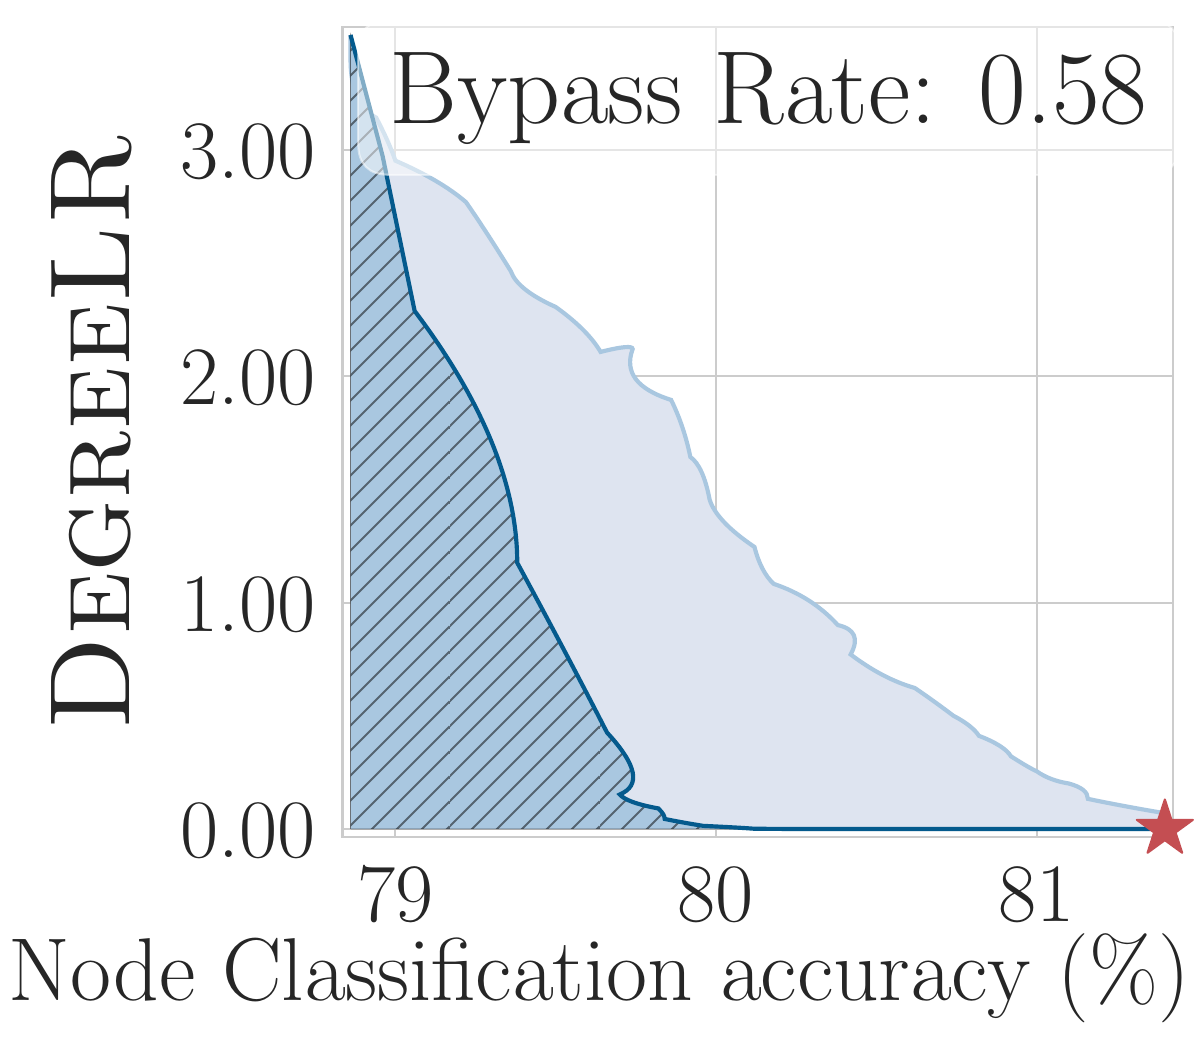} & 
        \includegraphics[width=\linewidth]{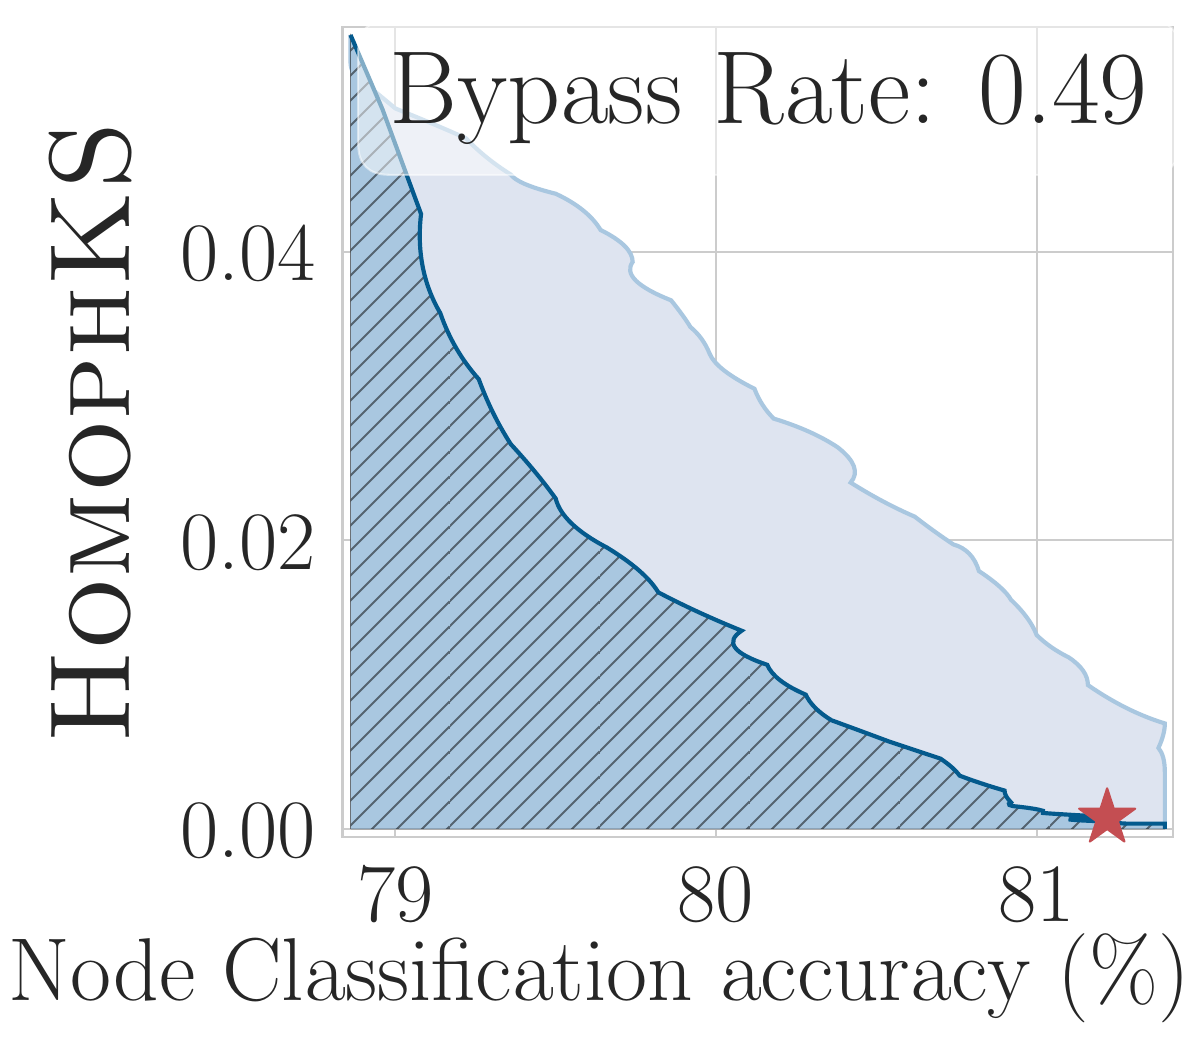} &
        \includegraphics[width=\linewidth]{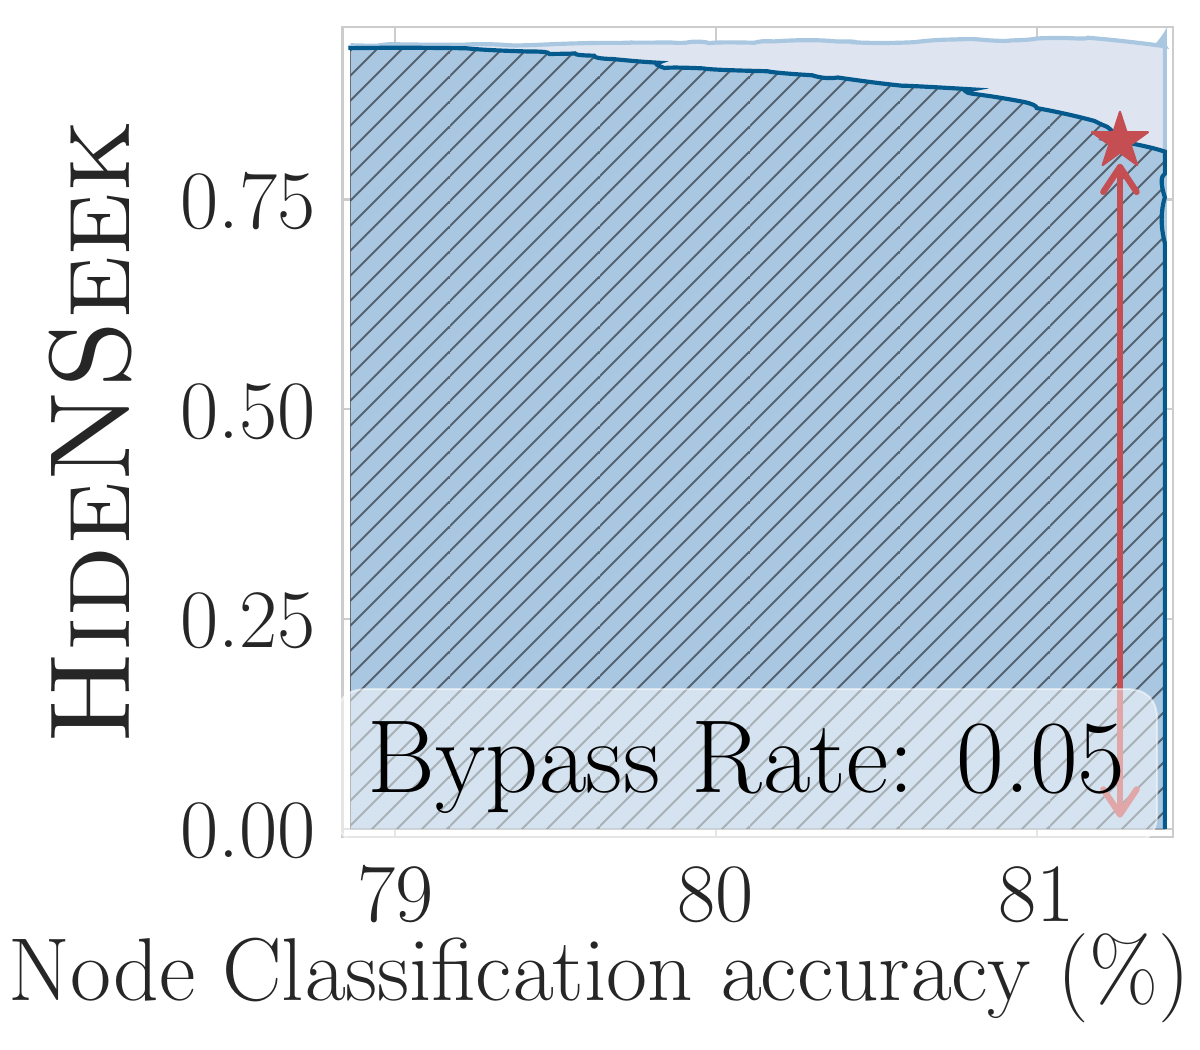} \\
        \hline
        \rotatebox[origin=c]{90}{\citeseer} & 
        \includegraphics[width=\linewidth]{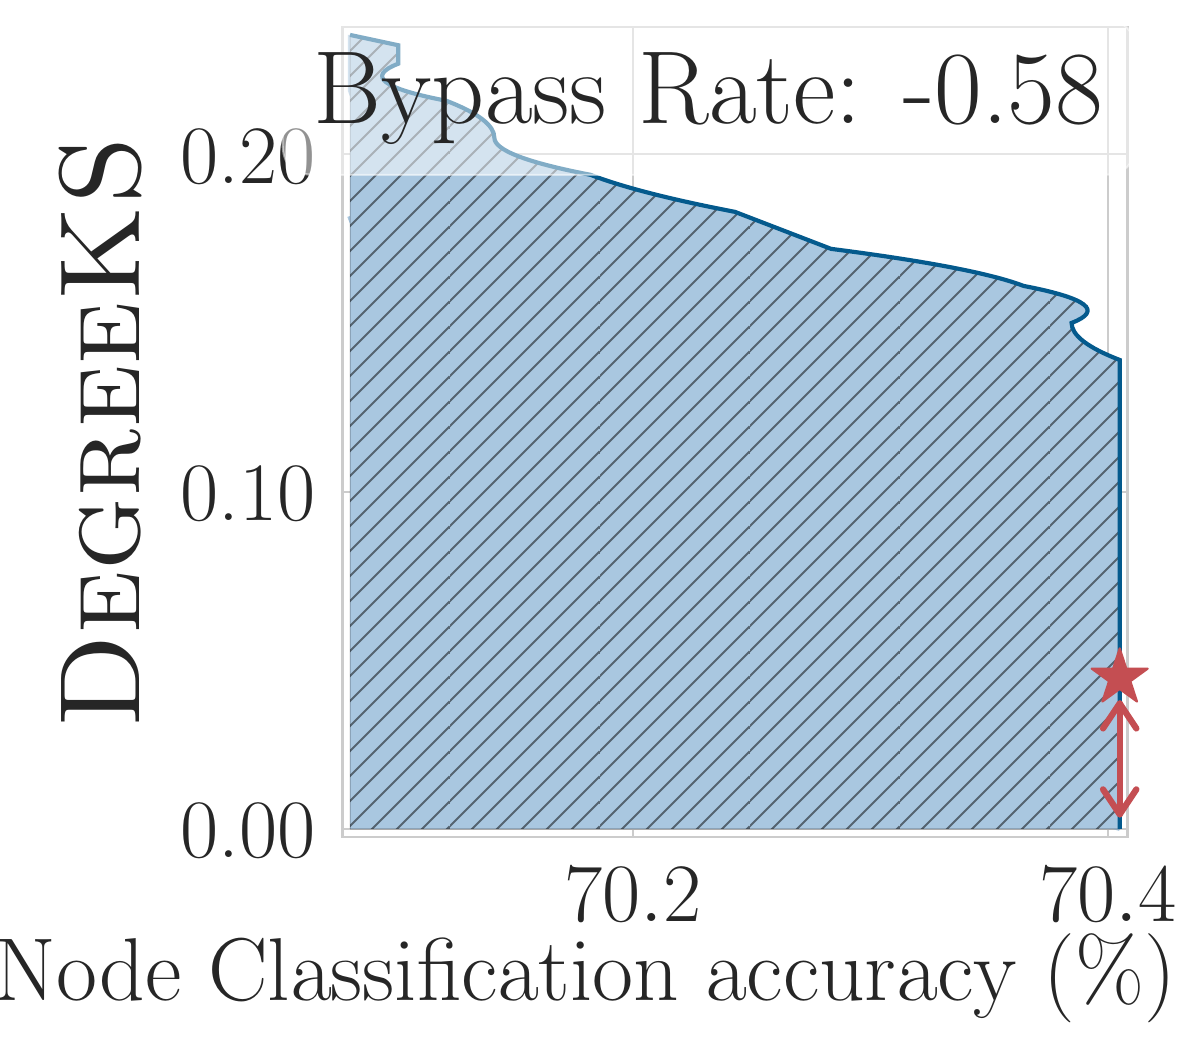} & 
        \includegraphics[width=\linewidth]{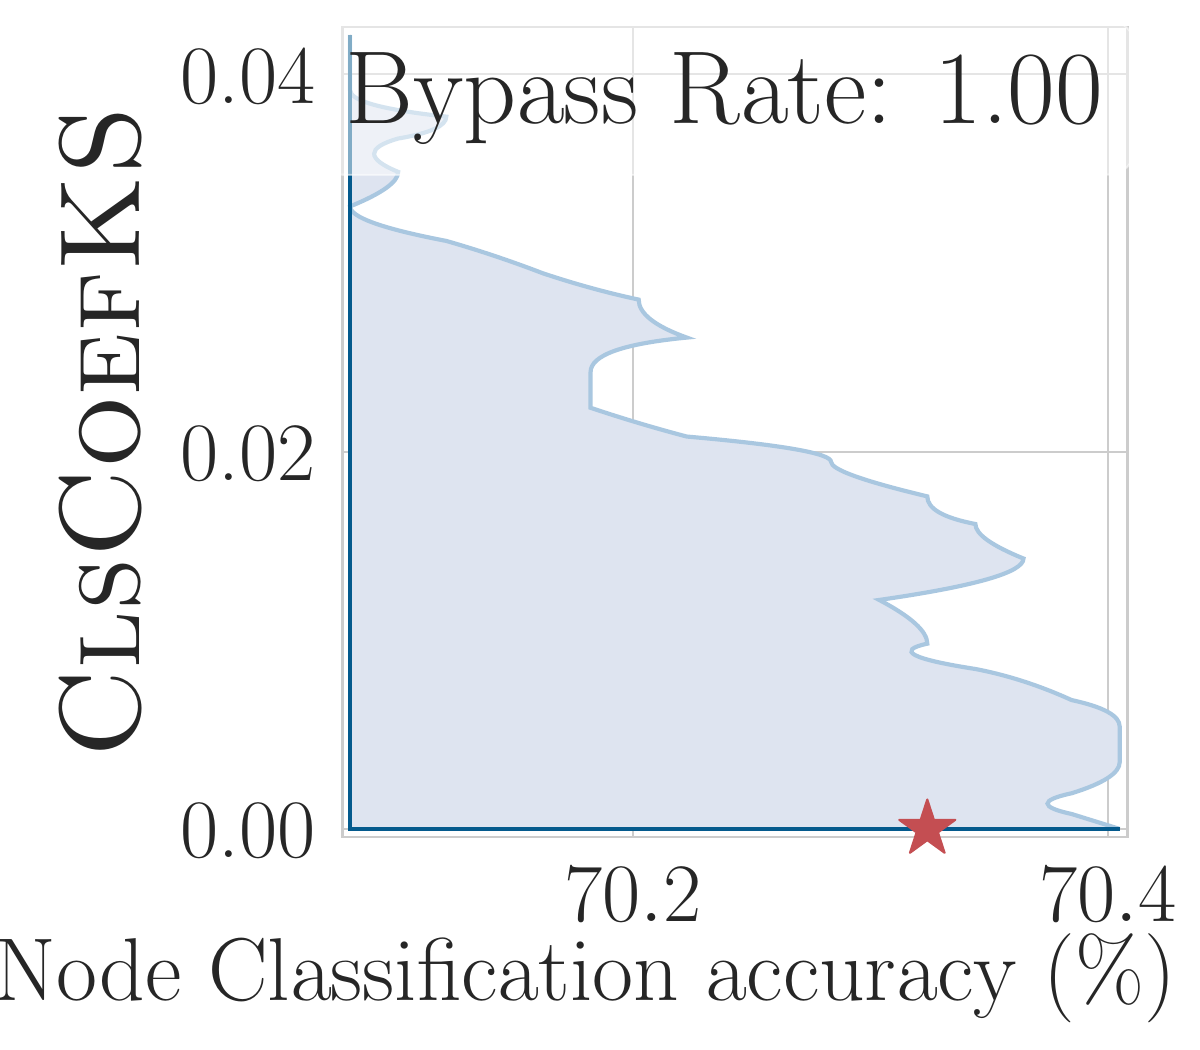} & 
        \includegraphics[width=\linewidth]{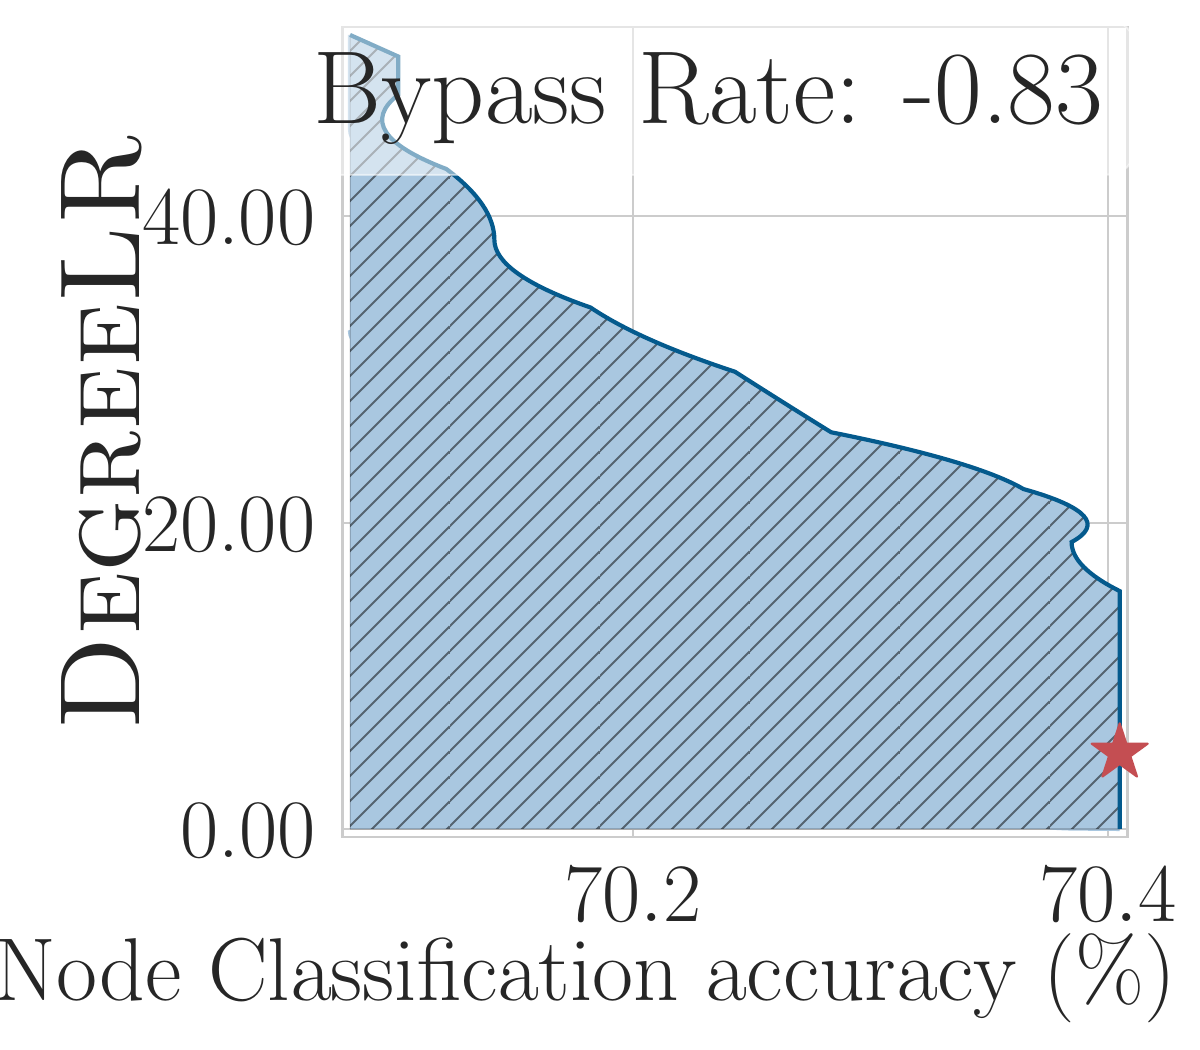} & 
        \includegraphics[width=\linewidth]{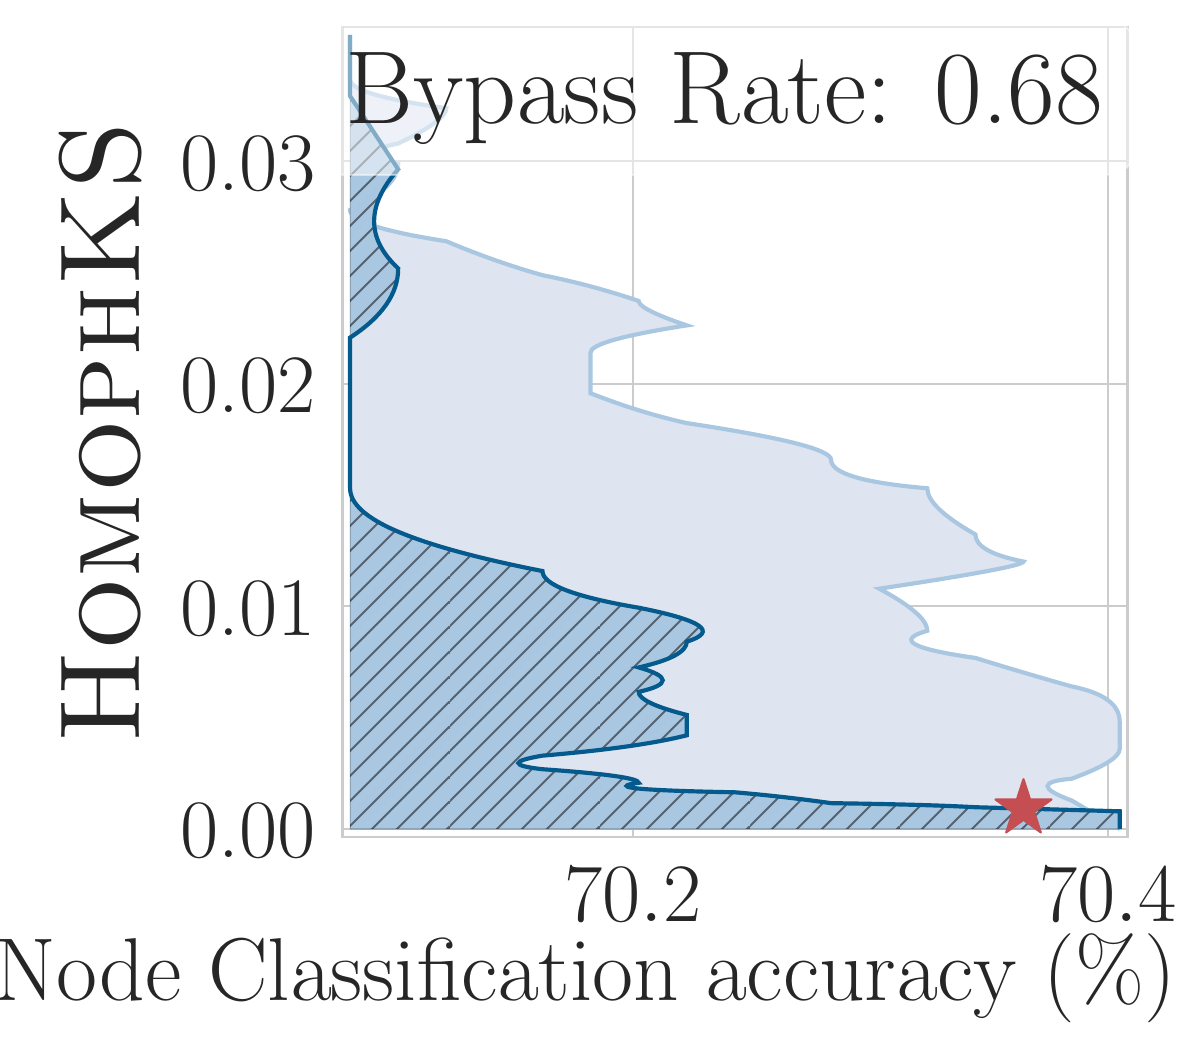} &
        \includegraphics[width=\linewidth]{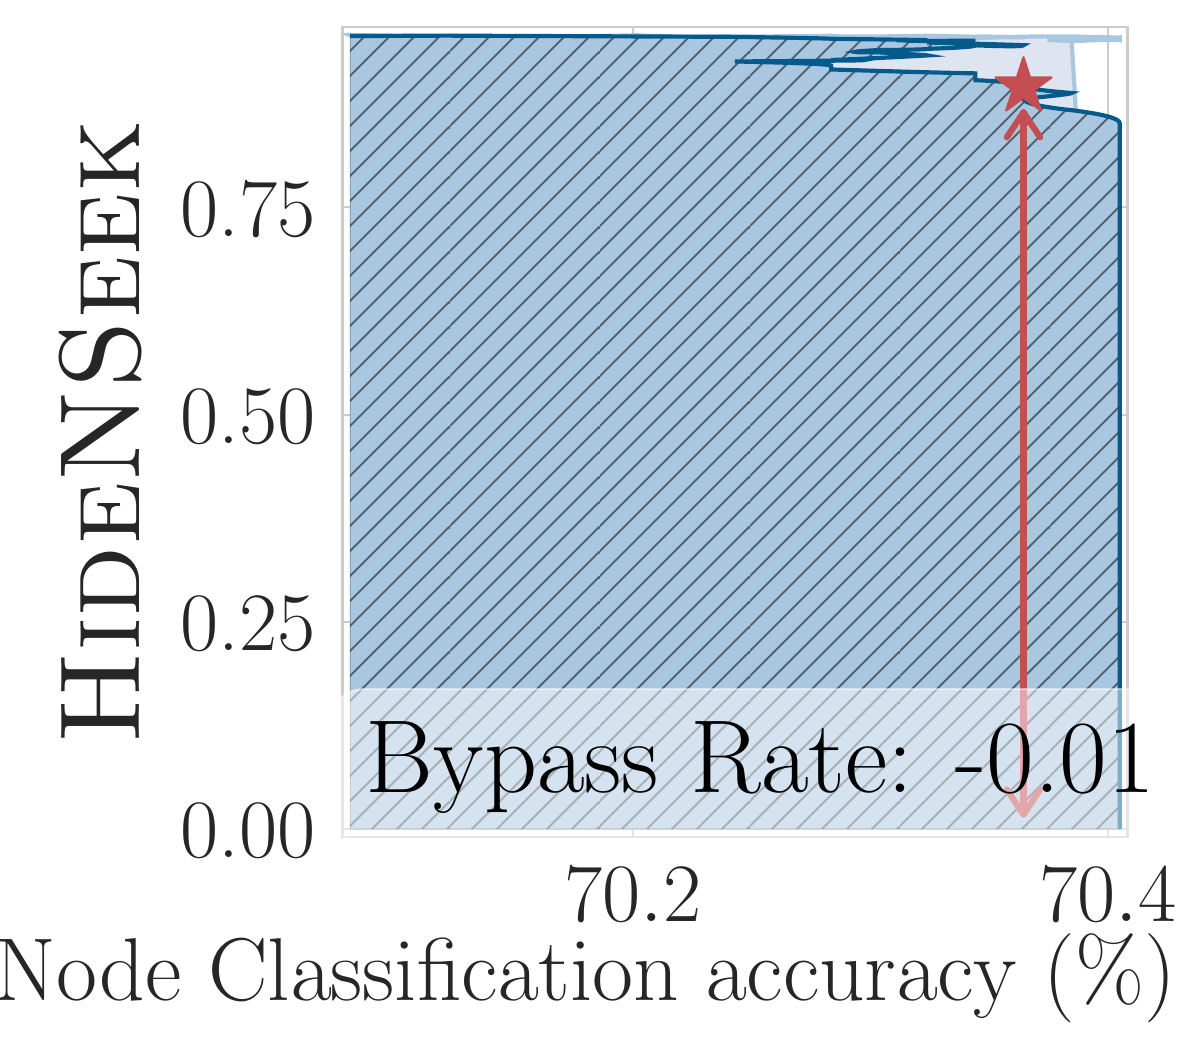} \\
        \hline
        \rotatebox[origin=c]{90}{\coraml} & 
        \includegraphics[width=\linewidth]{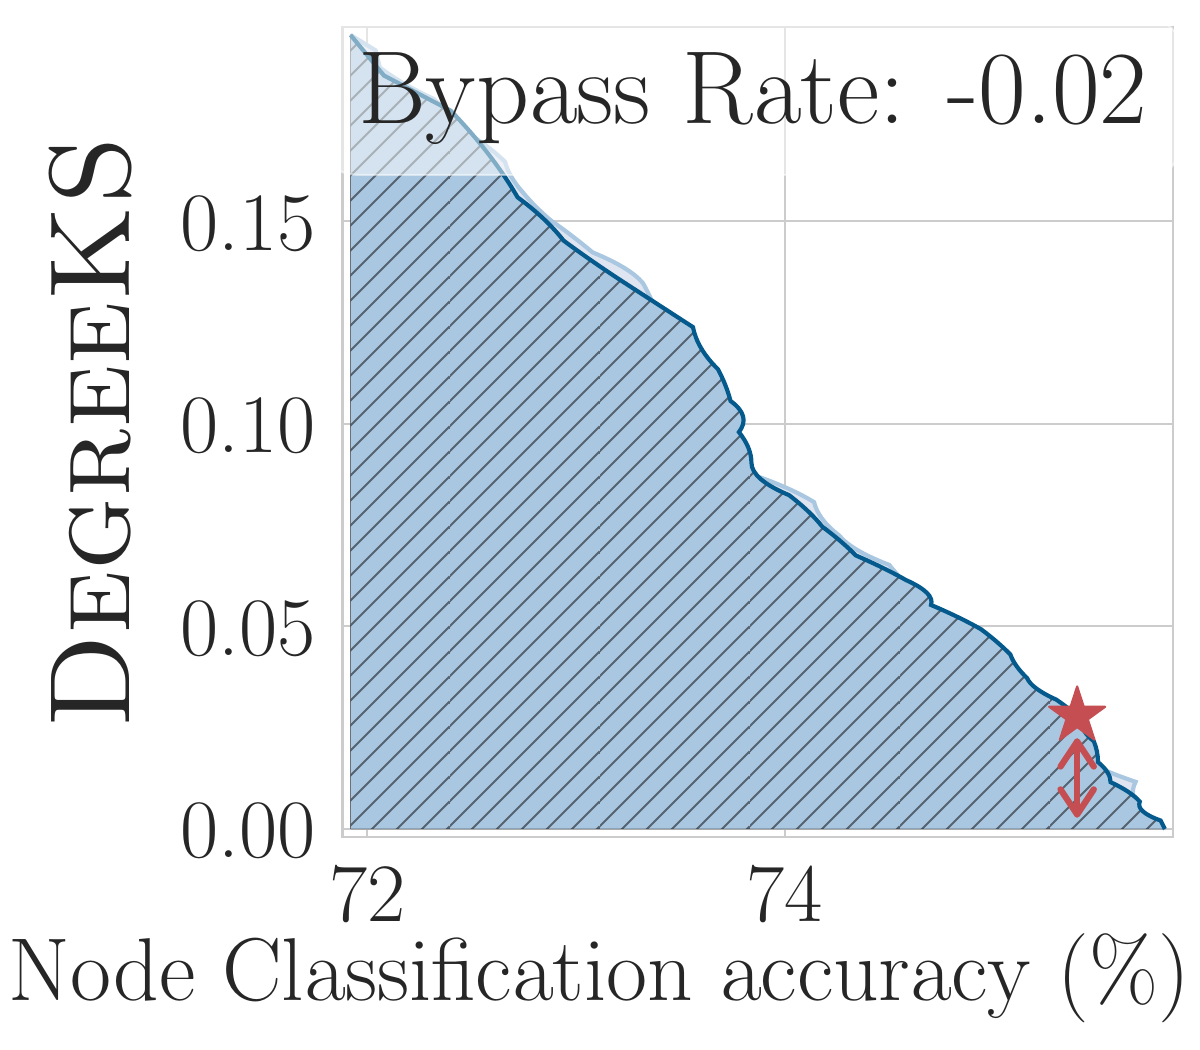} & 
        \includegraphics[width=\linewidth]{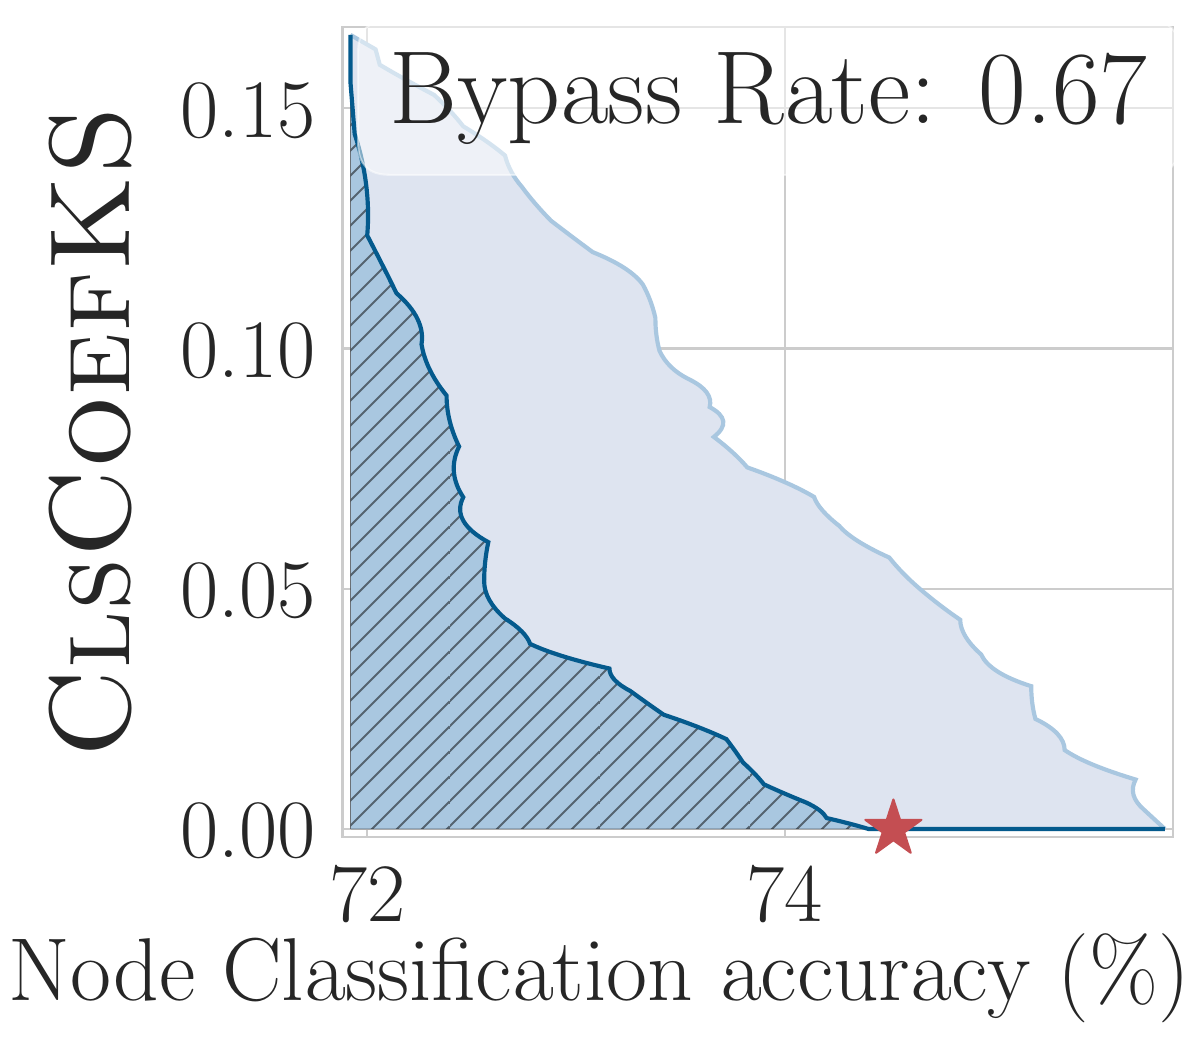} & 
        \includegraphics[width=\linewidth]{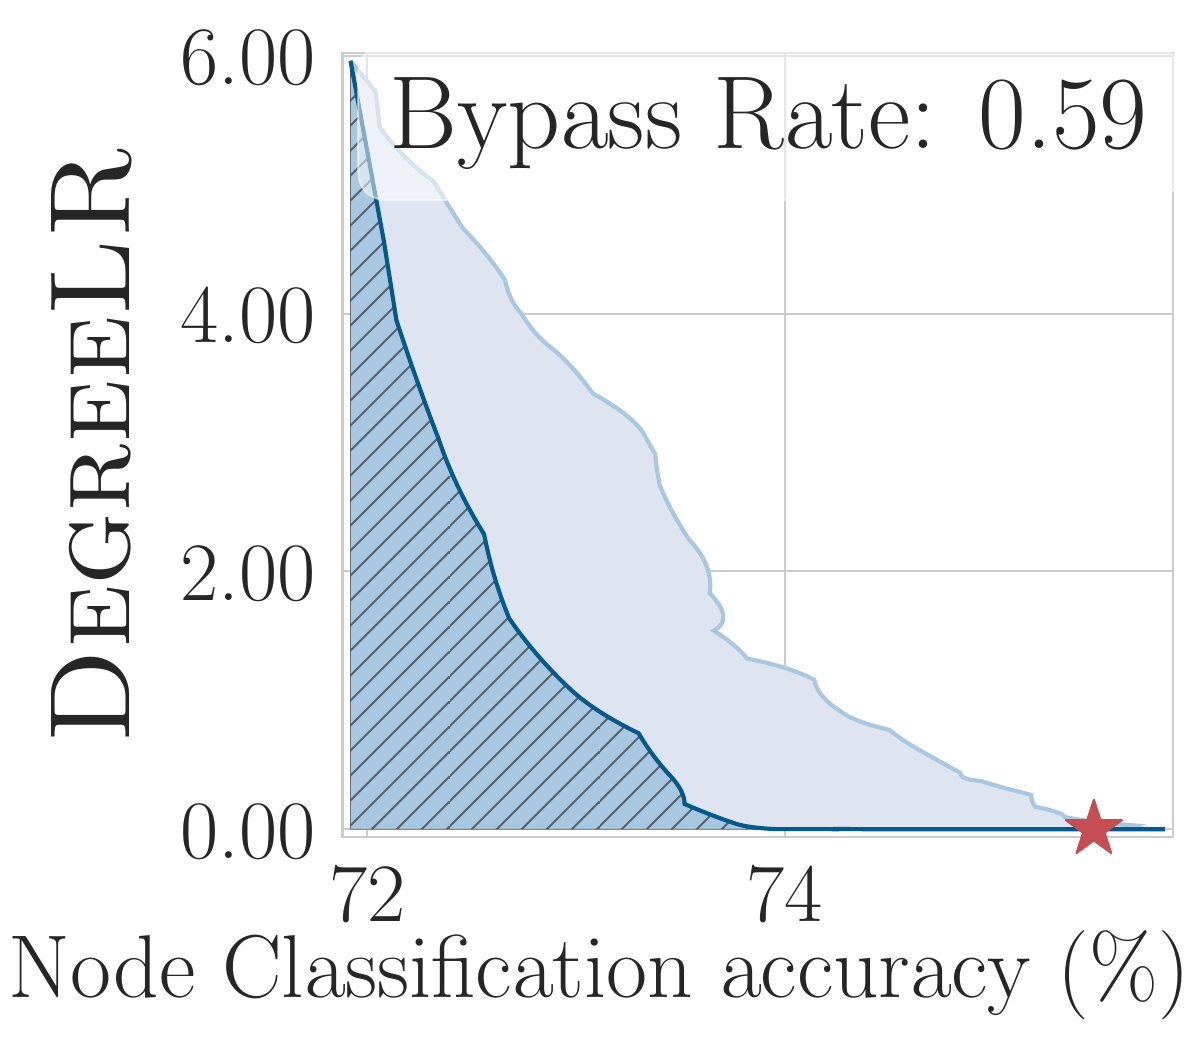} & 
        \includegraphics[width=\linewidth]{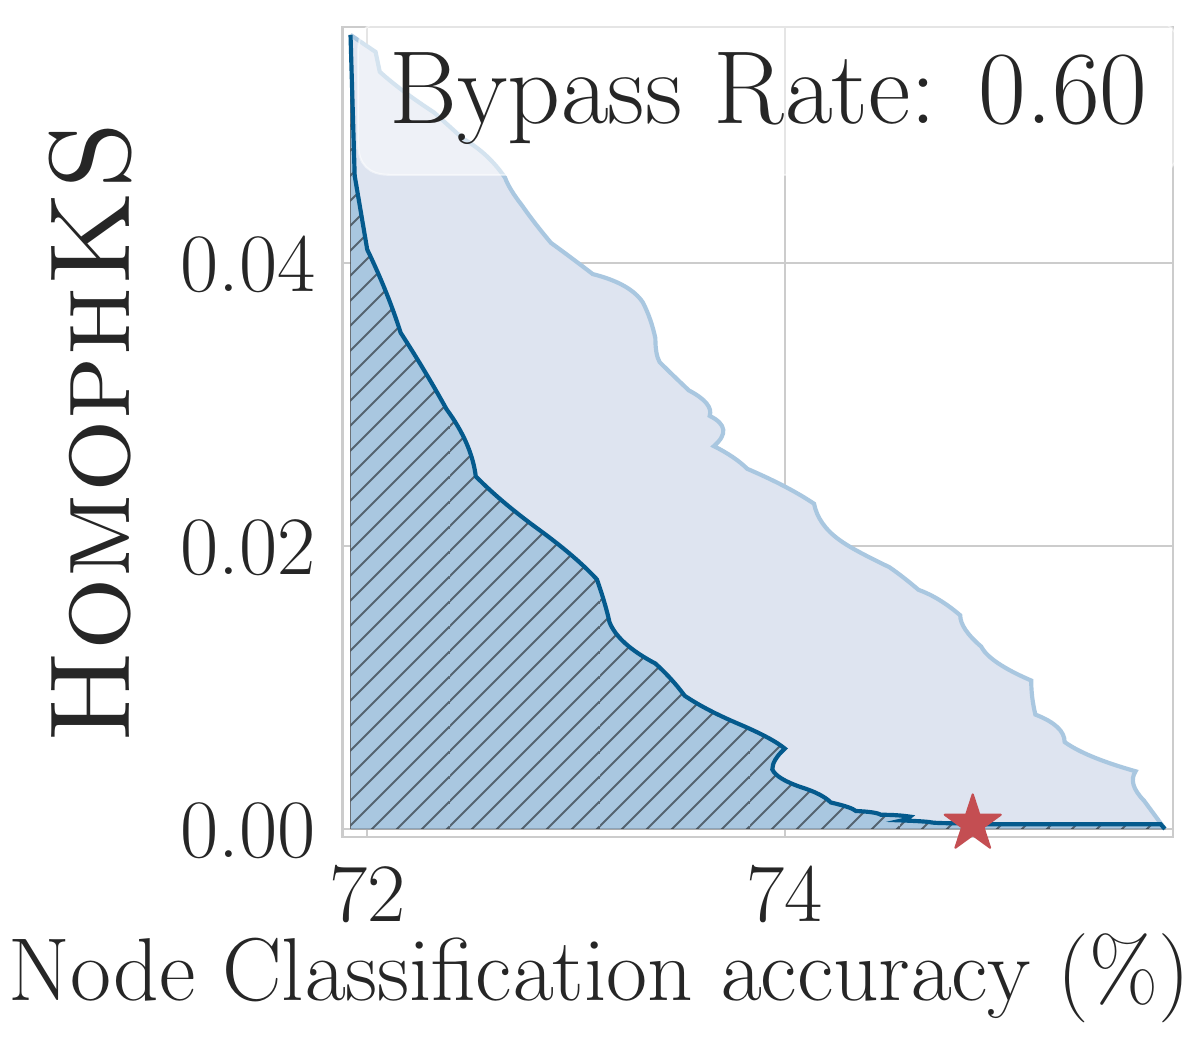} &
        \includegraphics[width=\linewidth]{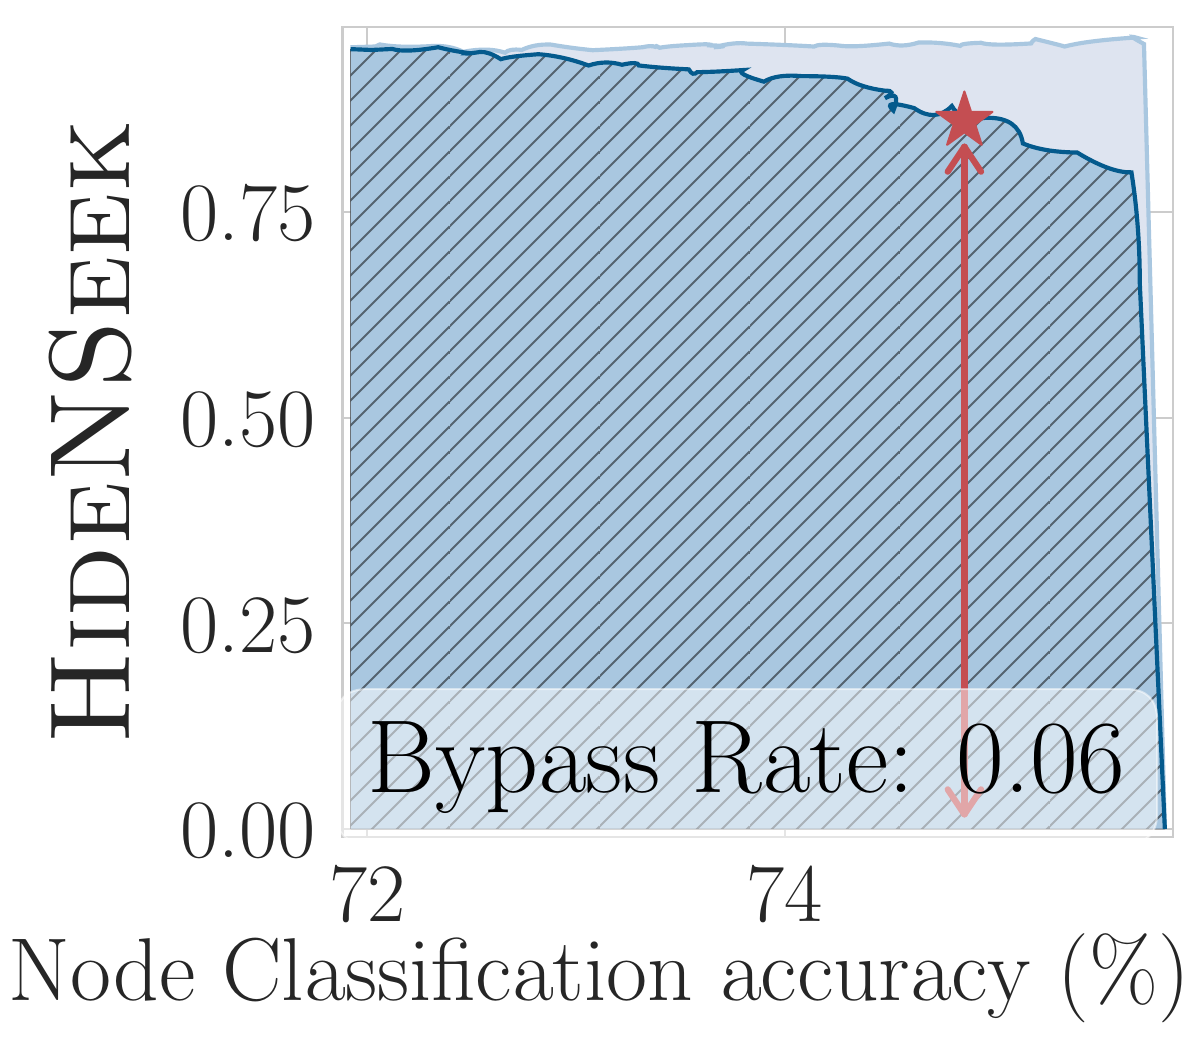} \\
        \hline
        \rotatebox[origin=c]{90}{\lastfmasia} & 
        \includegraphics[width=\linewidth]{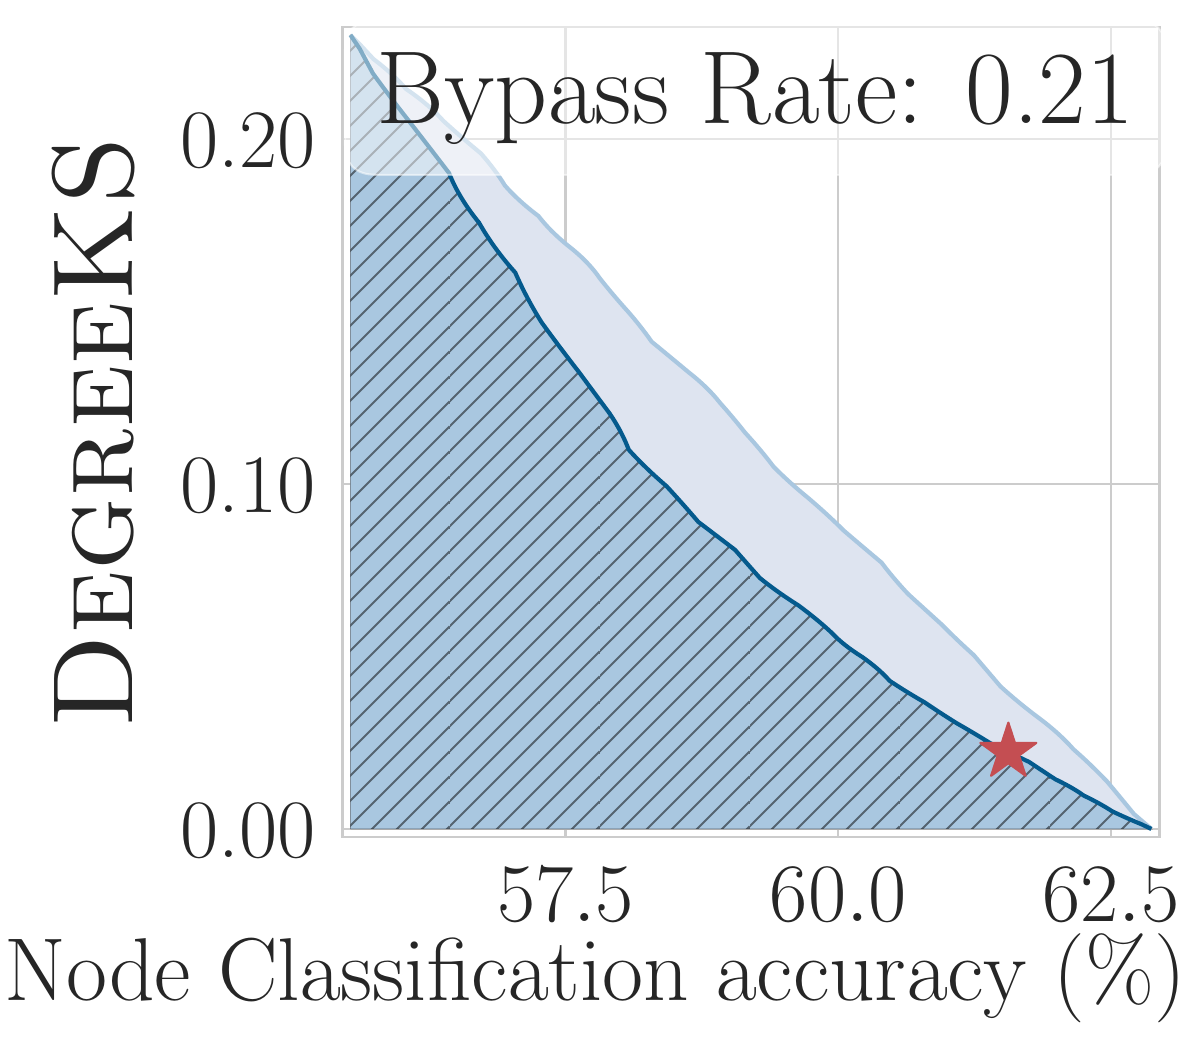} & 
        \includegraphics[width=\linewidth]{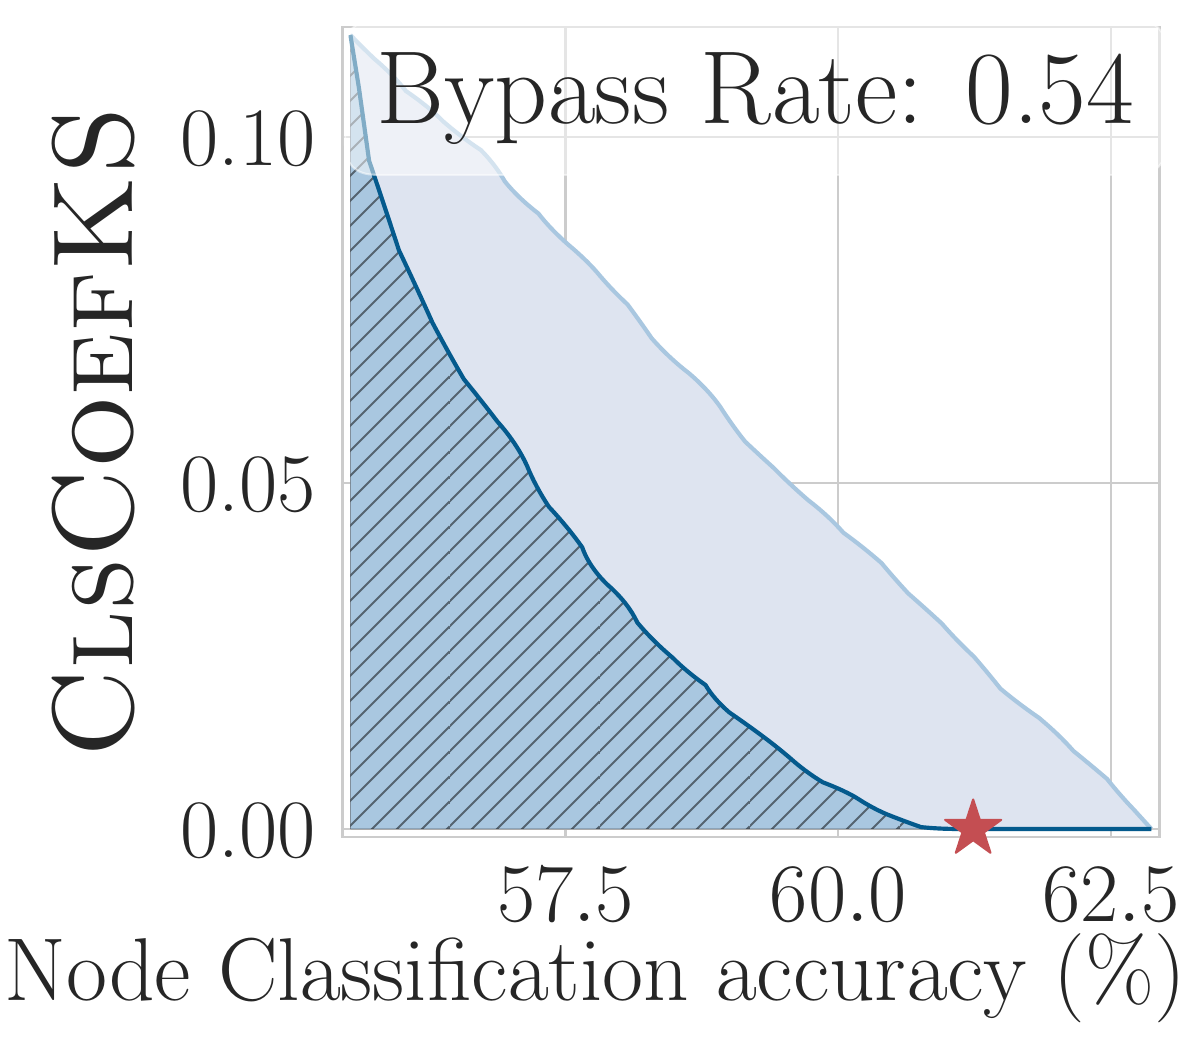} & 
        \includegraphics[width=\linewidth]{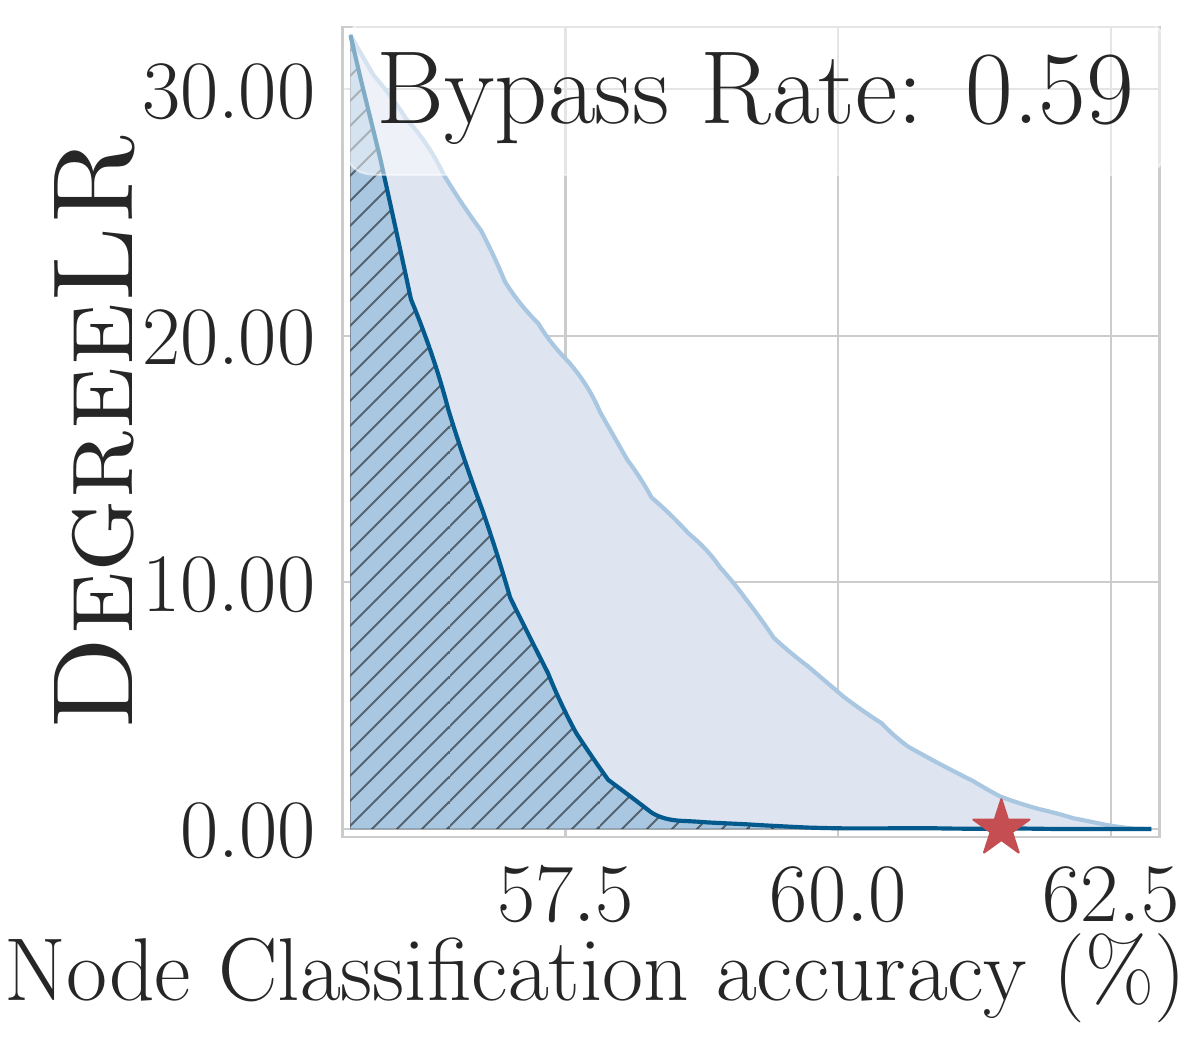} & 
        \includegraphics[width=\linewidth]{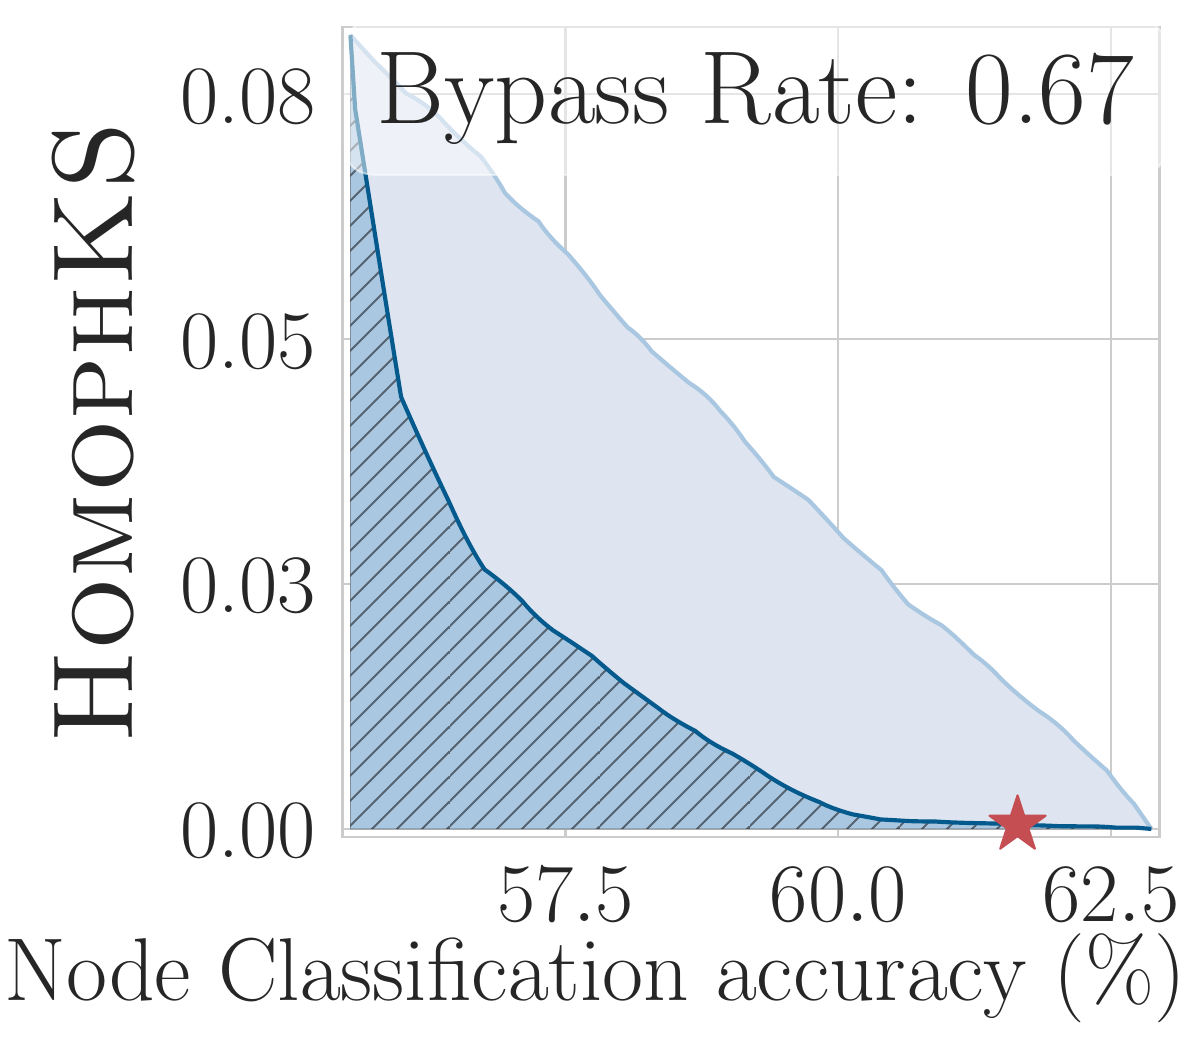} &
        \includegraphics[width=\linewidth]{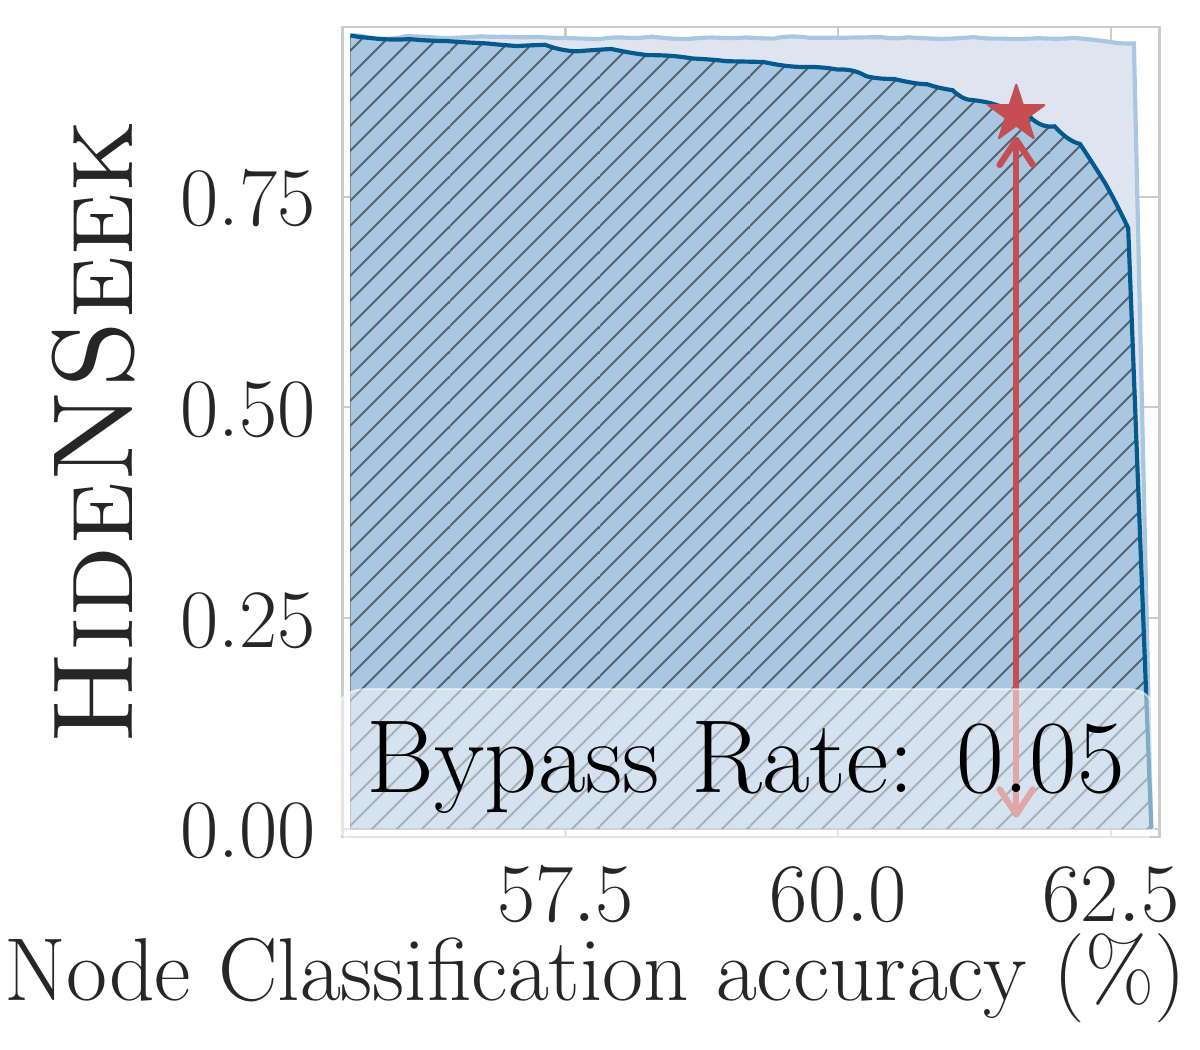} \\
        \hline
        % \rotatebox[origin=c]{90}{\chameleon} & 
        % \includegraphics[width=\linewidth]{FIG/EXP/chameleon/chameleon_structack_degree_q2.pdf} & 
        % \includegraphics[width=\linewidth]{FIG/EXP/chameleon/chameleon_structack_lc_q2.pdf} & 
        % \includegraphics[width=\linewidth]{FIG/EXP/chameleon/chameleon_structack_llr_q2.pdf} & 
        % \includegraphics[width=\linewidth]{FIG/EXP/chameleon/chameleon_structack_homophily_q2.pdf} &
        % \includegraphics[width=\linewidth]{FIG/EXP/chameleon/chameleon_structack_our_q2.pdf} \\
        % \hline
        % \rotatebox[origin=c]{90}{\squirrel} & 
        % \includegraphics[width=\linewidth]{FIG/EXP/squirrel/squirrel_structack_degree_q2.pdf} & 
        % \includegraphics[width=\linewidth]{FIG/EXP/squirrel/squirrel_structack_lc_q2.pdf} & 
        % \includegraphics[width=\linewidth]{FIG/EXP/squirrel/squirrel_structack_llr_q2.pdf} & 
        % \includegraphics[width=\linewidth]{FIG/EXP/squirrel/squirrel_structack_homophily_q2.pdf} &
        % \includegraphics[width=\linewidth]{FIG/EXP/squirrel/squirrel_structack_our_q2.pdf} \\
        % \hline
    \end{tabular}
    }
    \label{tab:exp:q2_structack}
\end{table*}

\newcolumntype{C}{>{\centering\arraybackslash}m{0.15\linewidth}}
\begin{table*}
    \centering
    \caption{The additional experimental results regarding Q2 \& Q3  on \metattack.}
    \resizebox{0.8\textwidth}{!}{
    \begin{tabular}{l||C|C|C|C||C}
        \hline
        % & \multicolumn{4}{c||}{Existing Measures} & \multirow{3}{*}{\textbf{\measure}} \\ 
        % \cline{2-5}
        % & Degree Dist. & Clustering Coeff. & Degree Dist. & Homophily Dist. & \\
        % & (KS test) & (KS test) & (LR test)& (KS test) & \\
        & \textsc{DegreeKS} & \textsc{ClsCoefKS} & \textsc{DegreeLR} & \textsc{HomophKS} & \textbf{\measure} \\
        \hline\hline
        \rotatebox[origin=c]{90}{\cora} & 
        \includegraphics[width=\linewidth]{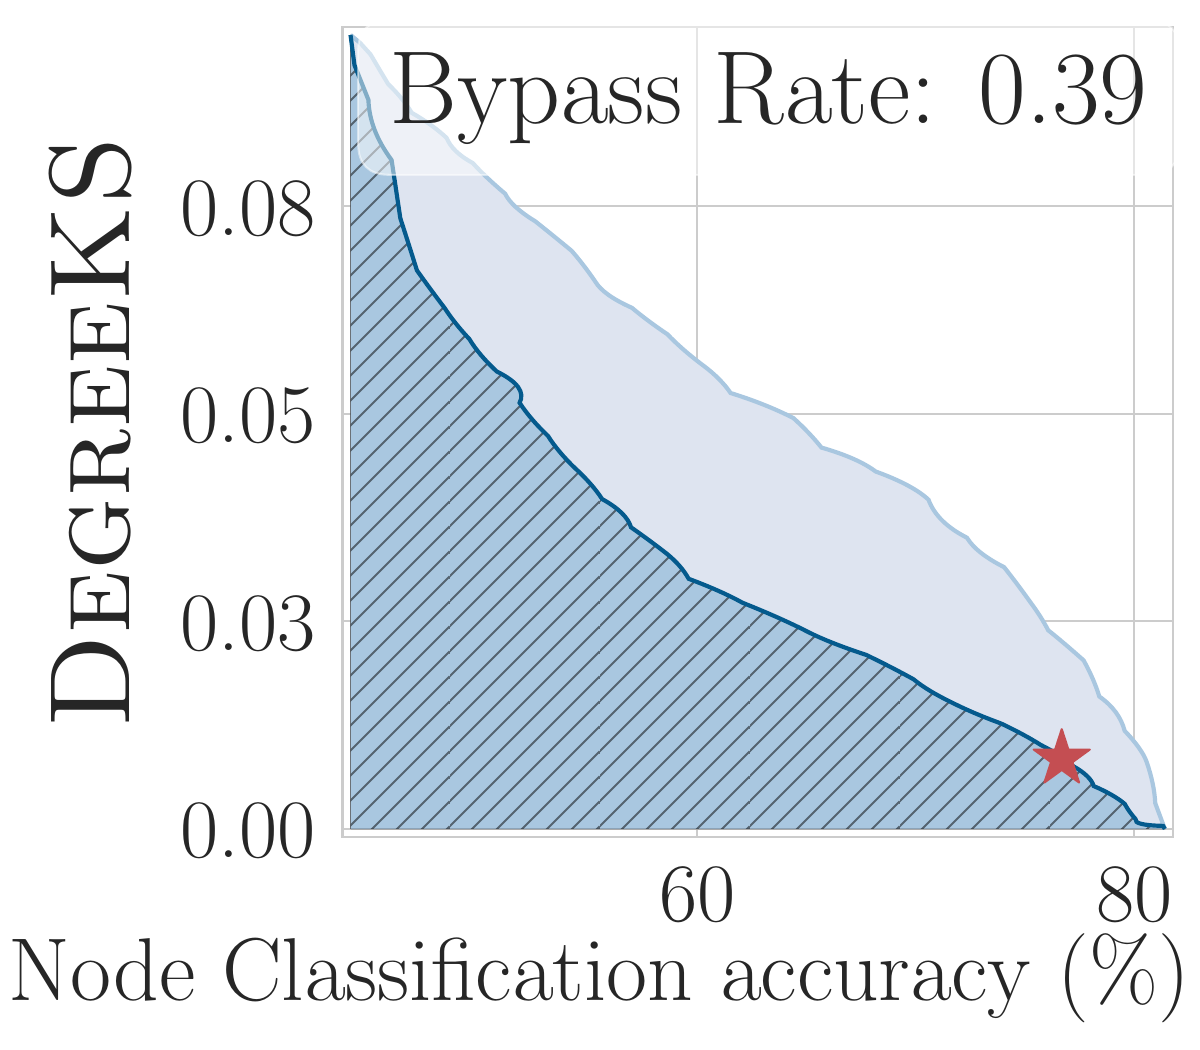} & 
        \includegraphics[width=\linewidth]{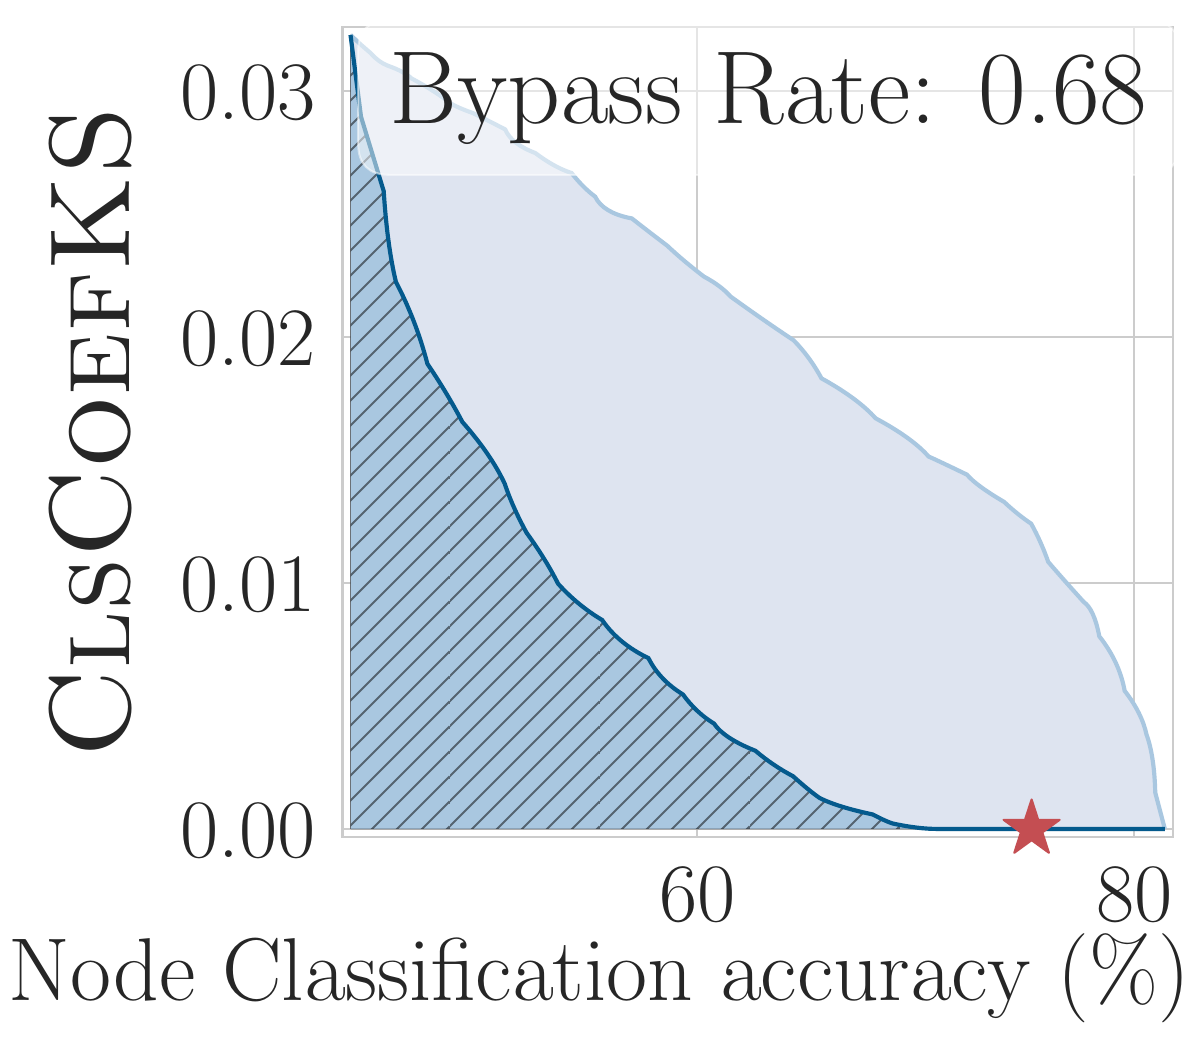} & 
        \includegraphics[width=\linewidth]{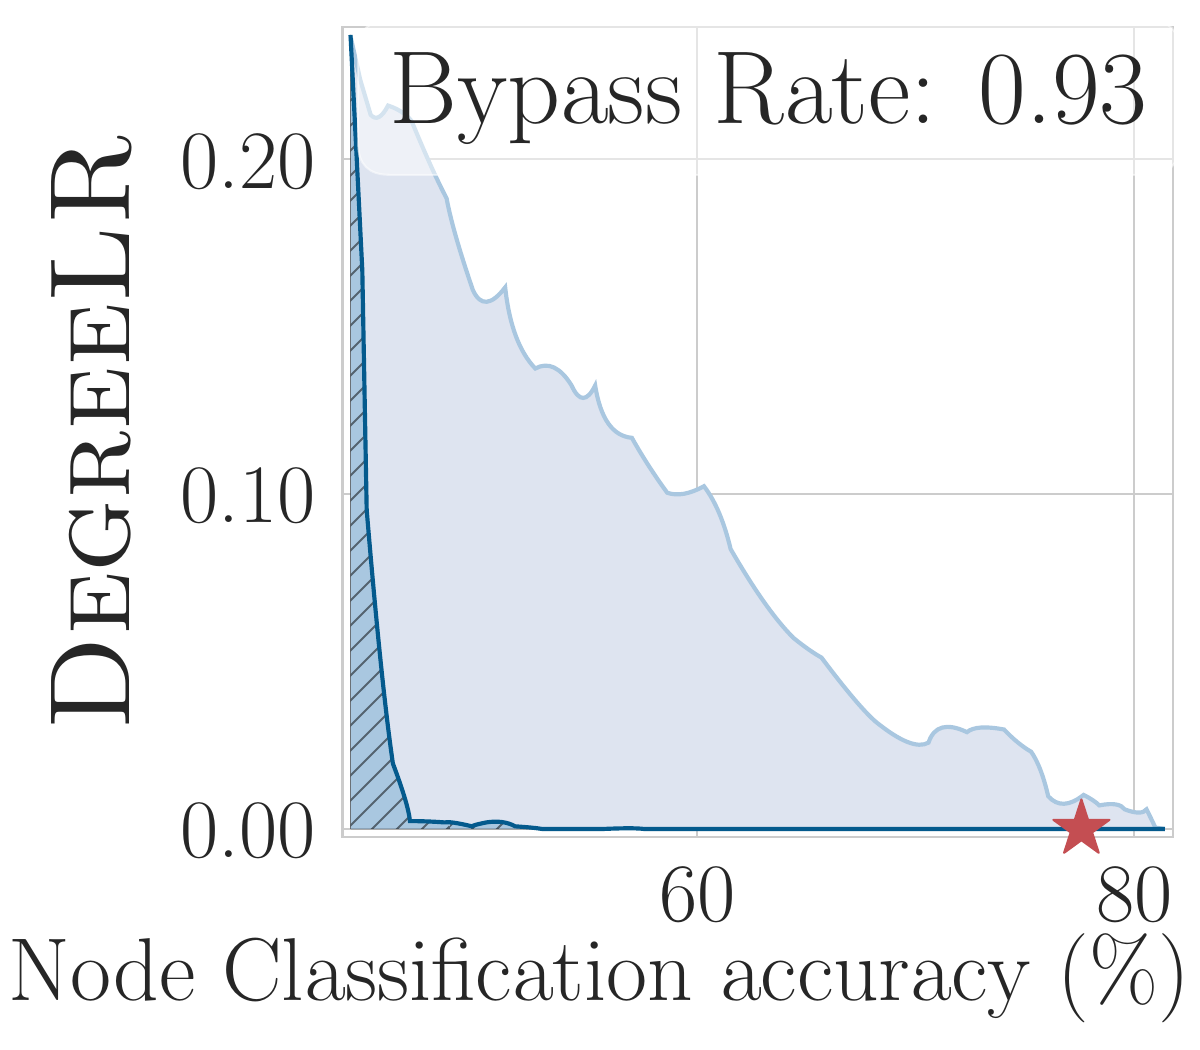} & 
        \includegraphics[width=\linewidth]{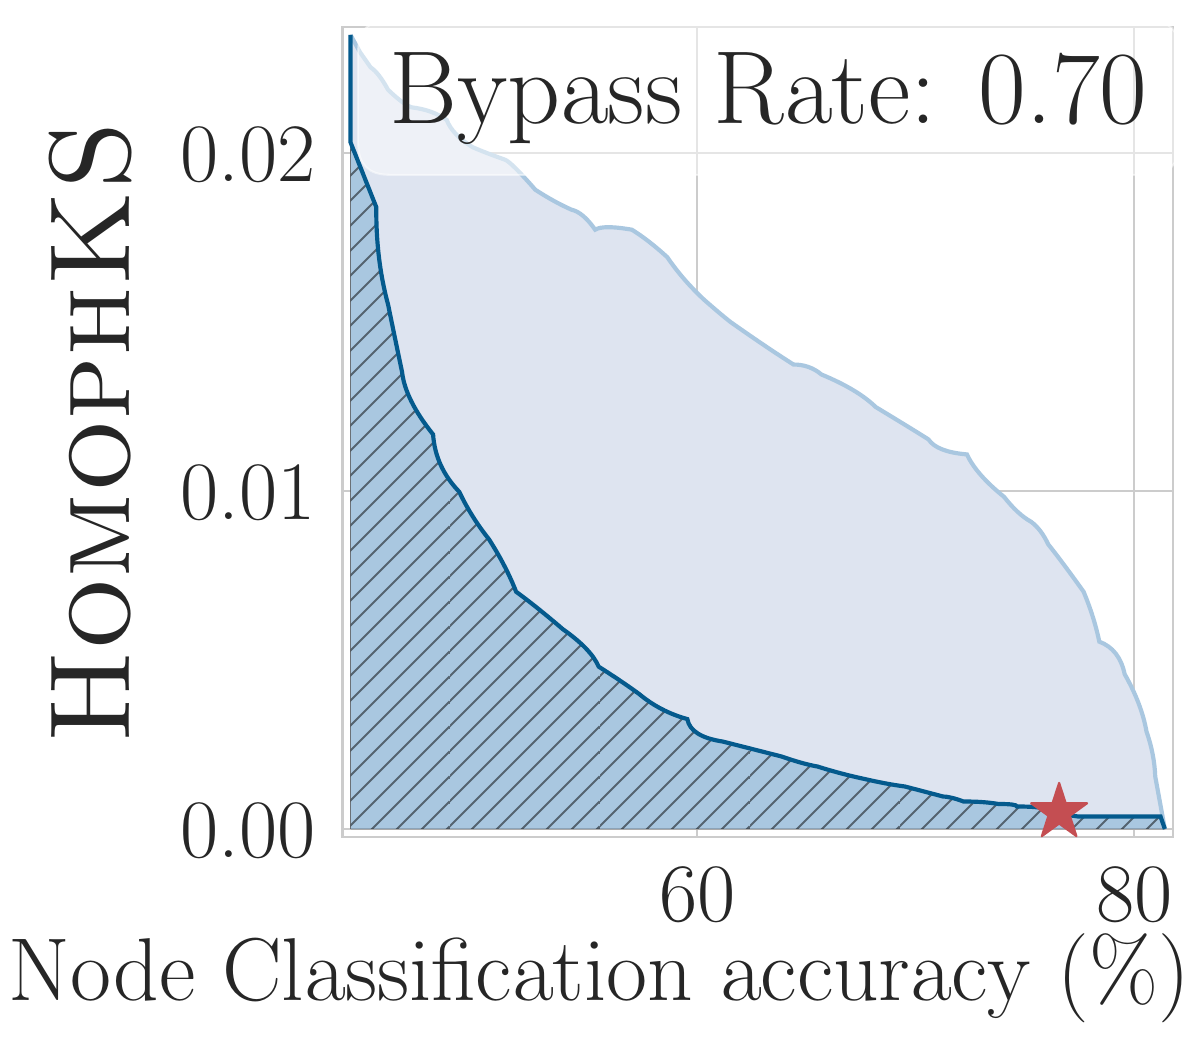} &
        \includegraphics[width=\linewidth]{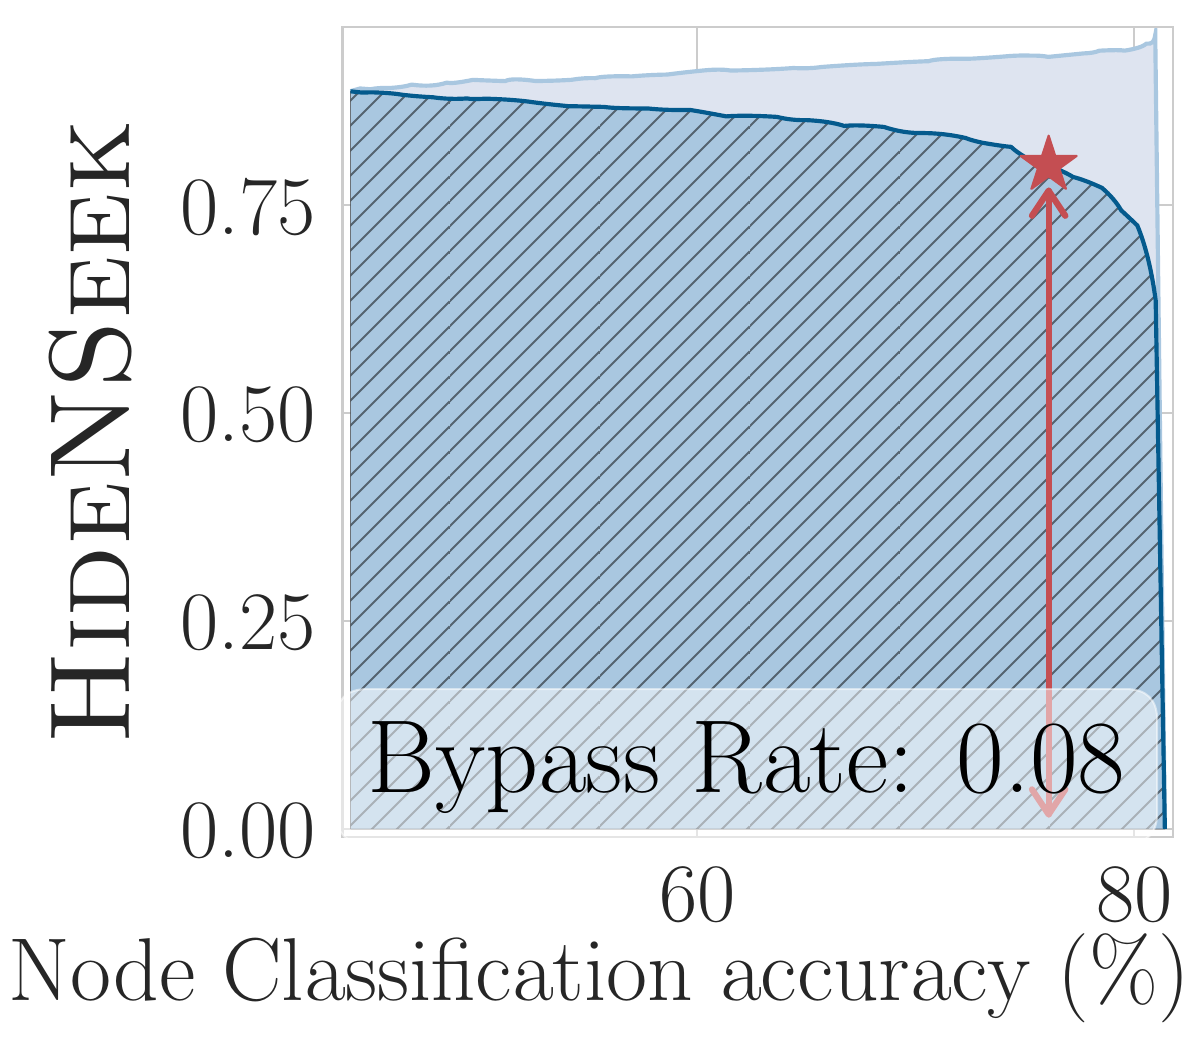} \\
        \hline
        \rotatebox[origin=c]{90}{\citeseer} & 
        \includegraphics[width=\linewidth]{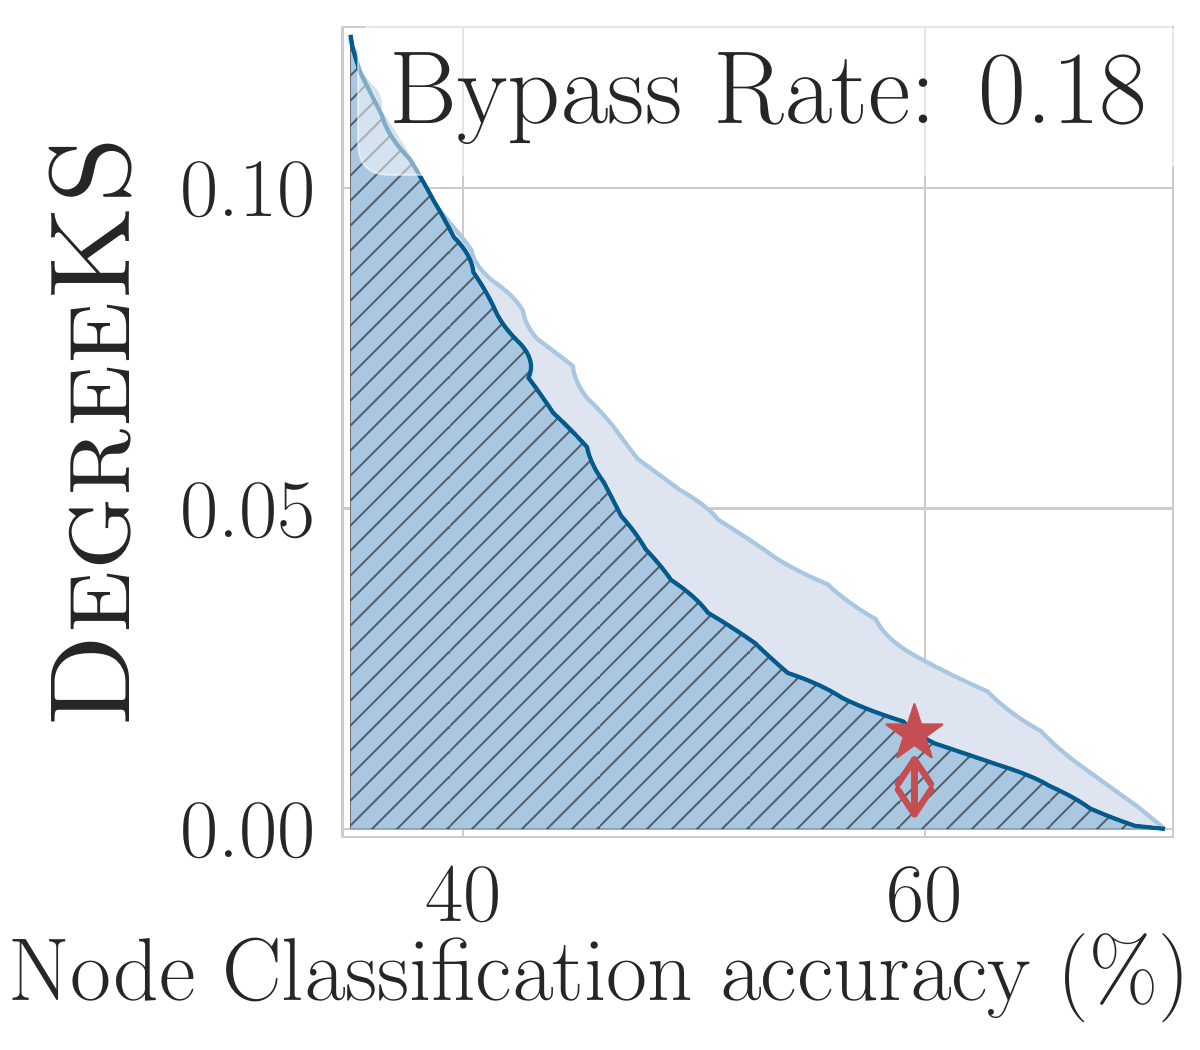} & 
        \includegraphics[width=\linewidth]{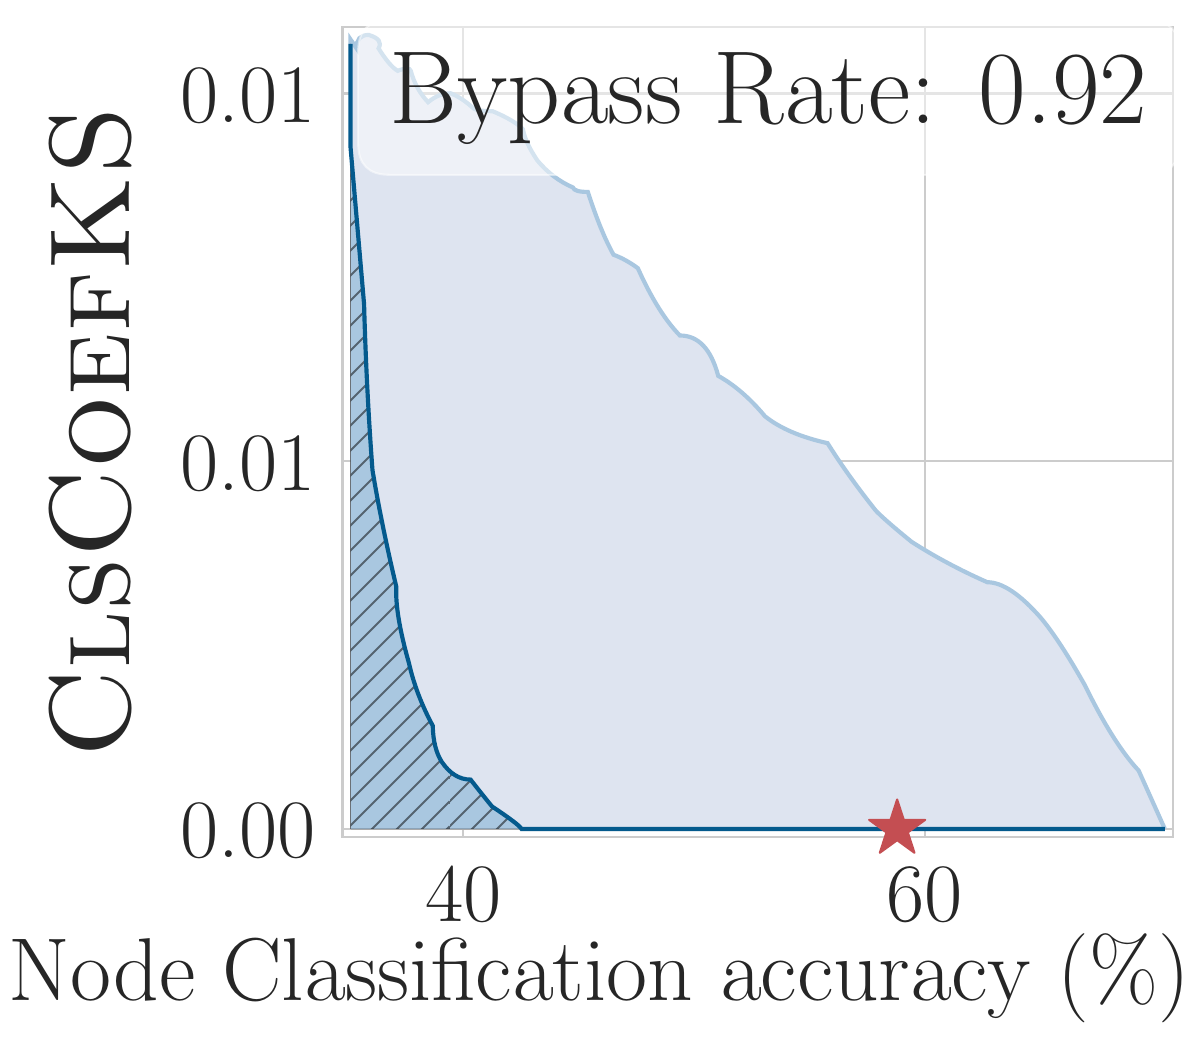} & 
        \includegraphics[width=\linewidth]{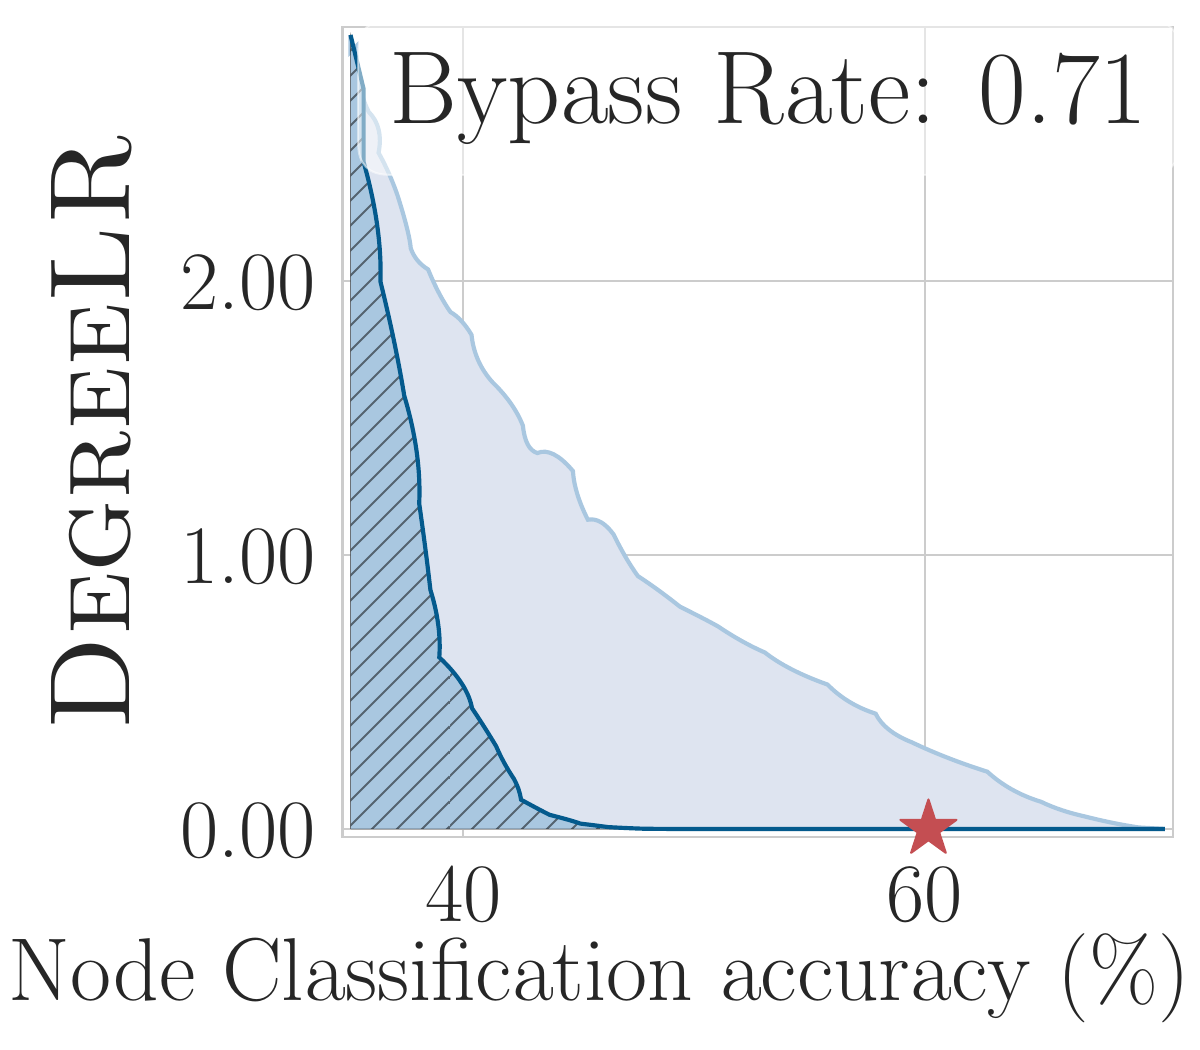} & 
        \includegraphics[width=\linewidth]{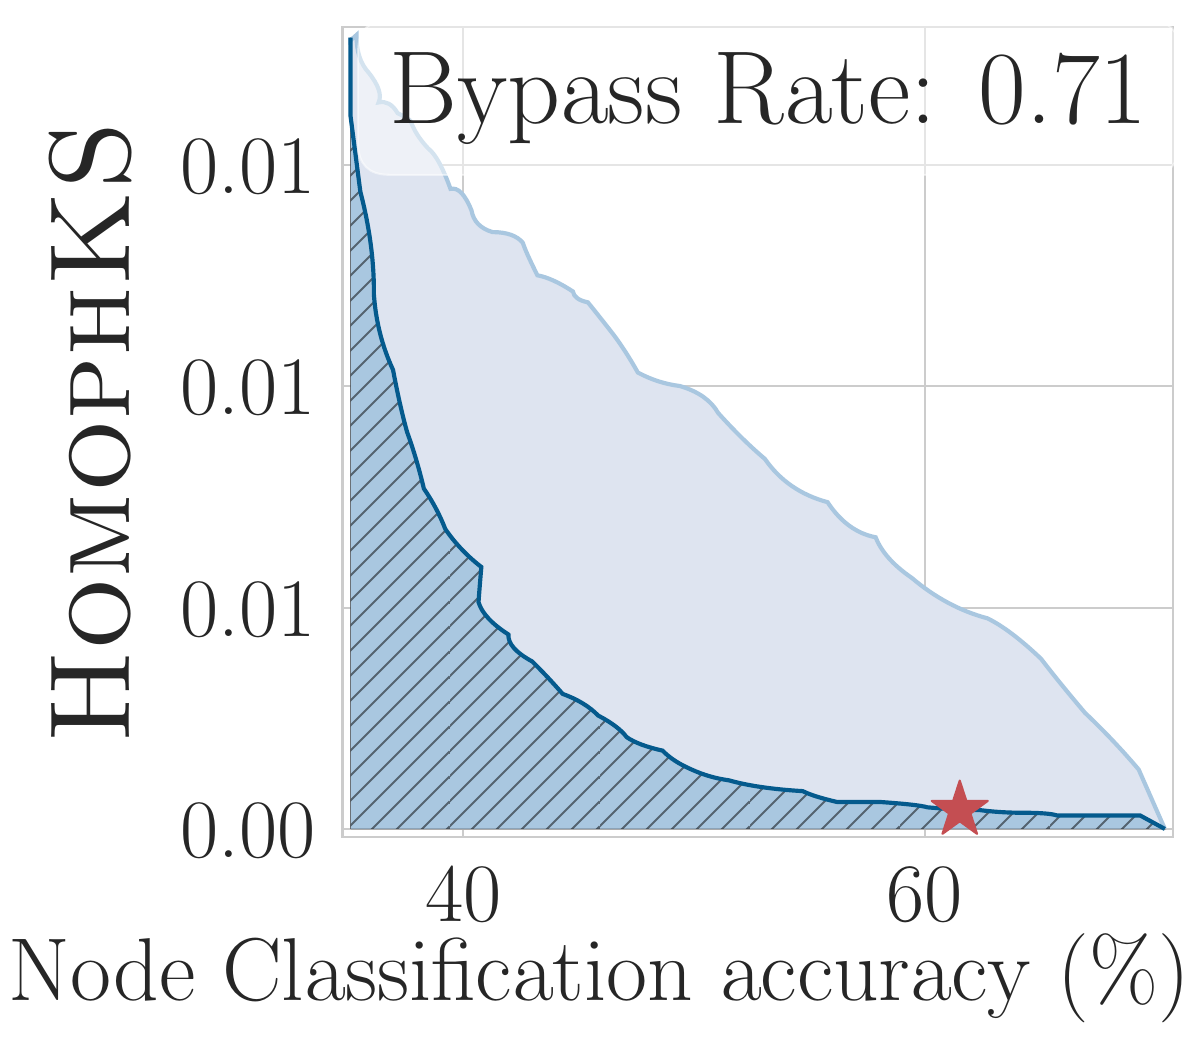} &
        \includegraphics[width=\linewidth]{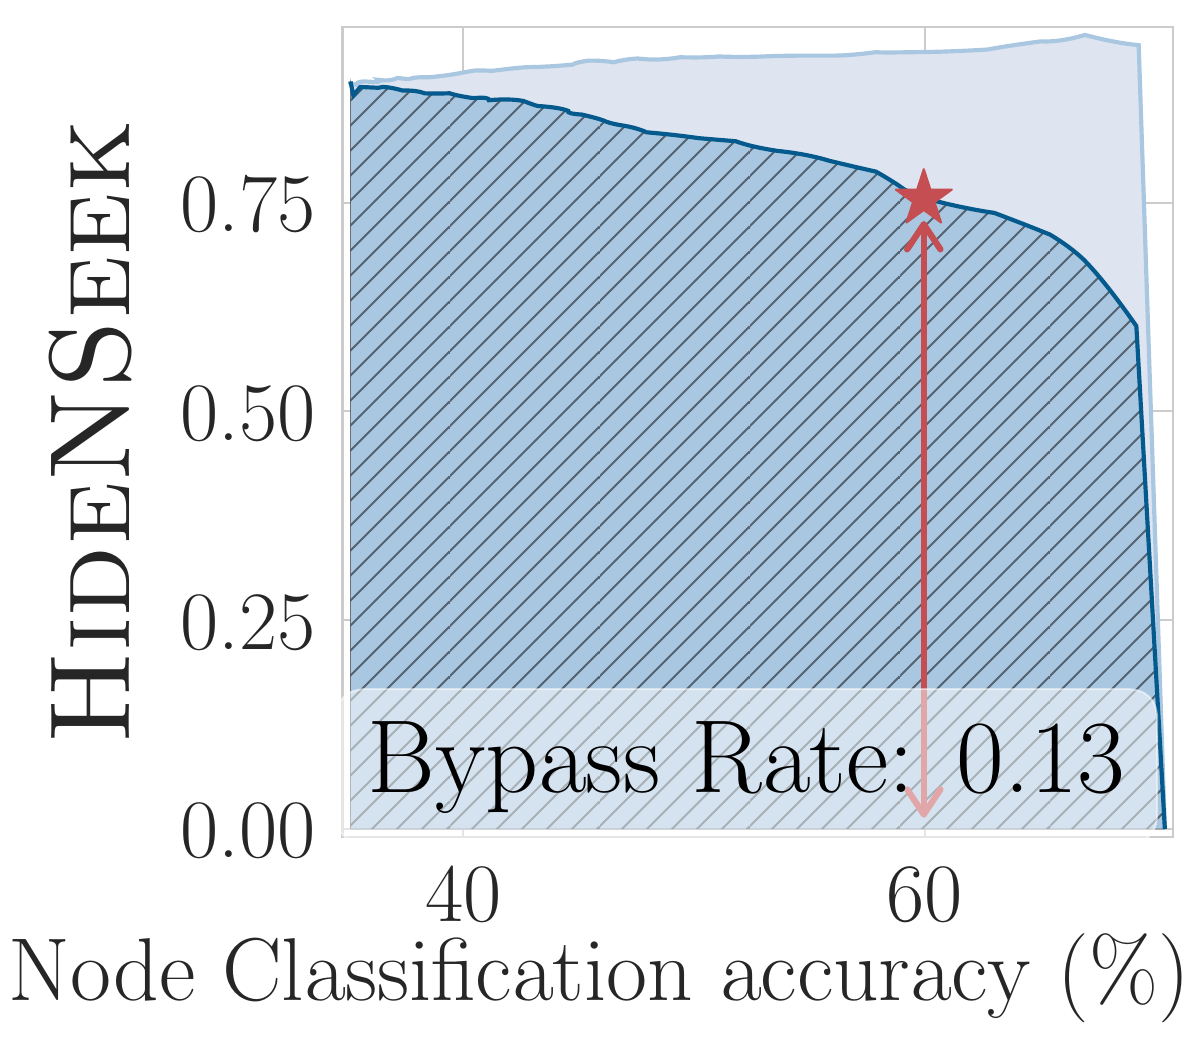} \\
        \hline
        \rotatebox[origin=c]{90}{\coraml} & 
        \includegraphics[width=\linewidth]{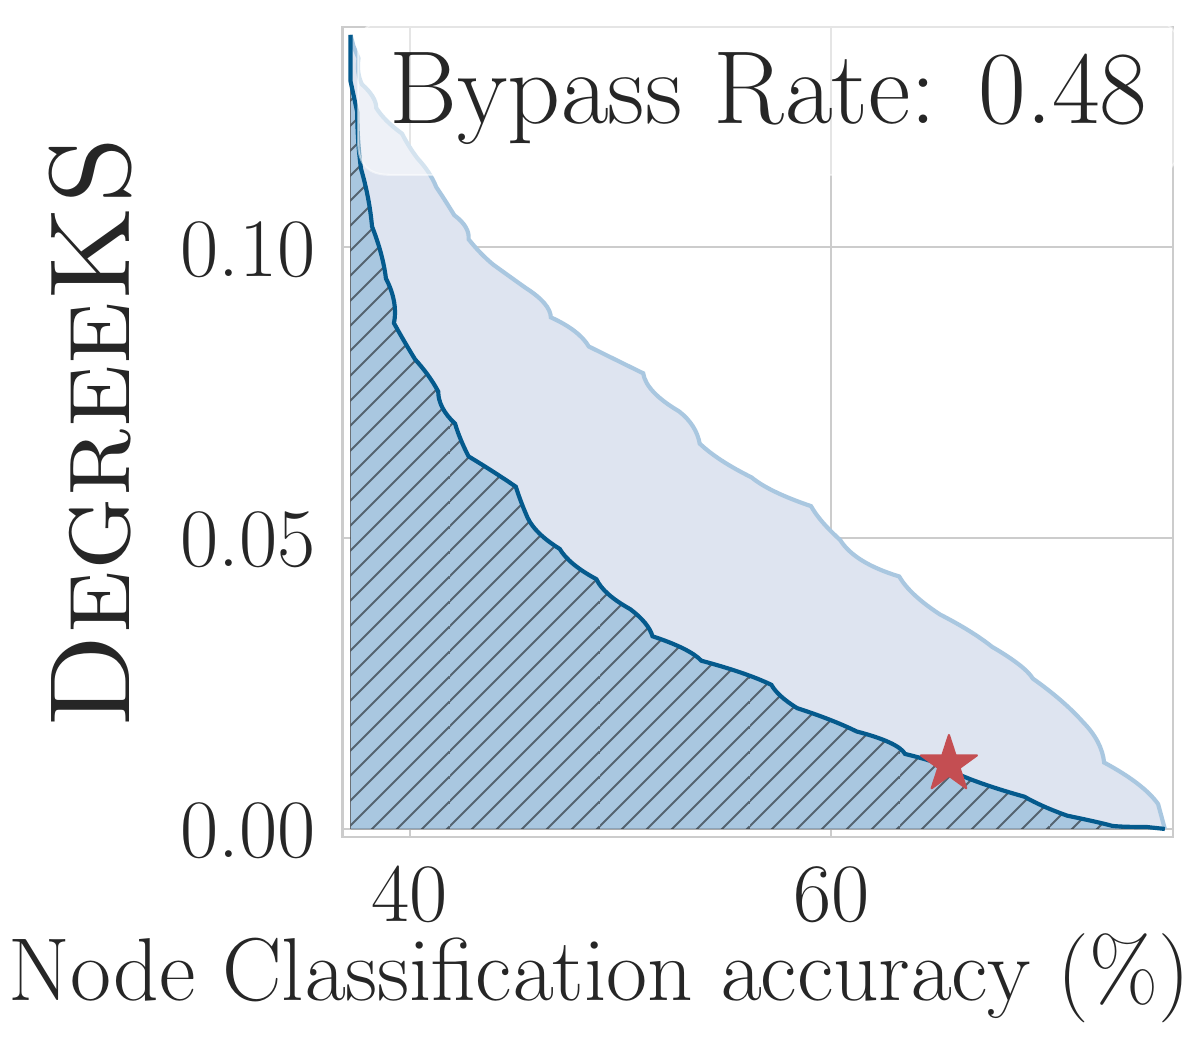} & 
        \includegraphics[width=\linewidth]{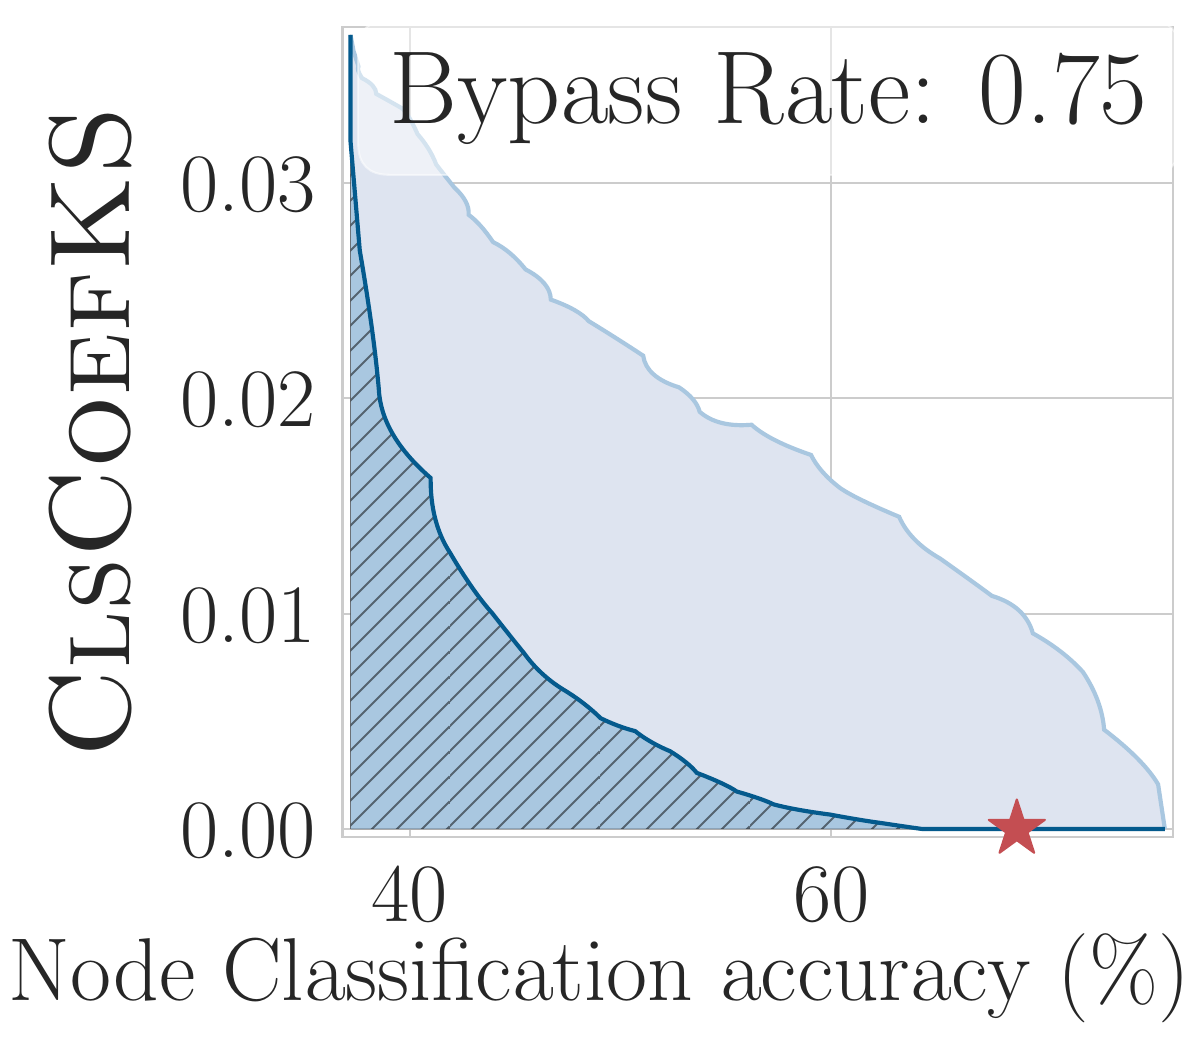} & 
        \includegraphics[width=\linewidth]{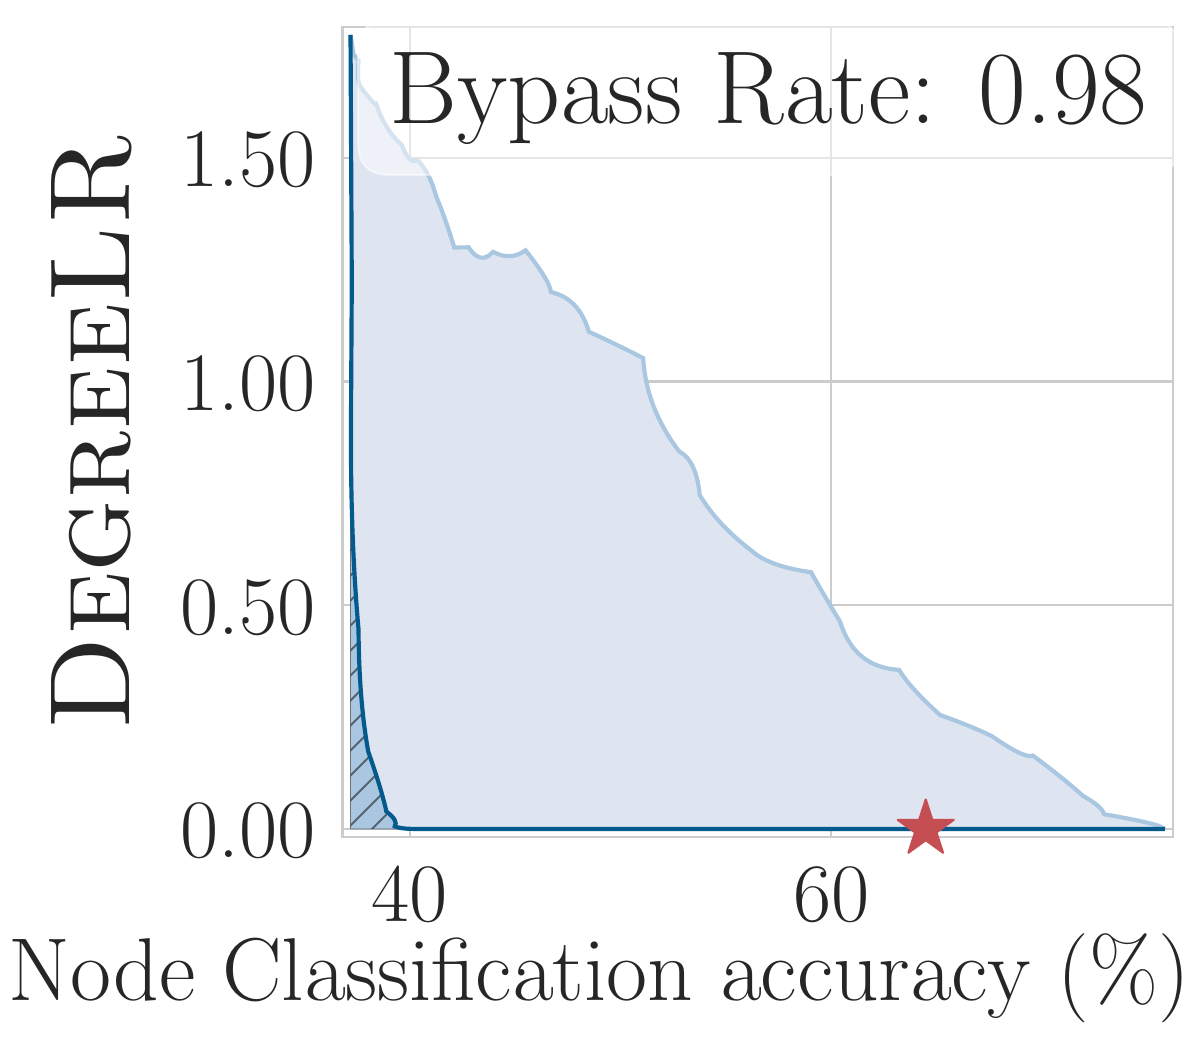} & 
        \includegraphics[width=\linewidth]{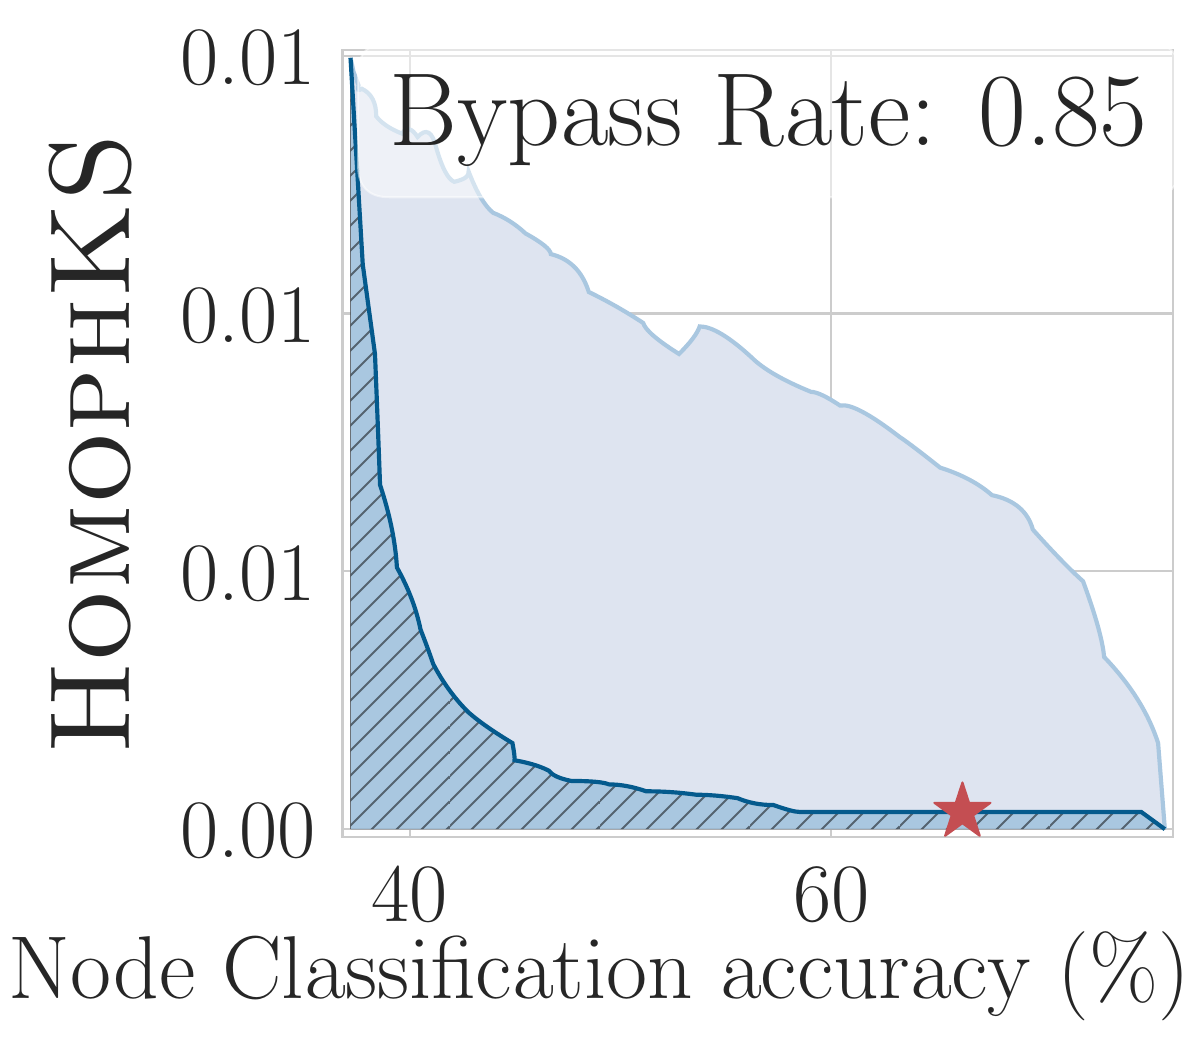} &
        \includegraphics[width=\linewidth]{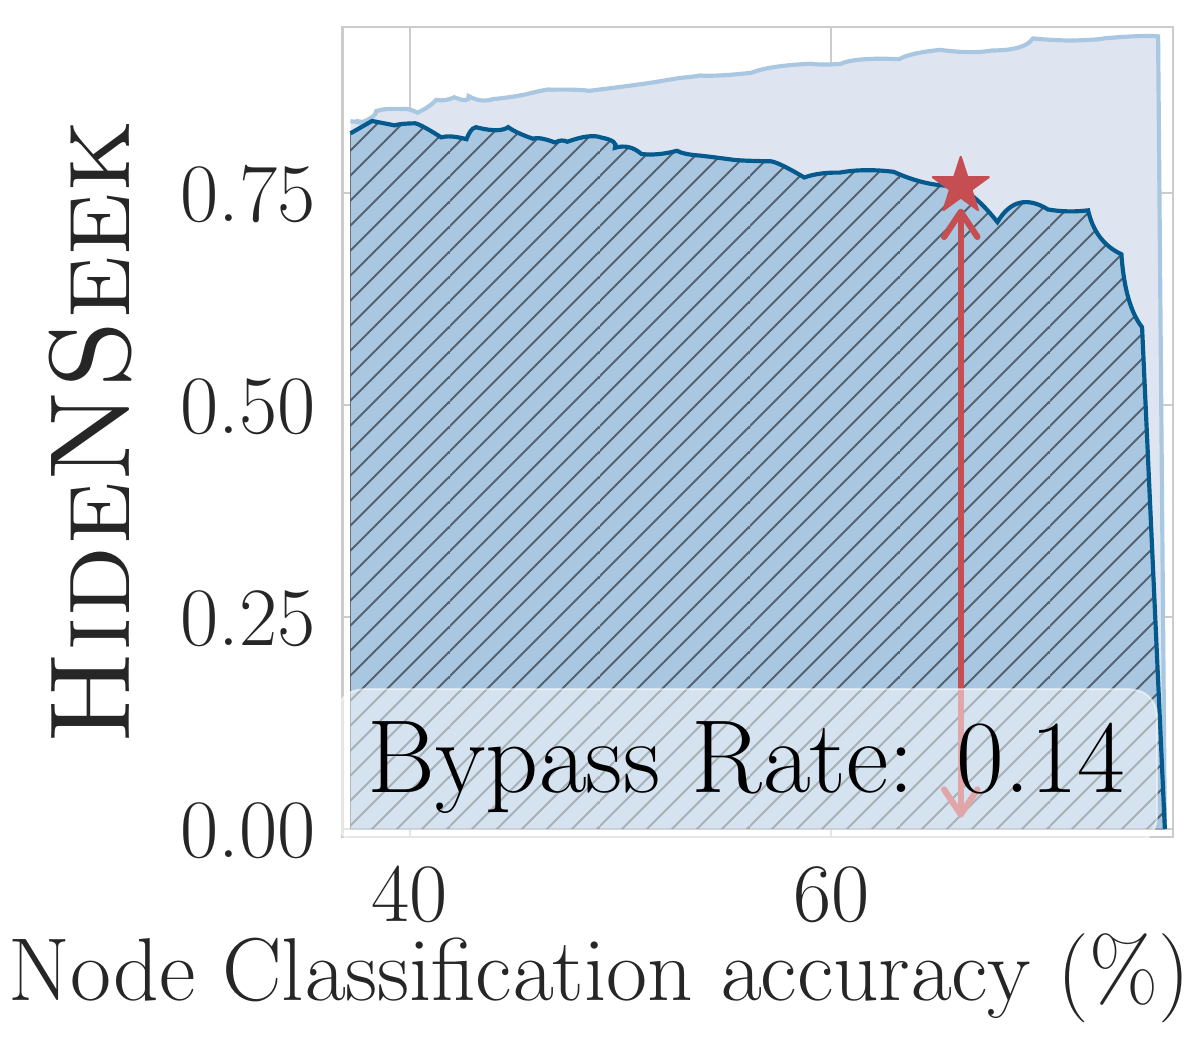} \\
        \hline
        % \rotatebox[origin=c]{90}{\lastfmasia} & 
        % \includegraphics[width=\linewidth]{FIG/EXP/lastfmasia/lastfmasia_metattack_degree_q2.pdf} & 
        % \includegraphics[width=\linewidth]{FIG/EXP/lastfmasia/lastfmasia_metattack_lc_q2.pdf} & 
        % \includegraphics[width=\linewidth]{FIG/EXP/lastfmasia/lastfmasia_metattack_llr_q2.pdf} & 
        % \includegraphics[width=\linewidth]{FIG/EXP/lastfmasia/lastfmasia_metattack_homophily_q2.pdf} &
        % \includegraphics[width=\linewidth]{FIG/EXP/lastfmasia/lastfmasia_metattack_our_q2.pdf} \\
        % \hline
        \rotatebox[origin=c]{90}{\chameleon} & 
        \includegraphics[width=\linewidth]{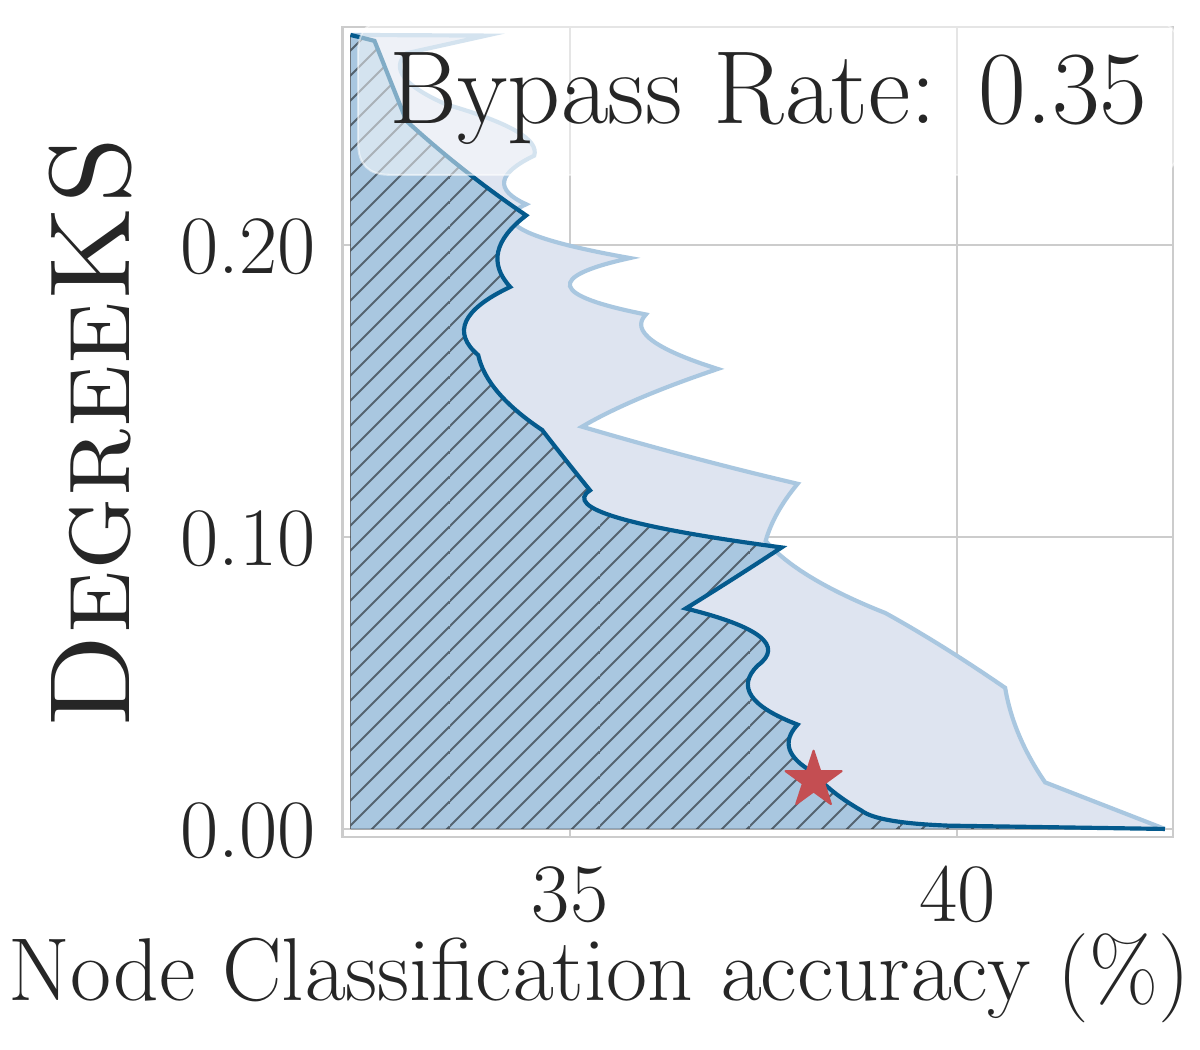} & 
        \includegraphics[width=\linewidth]{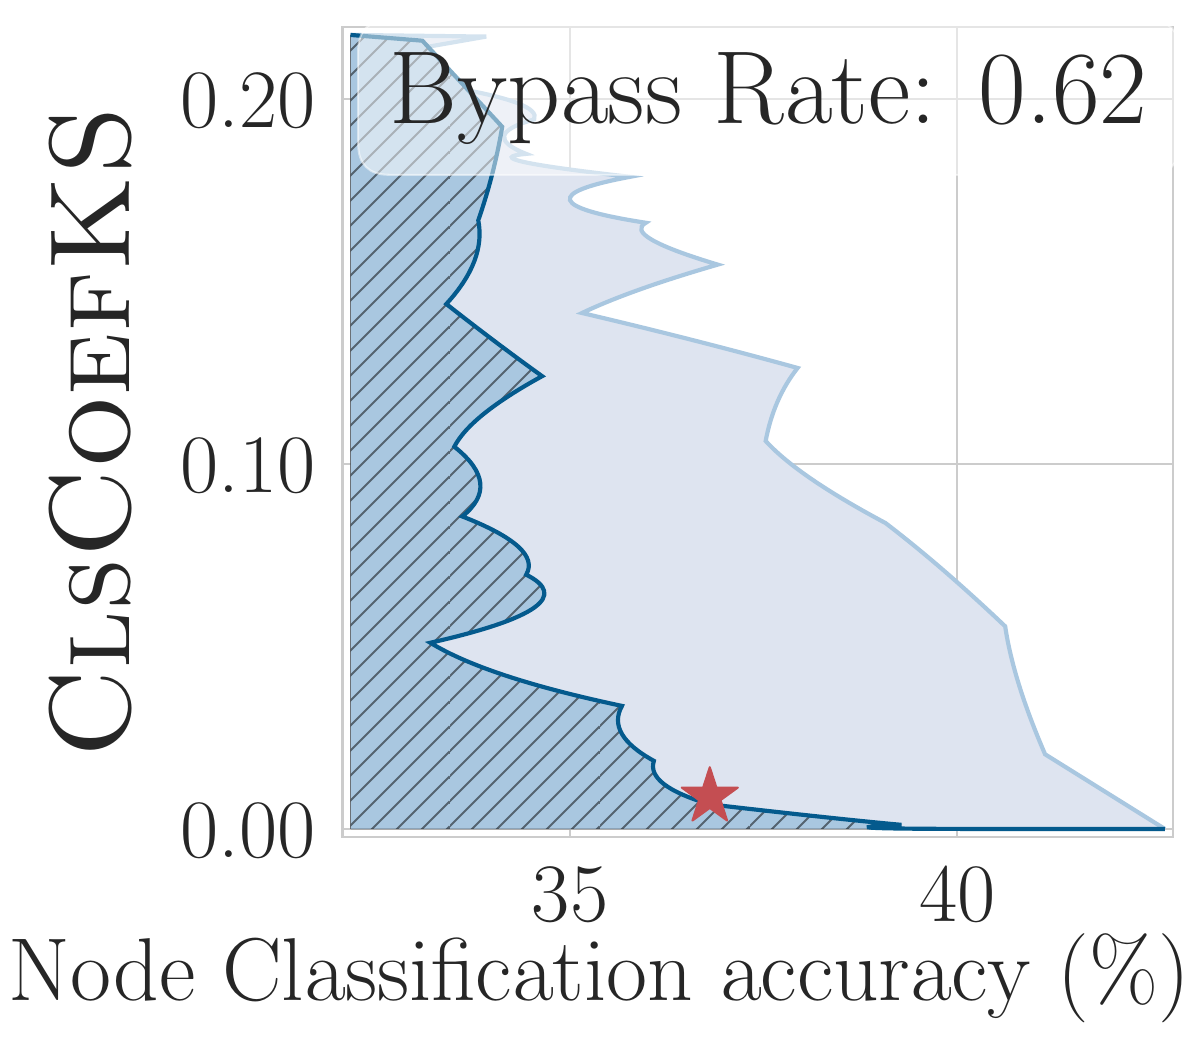} & 
        \includegraphics[width=\linewidth]{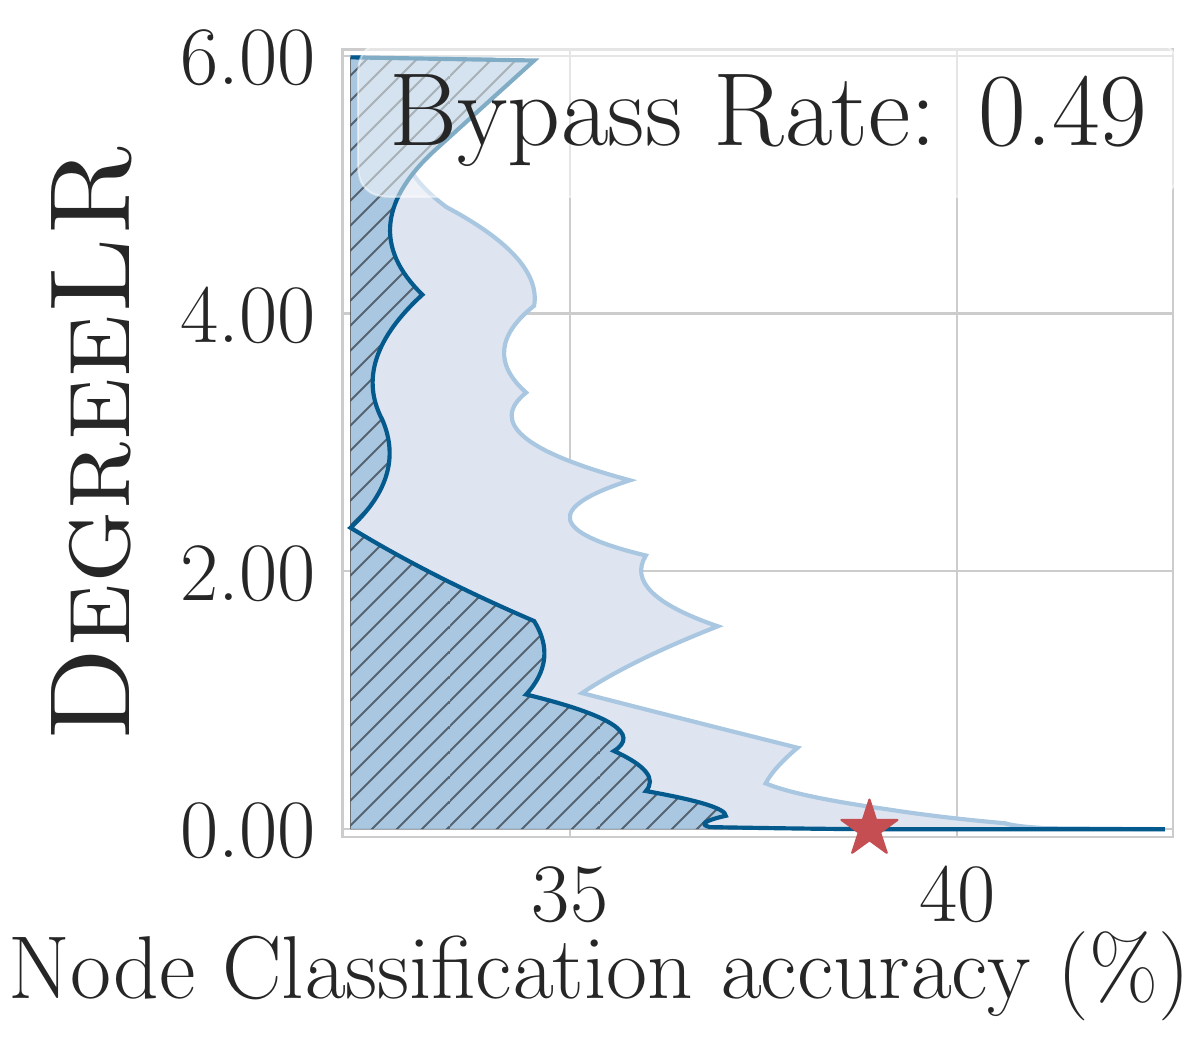} & 
        \includegraphics[width=\linewidth]{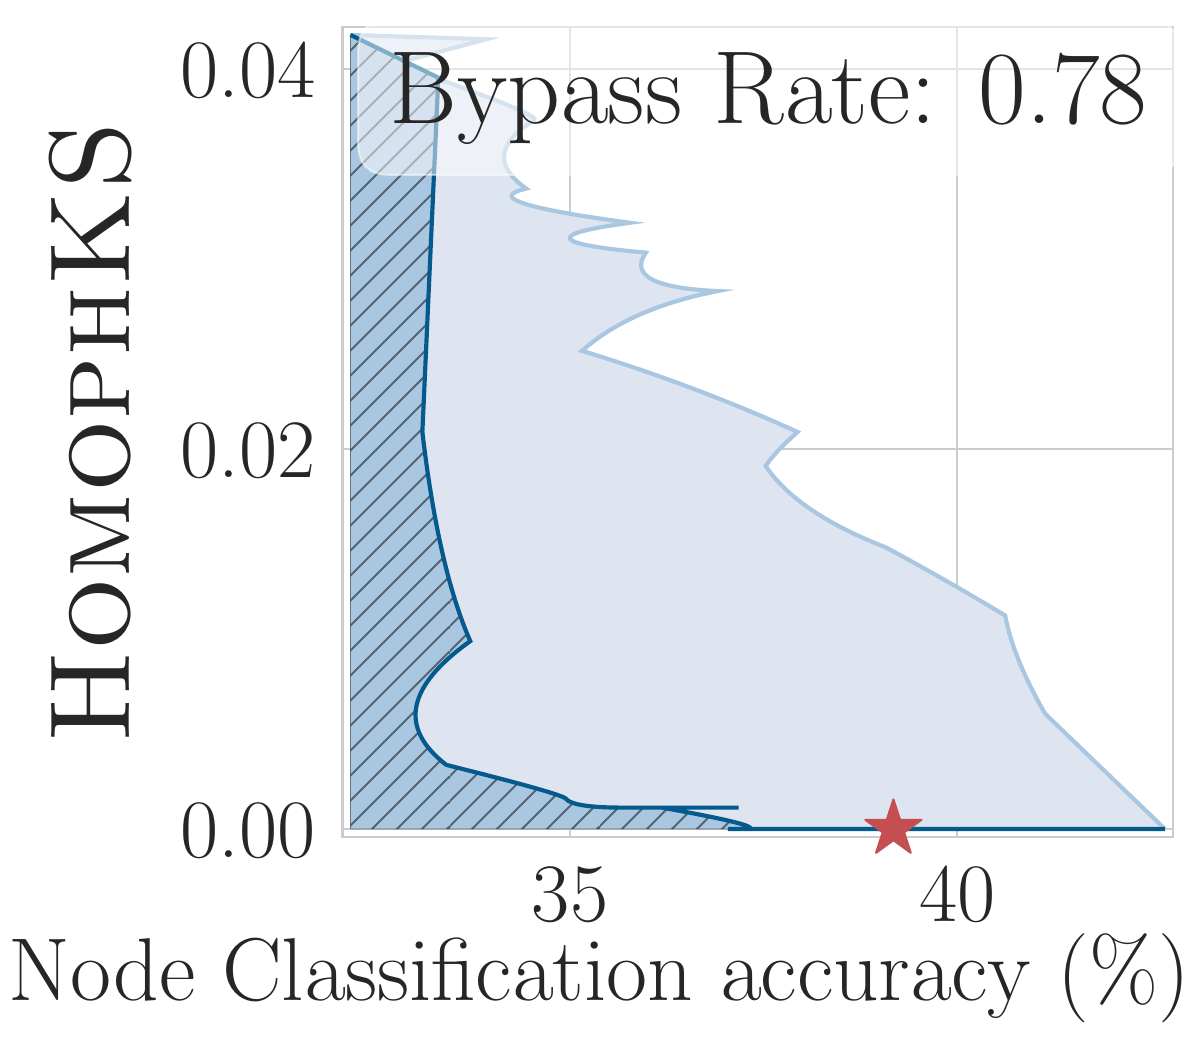} &
        \includegraphics[width=\linewidth]{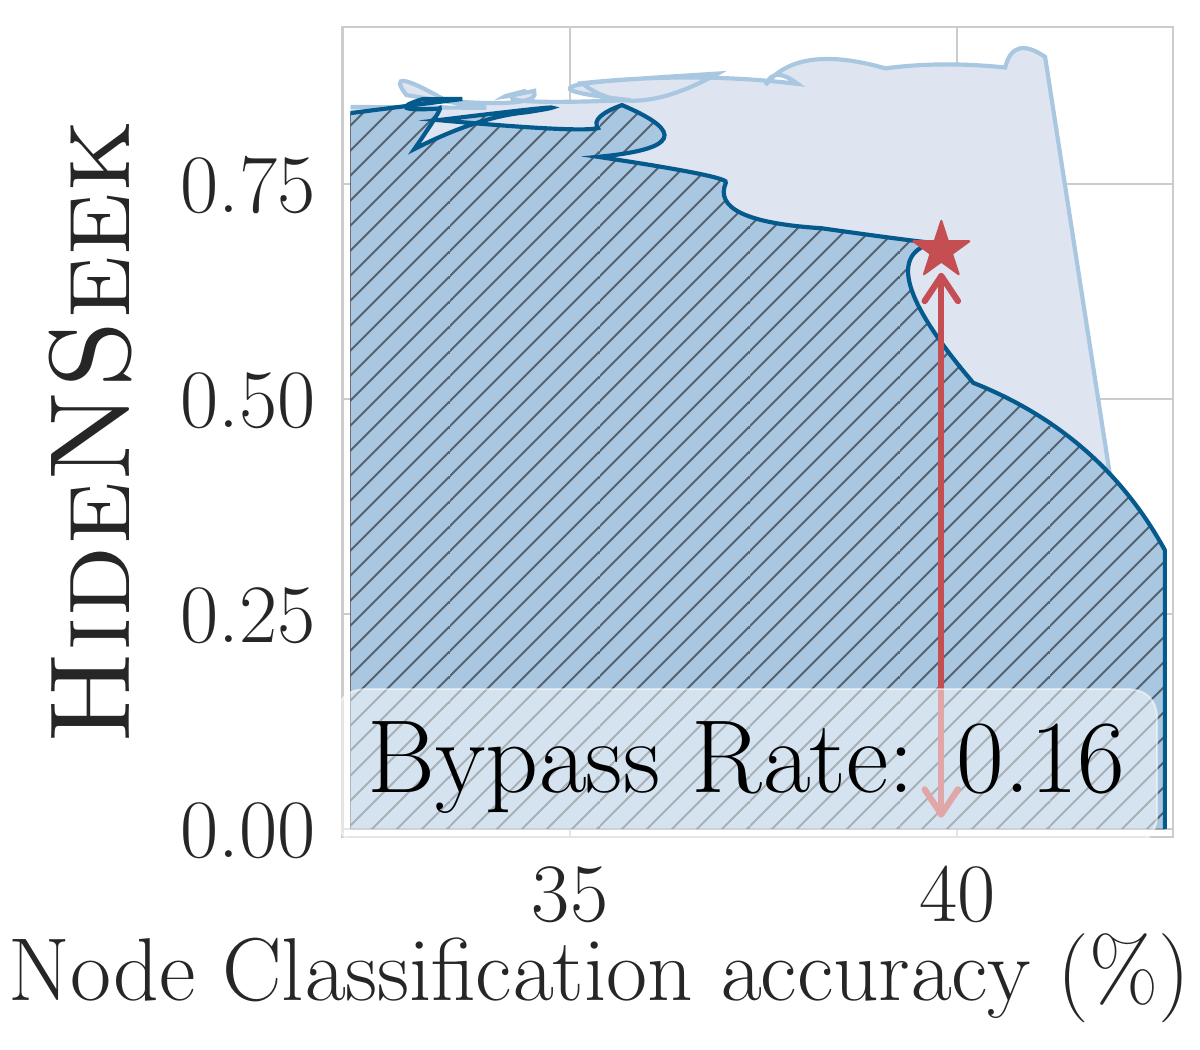} \\
        \hline
        \rotatebox[origin=c]{90}{\squirrel} & 
        \includegraphics[width=\linewidth]{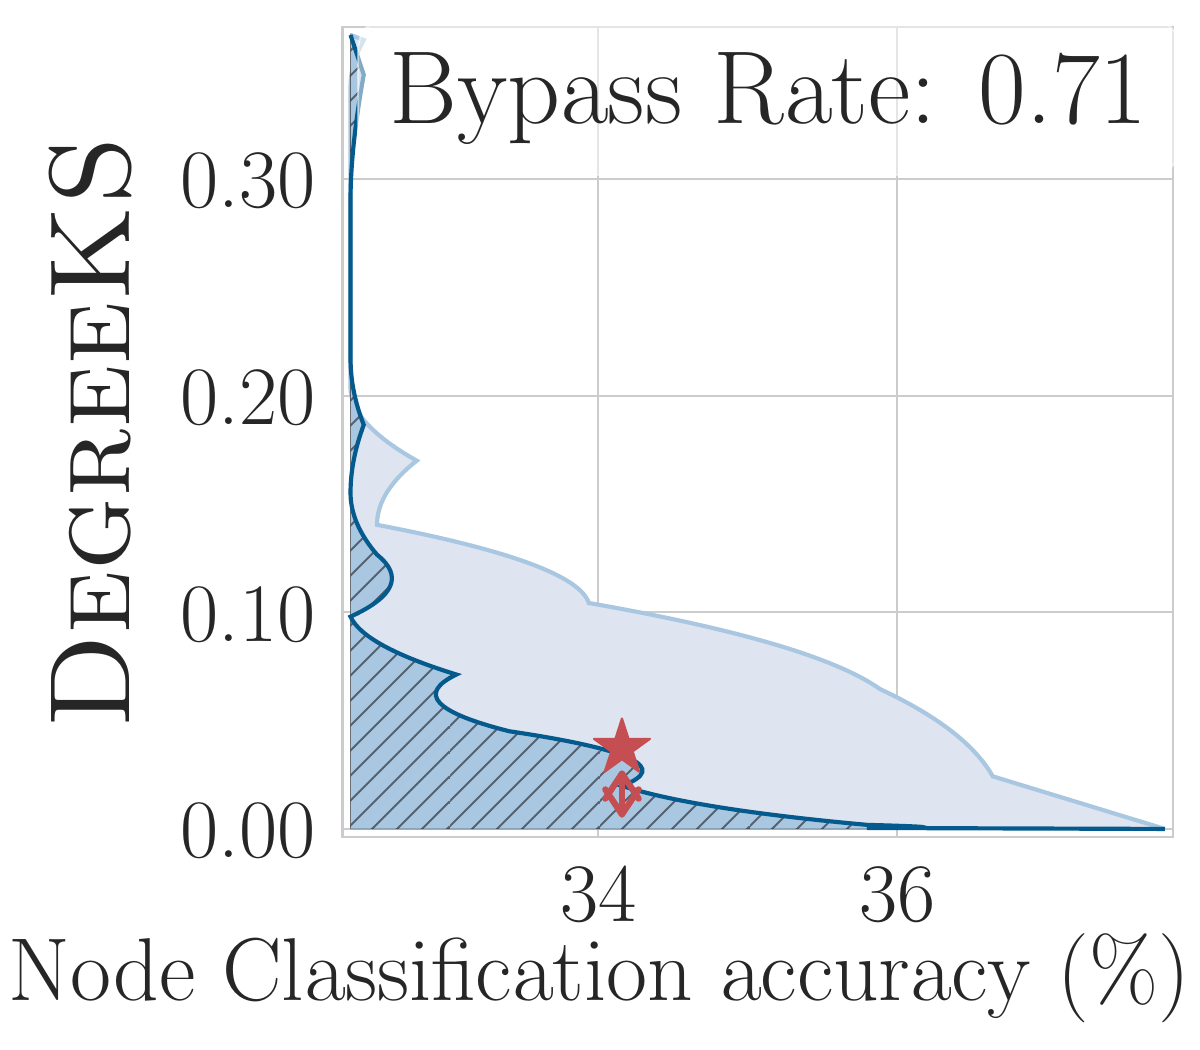} & 
        \includegraphics[width=\linewidth]{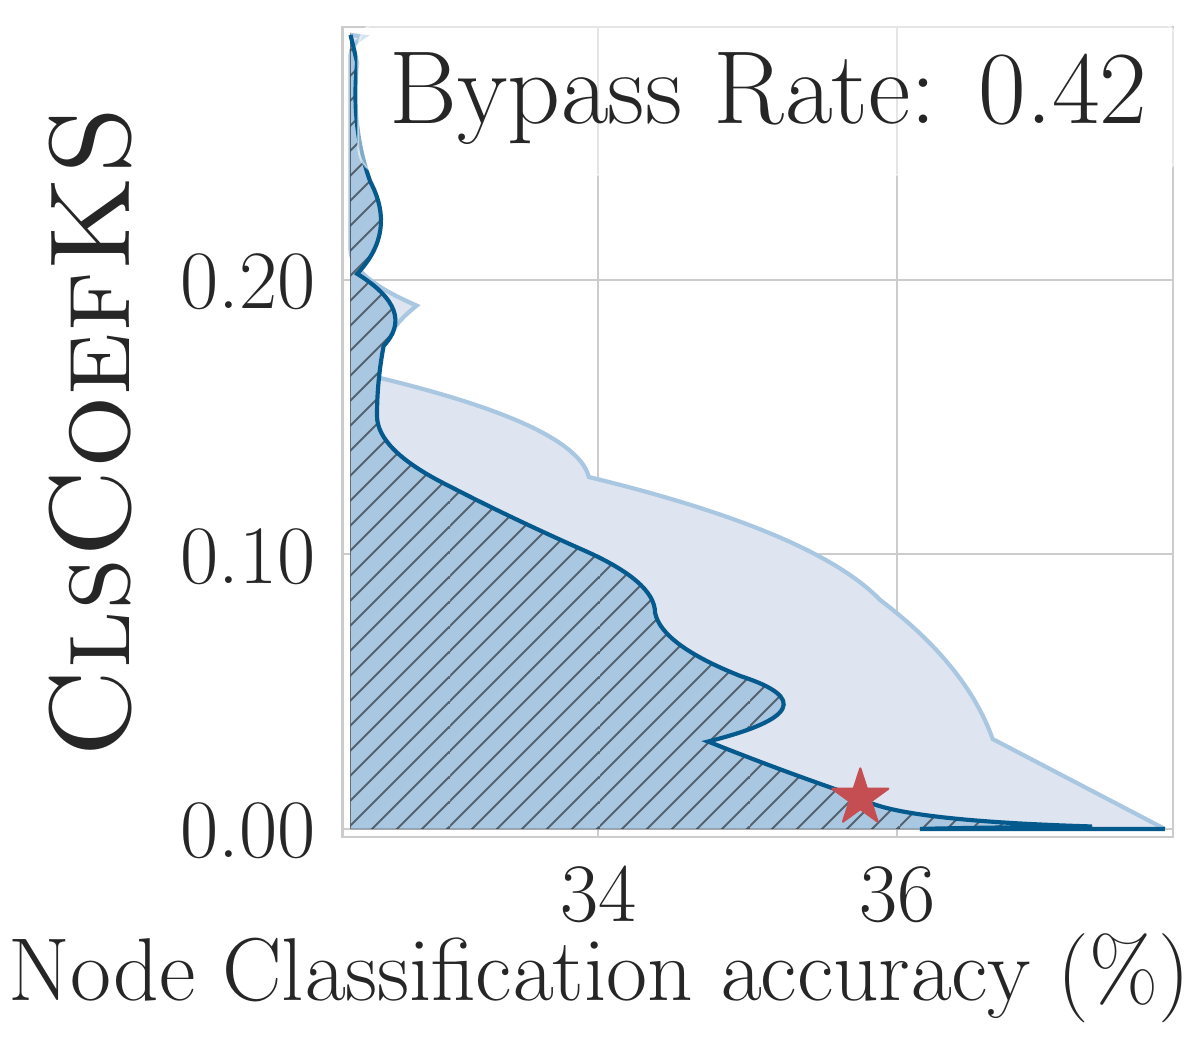} & 
        \includegraphics[width=\linewidth]{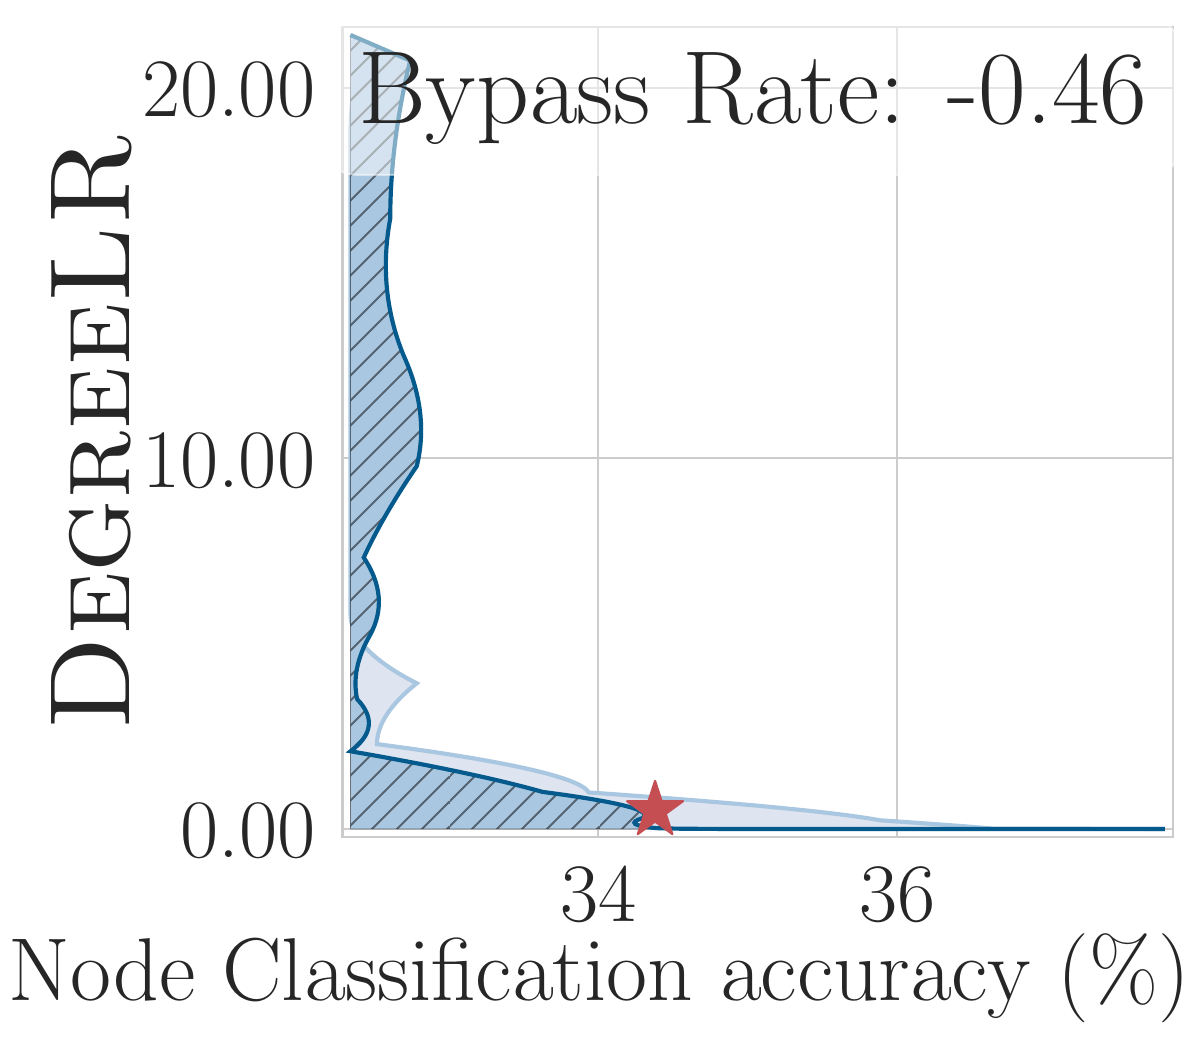} & 
        \includegraphics[width=\linewidth]{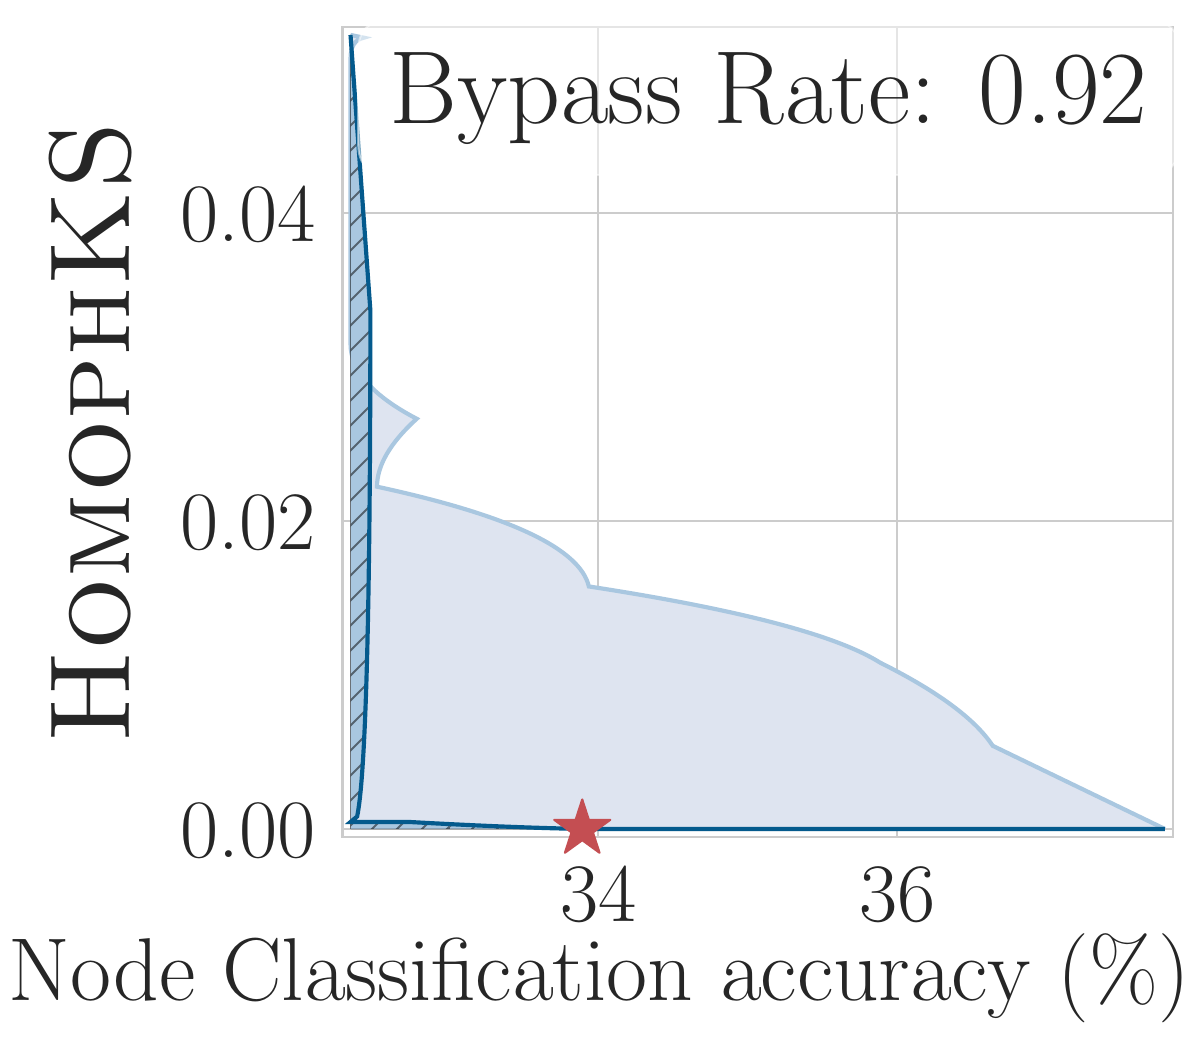} &
        \includegraphics[width=\linewidth]{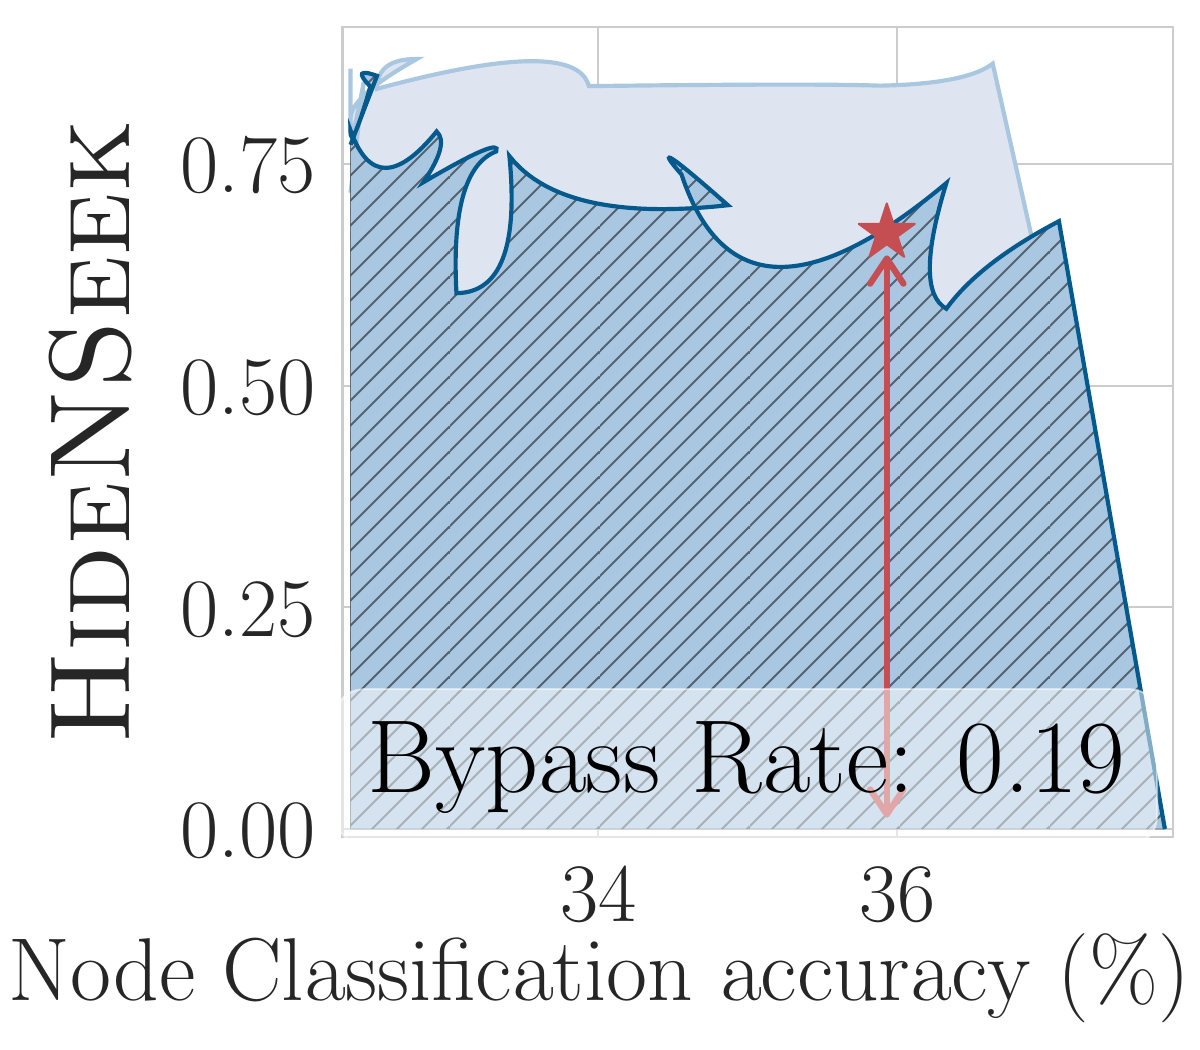} \\
        \hline
    \end{tabular}
    }
    \label{tab:exp:q2_metattack}
\end{table*}
